# Supplementary material for: Dynamic Heterogeneous Distribution Regression Panel Models, with an Application to Labor Income Processes
Source: arXiv:2202.04154 ancillary file (2026-07-03)
Supplement: Supplementary file 1 [file Supplement.pdf]

# SUPPLEMENT TO “DYNAMIC HETEROGENEOUS DISTRIBUTION REGRESSION PANEL MODELS, WITH AN APPLICATION TO LABOR INCOME PROCESSES”

IVÁN FERNÁNDEZ-VAL, WAYNE YUAN GAO, YUAN LIAO, AND FRANCIS VELLA

ABSTRACT. The supplement contains additional simulations, definitions of the analytical bias estimators, technical assumptions, and all proofs.

## CONTENTS

|                                                                                      |    |
|--------------------------------------------------------------------------------------|----|
| Appendix B. Additional Simulation Results                                            | 2  |
| B.1. Design 2: Calibrated Model                                                      | 2  |
| B.2. Dynamic probit model                                                            | 3  |
| Appendix C. Technical Details                                                        | 4  |
| C.1. Debiased estimators for $\beta_i(y)$                                            | 4  |
| C.2. The counterfactual distribution of stationary distribution                      | 6  |
| C.3. Definitions of leading terms in expansions                                      | 7  |
| C.4. Further technical conditions                                                    | 8  |
| Appendix D. Theories for the debiased estimators $\hat{\beta}_i$                     | 10 |
| D.1. Asymptotic expansion for $\hat{\beta}_i$                                        | 10 |
| D.2. Technical lemmas                                                                | 14 |
| Appendix E. Proof of Theorem 5.1                                                     | 16 |
| E.1. A high-level weak convergence result                                            | 16 |
| E.2. Proof of Theorem 5.1                                                            | 19 |
| Appendix F. Proof of Theorem 5.2                                                     | 26 |
| F.1. The functional $\vartheta^g(y) = \mathbb{E}_t f(\beta_i(y), \theta(y), D_{it})$ | 27 |
| F.2. Proof of Theorem 5.2                                                            | 32 |
| Appendix G. Proof of Theorem 5.3: the Counterfactual QE                              | 33 |
| Appendix H. Proof of Theorem 5.4: Bootstrap Validity                                 | 37 |
| H.1. Bootstrap weak convergence                                                      | 37 |
| H.2. Proof of Theorem 5.4 (i): coverage of $\theta(y)$                               | 41 |
| H.3. Proof of Theorem 5.4 (ii): coverage of cross-section distributions              | 45 |

---

*Date:* This draft: February 8, 2022.

|                                                    |    |
|----------------------------------------------------|----|
| H.4. Proof of Theorem 5.4 (iii): coverage of QE    | 46 |
| Appendix I. Proofs for the Stationary Distribution | 47 |
| I.1. The asymptotic distribution                   | 47 |
| References                                         | 55 |

## APPENDIX B. ADDITIONAL SIMULATION RESULTS

**B.1. Design 2: Calibrated Model.** Next, we simulate a dynamic distribution regression model from a heterogeneous-coefficient autoregressive model with calibrated parameters using the PSID data.

Specifically, using the empirical data, we first estimate the following model

$$Y_{i,t} = -\beta_{0i} - \beta_{1i}Y_{i,t-1} + \sigma\epsilon_{it}, \quad (\text{B.1})$$

for each in-sample individual  $i$  to calibrate  $\beta_{0i}, \beta_{1i}$  and  $\sigma$ , which we then use to calibrate the second-stage model parameters  $(\theta_{00}, \theta_{01}, \theta_{10}, \theta_{11})$  and  $\sigma_0, \sigma_1$  by running the regressions

$$\begin{aligned} \beta_{0,i} &= \theta_{00} + w'_{1i}\theta_{01} + \sigma_0\gamma_{0,i}, \\ \beta_{1,i} &= \theta_{10} + w'_{1i}\theta_{11} + \sigma_1\gamma_{1,i}. \end{aligned} \quad (\text{B.2})$$

where  $Y_{i,t}$  is the outcome variables (residual log income), and  $w_{1i}$  is the vector of individual characteristics consisting of the variables *edu*, *race*, *birth*, and *initialsalary*.

Letting  $x_{it} := (1, Y_{i,t-1})'$ ,  $w_i := (1, w'_{1i})'$  and assume  $\epsilon_{it} \sim \mathcal{N}(0, 1)$ , we may then rewrite (B.1) and (B.2) into the following heterogeneous dynamic distribution regression model

$$P(Y_{i,t} \leq y | x_{it}) = \Phi\left(\tilde{\beta}_{0,i}(y) + \tilde{\beta}_{1,i}(y)Y_{i,t-1}\right)$$

where

$$\begin{aligned} \tilde{\beta}_{0,i}(y) &:= \frac{y + \beta_{0,i}}{\sigma} = \tilde{\theta}_0(y)' w_i + \sigma_0\gamma_{0,i}, \\ \tilde{\beta}_{1,i}(y) &:= \frac{\beta_{1,i}}{\sigma} = \tilde{\theta}_1(y)' w_i + \sigma_1\gamma_{1,i}, \\ \tilde{\theta}_0(y) &:= \left(\frac{y + \theta_{00}}{\sigma}, \frac{\theta_{01}}{\sigma}\right)', \\ \tilde{\theta}_1(y) &:= \left(\frac{\theta_{10}}{\sigma}, \frac{\theta_{11}}{\sigma}\right)'. \end{aligned} \quad (\text{B.3})$$

TABLE B.1. QTE of Increasing  $edu$  by 1

| Quantiles  | Estimator MSE $\times 10^{-2}$ |       |       |       |       |
|------------|--------------------------------|-------|-------|-------|-------|
|            | 15%                            | 25%   | 50%   | 75%   | 85%   |
| No-debias  | 0.015                          | 0.015 | 0.022 | 0.019 | 0.015 |
| Analytical | 0.012                          | 0.07  | 0.016 | 0.016 | 0.015 |
| Jackknife  | 1.99                           | 1.54  | 1.48  | 1.76  | 2.03  |

We then simulate  $Y_{i,t}$  according to models (B.1) and (B.2) based on the calibrated values of  $\beta$ ,  $\sigma$ ,  $\sigma_0$  and  $\sigma_1$  and calculate the implied distribution regression parameters  $\tilde{\beta}_{0,i}(y)$ ,  $\tilde{\beta}_{1,i}(y)$ ,  $\tilde{\theta}_0(y)$  and  $\tilde{\theta}_1(y)$  based on (B.3), and apply the estimation methods we proposed in this paper to estimate the quantile treatment effects of a counterfactual increase of  $edu_i$  (education) by 1 year for every individual in the sample.

Table B.1 reports the results about the MSEs of our proposed estimators, one using analytical debiasing (“Analytical”) and one using jackknife debiasing (“Jackknife”), in comparison with the estimator without debiasing (“No-debias”). Here we note that, while the estimator with analytical debiasing performs well and generally better than the one with no debiasing, the jackknife debiased estimator suffers from notably larger MSEs. The main reason underlying the problem with jackknife debiasing here is a drastic worsening of the split-sample estimator on half of time periods, which seems to come from a reduction in the variations of the outcome variable. This suggests that the analytical debiasing be used when the number of time periods is relatively small.

**B.2. Dynamic probit model.** We also consider a dynamic probit model

$$\begin{aligned} P(y_{i,t+1}(y) = 1 | y_{i,t}(y), \beta_i(y)) &= \Phi(y_{i,t}(y)\beta_i(y) + 0.1) \\ \beta_i(y) &= \theta(y)w_{1,i} + 0.3w_{2,i} + \theta(y)\bar{\gamma}_i. \end{aligned}$$

The outcome variable depends on  $y \in (0, 1)$  through the coefficient  $\beta_i(y)$ . We independently simulate the relevant variables and the initial  $y_{i,0}$  as follows:

$$(w_{1,i}, w_{2,i}, \bar{\gamma}_i) \sim \text{Uniform}(-0.5, 0.5), \quad y_{i,0}(y) \sim \text{Bernoulli}(0.7).$$

As for the coefficient function, we take  $\theta(y) = 0.5/T^{2y^2}$  which is strictly decreasing and depends on  $T$ . Note that

$$\Sigma_{NT}(y) \approx \begin{cases} \frac{1}{NT}V_\psi(y), & y \rightarrow 1 \\ \frac{1}{N}3\text{Var}(\bar{\gamma}_i), & y \rightarrow 0 \end{cases}.$$

Hence the convergence rate of  $\Sigma_{NT}(y)$  varies as  $y$  approaches to either boundary of its support. Also note that  $|\beta_i(y)| < 0.65$  almost surely so  $Y_{it}(y)$  is stationary.

Table B.2 reports the coverage probabilities of the confidence band for  $\{\theta(y) : y \in M\}$ , where  $M = \{0, 0.2, \dots, 1\}$ . The three bootstrap based methods: proposed, no-debias and conservative bootstrap, perform overall satisfactorily, while the two plug-in methods are either very conservative or under-coveraging. In addition, Figure B.1 plots the true and estimated standard errors of  $\hat{\theta}(y)$ . As expected, the two plug-in standard errors are not uniformly good.

TABLE B.2. Coverage Probabilities of  $\{\theta(y) : y \in M\}$  in dynamic probit model

| $T$ | $N$ | Methods  |           |             |             |              |
|-----|-----|----------|-----------|-------------|-------------|--------------|
|     |     | Proposed | No-debias | Conser-boot | Plugin-over | Plugin-under |
| 200 | 300 | 0.947    | 0.945     | 0.950       | 0.996       | 0.894        |
|     | 400 | 0.961    | 0.956     | 0.954       | 0.995       | 0.910        |
| 250 | 300 | 0.945    | 0.940     | 0.943       | 0.997       | 0.886        |
|     | 400 | 0.951    | 0.948     | 0.949       | 0.997       | 0.909        |
| 300 | 300 | 0.950    | 0.951     | 0.959       | 0.996       | 0.894        |
|     | 400 | 0.953    | 0.947     | 0.953       | 0.996       | 0.886        |

FIGURE B.1.  $\text{Var}(\gamma_i(y))$  and estimated and true standard errors of  $\hat{\theta}(y)$  for  $y \in M$  in the dynamic probit model.  $N = 400, T = 300$ .

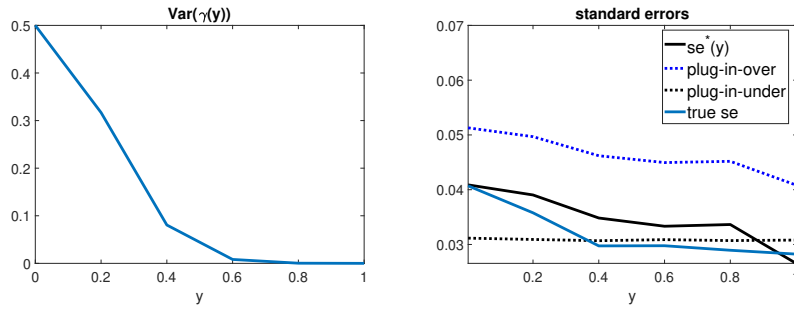

## APPENDIX C. TECHNICAL DETAILS

**C.1. Debiased estimators for  $\beta_i(y)$ .** First of all, recall that  $N_0(y)$  is the number of indexes  $i$  for which  $y < \underline{y}_i$ ,  $N_1(y)$  be the number of indexes  $i$  for which  $y \geq \bar{y}_i$ , and  $N_{01}(y) = N - N_0(y) - N_1(y)$ , that is the number of indexes  $i$  for which  $\tilde{\beta}_i(y)$  exists.

In addition, the imposed assumptions ensure that with probability approaching one, the following event holds:

For all  $y \in \mathcal{Y}$ , and all  $i = 1, \dots, N$ , we have  $\min_{t \leq T} y_{it} < y < \max_{t \leq T} y_{it}$ .

Under this event,  $N_0(y) = N_1(y) = 0$  and  $N_{01}(y) = N$  for all  $y \in \mathcal{Y}$ . So throughout the technical proofs, we condition on this event, which would not affect the asymptotic results.

C.1.1. *Analytical Debias.* The initial estimator can be expanded as

$$\tilde{\beta}_i(y) - \beta_i(y) = -\mathbb{A}_{1i}(y) \nabla Q_{y,i}(\beta_i(y)) - \frac{1}{T} B_{i,1T}(y) - \frac{1}{T} B_{i,2T}(y) + R_i(y)$$

where  $\mathbb{A}_{1i} = [\nabla^2 \mathbb{E} Q_{y,i}(\beta_i(y))]^{-1}$ ,  $\nabla Q_{y,i}(\beta_i(y)) = -\frac{1}{T} \sum_{t=1}^T \psi_{it}(y)$  and  $R_i(y)$  is the higher order term. To describe the first-order biases  $B_{i,1T}(y)$  and  $B_{i,2T}(y)$ , write  $A_{1i} = [\nabla^2 Q_{y,i}(\beta_i(y))]^{-1}$ ,  $A_{2i} = \nabla^3 Q_{y,i}(\beta_i(y))$ , and  $\mathbb{A}_{2i} = \nabla^3 \mathbb{E} Q_{y,i}(\beta_i(y))$ . Then

$$\mathbb{A}_{1i} \sqrt{T} \nabla Q_{y,i}(\beta_i(y)) = \frac{1}{\sqrt{T}} \sum_t \mathbb{A}_{1i} \psi_{it}(y), \quad \sqrt{T} A_{1i}^{-1} = \frac{1}{\sqrt{T}} \sum_t \varpi_{it}^2(y).$$

Here  $\varpi_{it}^2(y)$  is  $\dim(\beta_i) \times \dim(\beta_i)$ . Let  $\varpi_{it,k}^2(y)$  be its  $k$ th column and

$$V_{i,k}(y) := \text{Var} \left[ \frac{1}{\sqrt{T}} \sum_t \ell_{it} \right] = \begin{pmatrix} M_1(y) & M_{2,k}(y)' \\ M_{2,k}(y) & M_{3k}(y) \end{pmatrix}, \quad \ell_{it} := \begin{pmatrix} \mathbb{A}_{1i} \psi_{it}(y) \\ \varpi_{it,k}^2(y) \end{pmatrix}.$$

Then

$$\begin{aligned} B_{i,1T}(y) &= \frac{1}{2} \mathbb{A}_{1i} \mathbb{A}_{2i} \text{vec}(M_1(y)) \\ B_{i,2T}(y) &= -\mathbb{A}_{1i} \begin{pmatrix} \text{tr}(M_{2,1}(y)) \\ \vdots \\ \text{tr}(M_{2,\dim(\beta_i)}(y)) \end{pmatrix}. \end{aligned} \tag{C.1}$$

Hence we can estimate  $B_{i,1T}(y)$  and  $B_{i,2T}(y)$  by replacing  $V_{i,k}(y)$  by its estimator  $\hat{V}_{i,k}(y)$ ; the latter can be obtained by the Newey-West truncation.

$$\hat{V}_{i,k}(y) = \frac{1}{T} \sum_{t=1}^T \hat{\ell}_{it} \hat{\ell}_{it}' + \frac{1}{T} \sum_{h=1}^L \sum_{t>h} [\hat{\ell}_{it} \hat{\ell}_{i(t-h)}' + \hat{\ell}_{i(t-h)} \hat{\ell}_{it}'].$$

Let  $\hat{B}_{i,1T} = \frac{1}{2} \hat{\mathbb{A}}_{1i} \hat{\mathbb{A}}_{2i} \text{vec}(\hat{M}_1(y))$  and  $\hat{B}_{i,2T}$  be defined as  $B_{i,2T}(y)$  with  $\mathbb{A}_{1i}$  and  $M_{2,k}(y)$  replaced with their estimates.

C.1.2. *Jackknife Debias.* Alternative to the analytical debias, we can also employ the sample-splitting Jackknife debias to remove the higher order bias, which was used for instance, by Dhaene and Jochmans (2015); Okui and Yanagi (2019).

Randomly split  $\{1, \dots, T\} = \mathcal{I} \cup \mathcal{I}^c$ , so that  $|\mathcal{I}| = T/2$ . Let  $\tilde{\beta}_{i,\mathcal{I}}(y)$  be the same estimated  $\beta_i(y)$ , but using data only for  $t \in \mathcal{I}$ . Similarly, let  $\tilde{\beta}_{i,\mathcal{I}^c}(y)$  be the estimated  $\beta_i(y)$ , but using data only for  $t \in \mathcal{I}^c$ . Let

$$\bar{\beta}_i(y) = \frac{1}{2}[\tilde{\beta}_{i,\mathcal{I}}(y) + \tilde{\beta}_{i,\mathcal{I}^c}(y)].$$

Then the Jackknife debiased estimator is defined as:

$$\hat{\beta}_i(y) = 2\tilde{\beta}_i(y) - \bar{\beta}_i(y).$$

## C.2. The counterfactual distribution of stationary distribution.

C.2.1. *The model.* We recall that the stationary distribution is defined as  $F_\infty(y) = \mathbb{E}[F_{i,\infty}(y)]$ , where  $F_{i,\infty}(y) = \sum_{k: y_i^k \leq y} \pi_{ik}$ ; the ergodic probabilities  $\pi_i = (\pi_{i1}, \dots, \pi_{iK})$  are

$$\pi_i = (\mathbf{A}_i' \mathbf{A}_i)^{-1} \mathbf{A}_i' \mathbf{e}_{K+1}, \quad \mathbf{A}_i = \begin{pmatrix} \mathbf{I}_K - \mathbf{P}_i \\ \mathbf{1}' \end{pmatrix}$$

and  $\mathbf{e}_{K+1}$  is the  $(K+1)$ th column of  $\mathbf{I}_{K+1}$ . Also,  $\mathbf{P}_i$  is a  $K \times K$  matrix with element  $P_{i,jk} = \Pr(y_{it} = y_i^j \mid y_{i(t-1)} = y_i^k, \mathcal{F}_{it}) = \Lambda(-\mathbf{x}_i^{k'} \beta_i(y_i^j)) - 1(j > 1) \Lambda(-\mathbf{x}_i^{k'} \beta_i(y_i^{j-1}))$ .

Hence we can write

$$F_\infty(y) = \mathbb{E} f_i(\beta_i, y)$$

where  $\beta_i = \text{vec}(\beta_i(y_i^1), \dots, \beta_i(y_i^K))$  and

$$f_i(\beta_i, y) = \sum_{k=1}^K 1\{y_i^k \leq y\} \mathbf{e}_k' \mathbf{G}_i(\beta_i), \quad \mathbf{G}_i(\beta_i) = (\mathbf{A}_i' \mathbf{A}_i)^{-1} \mathbf{A}_i' \mathbf{e}_{K+1}.$$

The counterfactual stationary distribution is defined as

$$G_\infty(y) = \mathbb{E} f_i(\beta_i, \theta_i, y), \quad \theta_i = \text{vec}(\theta(y_i^1), \dots, \theta(y_i^K)),$$

where

$$f_i(\beta_i, \theta_i, y) = \sum_{k=1}^K 1\{y_i^k \leq y\} \mathbf{e}_k' (\mathbf{A}_i(\beta_i, \theta_i)' \mathbf{A}_i(\beta_i, \theta_i))^{-1} \mathbf{A}_i(\beta_i, \theta_i)' \mathbf{e}_{K+1}$$

and  $\mathbf{A}_i(\beta_i, \theta_i)$  is defined as  $\mathbf{A}_i$  but with  $\beta_i$  replaced by

$$\beta_i^g = \text{vec}(\beta_i(y_i^k) + \theta(y_i^k)(g(z_i) - z_i) : k = 1, \dots, K).$$

C.2.2. *The Estimators of stationary distributions.* Under the condition that  $\Lambda(-\mathbf{x}_i^{k'}\beta_i(y_i^j)) = 1$  for  $j = K$ , we have

$$\widehat{F}_\infty(y) = \frac{1}{N} \sum_{i=1}^N f_i(\widehat{\beta}_i, y) - \frac{1}{T} \frac{1}{N} \sum_{i=1}^N \widehat{B}_{\pi_i}$$

where  $\widehat{B}_{\pi_i} = \frac{1}{2} \text{tr} \left[ \partial_{\beta}^2 f_i(\widehat{\beta}_i, y) \frac{1}{T} \sum_t \widehat{\mathbf{Z}}_{it} \widehat{\mathbf{Z}}_{it}' \right]$  and

$$\widehat{\mathbf{Z}}_{it} = \text{vec}(\widehat{\mathbb{A}}_{1i}(y_i^1) \widehat{\psi}_{it}(y_i^1), \dots, \widehat{\mathbb{A}}_{1i}(y_i^K) \widehat{\psi}_{it}(y_i^K)).$$

Similarly, we estimate  $G_\infty$  by the following bias-corrected estimator:

$$\widehat{G}_\infty(y) = \frac{1}{N} \sum_i f_i(\widehat{\beta}_i, \widehat{\theta}_i, y) - \frac{1}{2NT} \sum_i \text{tr} \left[ \partial_{\beta}^2 f_i(\widehat{\beta}_i, \widehat{\theta}_i, y) \frac{1}{T} \sum_i \widehat{\mathbf{Z}}_{it} \widehat{\mathbf{Z}}_{it}' \right].$$

C.3. **Definitions of leading terms in expansions.** We shall show that

$$\begin{aligned} \widehat{F}_t(y) - F_t(y) &= \frac{1}{N} \sum_{i=1}^N \left[ \frac{1}{\sqrt{T}} d_{\psi,i}^0(y) + d_{\gamma,i}^0(y) \right] + o_P(\zeta_{NT}(y)) \\ \widehat{G}_t(y) - G_t(y) &= \frac{1}{N} \sum_{i=1}^N \left[ \frac{1}{\sqrt{T}} d_{\psi,i}^{II}(y) + d_{\gamma,i}^{II}(y) \right] + o_P(\zeta_{NT}(y)) \\ \widehat{F}_\infty(y) - F_\infty(y) &= \frac{1}{N} \sum_{i=1}^N \left[ \frac{1}{\sqrt{T}} d_{\psi,i}^\infty(y) + d_{\gamma,i}^\infty(y) \right] + o_P(\zeta_{NT}(y)) \\ \widehat{G}_\infty(y) - G_\infty(y) &= \frac{1}{N} \sum_{i=1}^N \left[ \frac{1}{\sqrt{T}} d_{\psi,i}^{\infty,II}(y) + d_{\gamma,i}^{\infty,II}(y) \right] + o_P(\zeta_{NT}(y)) \\ \widehat{\mathbf{Q}}\mathbf{E}_t(\tau) - \mathbf{Q}\mathbf{E}_t(\tau) &= \frac{1}{N} \sum_{i=1}^N \left[ \frac{1}{\sqrt{T}} p_{\psi,i}^{II}(\tau) + p_{\gamma,i}^{II}(\tau) \right] + o_P(\bar{\zeta}_{NT}(\tau)) \\ \widehat{\mathbf{Q}}\mathbf{E}_\infty(\tau) - \mathbf{Q}\mathbf{E}_\infty(\tau) &= \frac{1}{N} \sum_{i=1}^N \left[ \frac{1}{\sqrt{T}} p_{\psi,i}^{\infty,II}(\tau) + p_{\gamma,i}^{\infty,II}(\tau) \right] + o_P(\bar{\zeta}_{NT}(\tau)). \end{aligned}$$

The involved terms are defined as follows. We introduce some notation. Let

$$\mathbf{Z}_{jt,i} = \text{vec}(\mathbb{A}_{1j}(y_i^1) \psi_{jt}(y_i^1), \dots, \mathbb{A}_{1j}(y_i^K) \psi_{jt}(y_i^K)). \quad \mathbf{Z}_{it} := \mathbf{Z}_{it,i}.$$

In addition,  $q_{\infty,0}(\tau) = \phi(F_\infty, \tau)$ , and  $q_{\infty,II}(\tau) = \phi(G_\infty, \tau)$ , and  $\boldsymbol{\gamma}_{j,i} = \text{vec}(\gamma_j(y_i^1), \dots, \gamma_j(y_i^K))$ .

$$\begin{aligned} d_{\psi,i}^0(y) &:= \frac{1}{\sqrt{T}} \sum_{t=1}^T \dot{\Lambda}(-\mathbf{x}_{it}' \boldsymbol{\beta}_i(y)) \mathbf{x}_{it}' \mathbb{A}_{1i}(y) \psi_{it}(y), \\ d_{\psi,i}^{II}(y) &= \frac{1}{\sqrt{T}} \sum_{t=1}^T [\mathbf{w}_i' S_{wz} \bar{G}(y) + \dot{\Lambda}(-\mathbf{x}_{it}' \boldsymbol{\beta}_i^g(y)) \mathbf{x}_{it}'] \mathbb{A}_{1i}(y) \psi_{it}(y) \end{aligned}$$

$$\begin{aligned}
d_{\gamma,i}^0(y) &= \Lambda(-\mathbf{x}'_{it}\beta_i(y)) - \mathbb{E}_t \Lambda(-\mathbf{x}'_{it}\beta_i(y)) \\
d_{\gamma,i}^{II}(y) &= \mathbf{w}'_i S_{wz} \bar{G}(y) \gamma_i(y) + \Lambda(-\mathbf{x}'_{it}\beta_i^g(y)) - \mathbb{E}_t \Lambda(-\mathbf{x}'_{it}\beta_i^g(y)), \\
d_{\psi,i}^\infty(y) &:= -\partial_{\beta} f_i(\beta_i, y)' \frac{1}{\sqrt{T}} \sum_{t=1}^T \mathbf{Z}_{it}, \\
d_{\gamma,i}^\infty(y) &:= f(\beta_i, y) - \mathbb{E} f(\beta_i, y) \\
d_{\psi,j}^{\infty,II}(y) &:= -\frac{1}{\sqrt{T}} \sum_t \partial_{\beta} f_j(y)' \mathbf{Z}_{jt} + \frac{1}{\sqrt{T}} \sum_t H_{jt}(y) \mathbf{w}'_j S_{wz}, \quad H_{jt}(y) := \frac{1}{N} \sum_i \partial_{\theta} f_i(y)' \mathbf{Z}_{jt,i} \\
d_{\gamma,j}^{\infty,II}(y) &:= \frac{1}{N} \sum_i \partial_{\theta} f_i(\beta_i, \theta_i, y)' \gamma_{j,i} \mathbf{w}'_j S_{wz} + \frac{1}{N} \sum_i f(\beta_i, \theta_i, y) - \mathbb{E} f(\beta_i, \theta_i, y), \\
p_{\psi,i}^{II}(\tau) &= \kappa^{II}(\tau) d_{\psi,i}^{II}(\phi(G_t, \tau)) + \kappa^0(\tau) d_{\psi,i}^0(\phi(F_t, \tau)) \\
p_{\gamma,i}^{II}(\tau) &= \kappa^{II}(\tau) d_{\gamma,i}^{II}(\phi(G_t, \tau)) + \kappa^0(\tau) d_{\gamma,i}^0(\phi(F_t, \tau)) \\
p_{\psi,i}^{\infty,II}(\tau) &= \kappa^{\infty,II}(\tau) d_{\psi,i}^{\infty,II}(\phi(G_\infty, \tau)) + \kappa^\infty(\tau) d_{\psi,i}^\infty(\phi(F_\infty, \tau)) \\
p_{\gamma,i}^{\infty,II}(\tau) &= \kappa^{\infty,II}(\tau) d_{\gamma,i}^{\infty,II}(\phi(G_\infty, \tau)) + \kappa^\infty(\tau) d_{\gamma,i}^\infty(\phi(F_\infty, \tau)).
\end{aligned}$$

where  $\bar{G}(y) = -\mathbb{E}_t \dot{\Lambda}(-\mathbf{x}'_{it}\beta_i^g(y)) \text{vec}(\mathbf{x}_{it}(g(\mathbf{z}_i) - \mathbf{z}_i)')$ , and

$$\begin{aligned}
\kappa^{II}(\tau) &= \frac{-1}{\dot{G}_t(\phi(G_t, \tau))}, \quad \kappa^0(\tau) = \frac{1}{\dot{F}_t(\phi(F_t, \tau))} \\
\kappa^{\infty,II}(\tau) &= \frac{-1}{\dot{G}_\infty(\phi(G_\infty, \tau))}, \quad \kappa^\infty(\tau) = \frac{1}{\dot{F}_\infty(\phi(F_\infty, \tau))}.
\end{aligned} \tag{C.2}$$

**C.4. Further technical conditions.** We additional assume the following assumptions.

**Assumption C.1** (For Jackknife). *(i) For each  $i$ ,  $\{(Y_{it}, \mathbf{x}_{it}) : t = 1, \dots, T\}$  is serially strictly stationary.*

*(ii) Long-run covariance: write*

$$\mu_{i,T}(y) := \frac{1}{\sqrt{T}} \sum_{t=1}^T (\psi_{it}(y)', \text{vec}(\varpi_{it}^2(y)))'.$$

*Then almost surely,  $\lim_{T \rightarrow \infty} \text{Cov}(\mu_{i,T}(y))$  exists and*

$$\max_i \sup_y \|\text{Cov}(\mu_{i,T}(y)) - \lim_{T \rightarrow \infty} \text{Cov}(\mu_{i,T}(y))\| = O(T^{-1/2}).$$

For the estimation of QE, we additionally require the following.

**Assumption C.2** (For QE). *There is  $C > 0$ , so that*

$$\begin{aligned}
\text{Var}_t(d_{\gamma,i}^0(q_0(\tau))) + \text{Var}_t(d_{\gamma,i}^I(q_I(\tau))) &\leq C \text{Var}_t(\kappa^0(\tau) d_{\gamma,i}^0(q_0(\tau)) + \kappa^I(\tau) d_{\gamma,i}^I(q_I(\tau))) \\
\text{Var}_t(d_{\gamma,i}^0(q_0(\tau))) + \text{Var}_t(d_{\gamma,i}^{II}(q_{II}(\tau))) &\leq C \text{Var}_t(\kappa^0(\tau) d_{\gamma,i}^0(q_0(\tau)) + \kappa^{II}(\tau) d_{\gamma,i}^{II}(q_{II}(\tau))).
\end{aligned}$$

**Assumption C.3** (For stationary distributions). (i) For  $d = 1, 2$ ,  $\max_i \mathbb{E} \sup_y \|\partial_\beta^d f_i(\beta_i, y)\|^2 < C$ . Also

$$\max_i \mathbb{E} \sup_y \|\partial_\beta^d f_i(\beta_i, \theta_i, y)\|^2 < C \text{ and } \max_i \mathbb{E} \sup_y \|\partial_\theta^d f_i(\beta_i, \theta_i, y)\|^4 < C.$$

(ii) For every  $y_1, y_2$ , for  $d = 1, 2$ ,

$$\mathbb{E} \sup_{|y_1 - y_2| \leq \epsilon} \|\partial_\beta^d f_i(\beta_i, y_1) - \partial_\beta^d f_i(\beta_i, y_2)\|^4 \leq C\epsilon^4$$

$$\mathbb{E} \sup_{|y_1 - y_2| \leq \epsilon} \|\partial_\beta^d f_i(\beta_i, \theta_i, y_1) - \partial_\beta^d f_i(\beta_i, \theta_i, y_2)\|^4 \leq C\epsilon^4$$

$$\mathbb{E} \sup_{|y_1 - y_2| \leq \epsilon} \|\partial_\theta^d f_i(\beta_i, \theta_i, y_1) - \partial_\theta^d f_i(\beta_i, \theta_i, y_2)\|^4 \leq C\epsilon^4$$

In addition, for  $f_i \in \{f_i(\beta_i, y), f_i(\beta_i, \theta_i, y)\}$ .

$$\begin{aligned} \mathbb{E} \sup_{\rho(y_1, y_2) < \delta} \frac{|f_i(y_1) - \mathbb{E} f_i(y_1) - (f_i(y_2) - \mathbb{E} f_i(y_2))|^2}{\sqrt{\text{Var}(f_i(y_1))\text{Var}(f_i(y_2))}} &\leq \delta^2 \\ \sup_{\rho(y_1, y_2) < \delta} \frac{|\text{Var}(f_i(y_1)) - \text{Var}(f_i(y_2))|^2}{\text{Var}(f_i(y_1))\text{Var}(f_i(y_2))} &\leq \delta^2 \\ \mathbb{E} \sup_{\rho(y_1, y_2) < \delta} \frac{\|\partial_\theta f_i(\beta_i, \theta_i, y_1) - \partial_\theta f_i(\beta_i, \theta_i, y_2)\|^2 \|\gamma_{j,i} \mathbf{w}'_j\|^2}{\sqrt{\bar{V}_\gamma(y_1)\bar{V}_\gamma(y_2)}} &\leq \delta^2 \\ \sup_{\rho(y_1, y_2) < \delta} \frac{|\bar{V}_\gamma(y_1) - \bar{V}_\gamma(y_2)|^2}{\bar{V}_\gamma(y_1)\bar{V}_\gamma(y_2)} &\leq \delta^2 \end{aligned}$$

(iii)  $\|\partial_\beta^2 f_i(b_1, y) - \partial_\beta^2 f_i(b_2, y)\| \leq C_i(y)\|b_1 - b_2\|$  and  $\|\partial_\beta^2 f_i(b_1, \theta_i, y) - \partial_\beta^2 f_i(b_2, \theta_i, y)\| \leq C_i(y)\|b_1 - b_2\|$  where  $\sup_y \frac{1}{N} \sum_i C_i(y)^4 = O_P(1)$ .

(iv)  $\mathbb{E} \sup_y \|\frac{1}{\sqrt{T}} \sum_{t=1}^T \partial_\beta f_i(\beta_i, y)' \mathbf{Z}_{it}\|^{2+a} \leq C$  for some  $a \geq 2$ . In addition,

$$\mathbb{E} \sup_y \left\| \frac{1}{\sqrt{T}} \sum_{t=1}^T \partial_\beta f_i(\beta_i, \theta_i, y)' \mathbf{Z}_{it} \right\|^{2+a} + \mathbb{E} \sup_y \left\| \frac{1}{\sqrt{T}} \sum_{t=1}^T H_{it}(y) \mathbf{w}_i \right\|^{2+a} \leq C.$$

(v)  $\mathbb{E} \sup_y [\mathbb{Z}_t(g_i(y))]^{2a} < C$ , for all

$$g_i(y) \in \{f(\beta_i, y), \partial_\theta f_i(\beta_i, \theta_i, y)' \gamma_{j,i} \mathbf{w}'_j S_{wz} + f_i(\beta_i, \theta_i, y)\}$$

(vi)  $\mathbb{E}[\|\frac{1}{\sqrt{T}} \sum_{t=1}^T \mathbf{Z}_{it}\|^4 | \beta_i] < C$  and  $\frac{1}{N} \sum_i \mathbb{E} \|\mathbf{w}'_j S_{wz}\|^4 \|\frac{1}{\sqrt{T}} \sum_t \mathbf{Z}_{jt,i}\|^4 < C$ .

(vii) Let  $V_{k_1, k_2}$  denote the  $(k_1, k_2)$  th block of  $\text{Var}(\frac{1}{\sqrt{T}} \sum_t \bar{\mathbf{Z}}_{jt} | \beta, \mathbf{w}_j)$ , which is a matrix collecting pairwise conditional covariances between elements of  $\mathbf{Z}_{jt, k_1}$  and  $\mathbf{Z}_{jt, k_2}$ .

We have  $\max_{k_1, k_2 \leq N} \|V_{k_1, k_2}\| \leq C$ .

(viii)  $\text{Var}_t(d_{\gamma,i}^\infty) + \text{Var}_t(d_{\gamma,i}^{\infty, II}) = O(\text{Var}(p_{\gamma,i}^{\infty, II}))$ .

APPENDIX D. THEORIES FOR THE DEBIASED ESTIMATORS  $\widehat{\beta}_i$ 

Using the true value  $\beta_i := \beta_i(y)$  (we drop  $y$  for notational simplicity), define

$$\begin{aligned} R_{i,4} &= \frac{1}{2} \mathbb{A}_{1i} \mathbb{A}_{2i} \mathbb{E}[(\mathbb{A}_{1i} \nabla Q_i(\beta_i)) \otimes (\mathbb{A}_{1i} \nabla Q_i(\beta_i))] - \frac{1}{2} \mathbb{A}_{1i} \mathbb{A}_{2i} [(\mathbb{A}_{1i} \nabla Q_i(\beta_i)) \otimes (\mathbb{A}_{1i} \nabla Q_i(\beta_i))] \\ R_{i,5} &= \mathbb{A}_{1i} [(A_{1i}^{-1} - \mathbb{A}_{1i}^{-1}) \mathbb{A}_{1i} \nabla Q_i(\beta_i) - \mathbb{E}((A_{1i}^{-1} - \mathbb{A}_{1i}^{-1}) \mathbb{A}_{1i} \nabla Q_i(\beta_i))] \\ B_{i,1T} &= \frac{1}{2} \mathbb{A}_{1i} \mathbb{A}_{2i} \mathbb{E}[(\mathbb{A}_{1i} \sqrt{T} \nabla Q_i(\beta_i)) \otimes (\mathbb{A}_{1i} \sqrt{T} \nabla Q_i(\beta_i))] \\ B_{i,2T} &= -\mathbb{A}_{1i} \mathbb{E}[\sqrt{T} (A_{1i}^{-1} - \mathbb{A}_{1i}^{-1}) \mathbb{A}_{1i} \sqrt{T} \nabla Q_i(\beta_i)]. \end{aligned}$$

Standard first-order Taylor expansion gives

$$\widetilde{\beta}_i - \beta_i = -\nabla^2 Q_i(\beta_i)^{-1} \nabla Q_i(\beta_i) + \Delta_i \quad (\text{D.1})$$

where for some  $\beta_i^*$  between  $\widetilde{\beta}_i$  and  $\beta_i$ ,

$$\Delta_i = -\nabla^2 Q_i(\beta_i)^{-1} [\nabla^2 Q_i(\beta_i^*) - \nabla^2 Q_i(\beta_i)] (\widetilde{\beta}_i - \beta_i).$$

Let  $A_{1i} = [\nabla^2 Q_i(\beta_i)]^{-1}$ ,  $A_{2i} = \nabla^3 Q_i(\beta_i)$ ,  $\mathbb{A}_{1i} = [\nabla^2 \mathbb{E} Q_i(\beta_i)]^{-1}$ ,  $\mathbb{A}_{2i} = \nabla^3 \mathbb{E} Q_i(\beta_i)$ .

**D.1. Asymptotic expansion for  $\widehat{\beta}_i$ .** Recall that the jackknife debiased estimator is

$$\widehat{\beta}_i := \widetilde{\beta}_i - (\bar{\beta}_i - \widetilde{\beta}_i)$$

and the analytical debiased estimator is given by

$$\widehat{\beta}_i = \widetilde{\beta}_i + \frac{1}{T} [\widehat{B}_{i,1T} + \widehat{B}_{i,2T}].$$

**Lemma D.1** (Jackknife debias). *Additionally assume Assumption C.1. Let  $R_{i,d,\mathcal{I}}$  be similarly defined using data in  $\mathcal{I}$ , and  $\bar{R}_{i,d} = \frac{1}{2} [R_{i,d,\mathcal{I}} + R_{i,d,\mathcal{I}^c}]$ . Then the jackknife estimator satisfies: for some  $R_{i,9}$ , (we drop  $y$  for notational simplicity)*

$$\widehat{\beta}_i - \beta_i = -\mathbb{A}_{1i} \frac{1}{T} \sum_t \psi_{it}(y) + R_{i,9} + 2R_{i,4} + 2R_{i,5} - \bar{R}_{i,4} - \bar{R}_{i,5}$$

where  $\sup_y \frac{1}{N} \sum_i \|R_{i9}\|^2 = O_P(T^{-3})$  and  $\frac{1}{T} \sum_t \psi_{it}(y) = \nabla Q_i(\beta_i)$ .

*Proof.* By Lemma D.3, for  $\sup_y \frac{1}{N} \sum_i \|\Delta_i\|^2 = O_P(T^{-3})$ ,

$$\begin{aligned} \widetilde{\beta}_i - \beta_i &= -\mathbb{A}_{1i} \nabla Q_i(\beta_i) - \frac{1}{T} B_{i,1T} - \frac{1}{T} B_{i,2T} + R_{i,4} + R_{i,5} + \Delta_i \\ &= -\mathbb{A}_{1i} \nabla Q_i(\beta_i) - \frac{1}{T} B_i + R_{i,4} + R_{i,5} + \Delta_i + R_{i,7} \end{aligned}$$

where

$$B_i = \lim_{T \rightarrow \infty} B_{i,1T} + \lim_{T \rightarrow \infty} B_{i,2T}$$

$$R_{i,7} = \frac{1}{T} \left( \lim_{T \rightarrow \infty} B_{i,1T} + \lim_{T \rightarrow \infty} B_{i,2T} - B_{i,1T} - B_{i,2T} \right).$$

Note that the existence of  $\lim_{T \rightarrow \infty} B_{i,1T} + \lim_{T \rightarrow \infty} B_{i,2T}$  follows from Assumption 5.2 because  $B_{i,1T} + B_{i,2T}$  is a function of  $\text{Cov}(\mu_{i,T}(y)|\mathbf{w}_i)$  and  $\mathbb{A}_{1i}$ ;  $\mathbb{A}_{1i}$  does not depend on  $T$  due to the serial stationarity. We introduce  $B_i = \lim_{T \rightarrow \infty} B_{i,1T} + \lim_{T \rightarrow \infty} B_{i,2T}$  in the above expansion so that the higher-order bias  $-\frac{1}{T}B_i$  becomes independent of  $T$ ; in contrast  $B_{i,1T} + B_{i,2T}$  may depend on  $T$  due to the weak serial dependence. The fact that  $B_i$  is independent of  $T$  is required to apply the jackknife debias device, as we show below. By Assumption 5.2

$$\frac{1}{N} \sum_i \|R_{i,7}\|^2 \leq O(T^{-3}).$$

Similar expansion holds for  $\tilde{\beta}_{i,\mathcal{I}}$  and  $\tilde{\beta}_{i,\mathcal{I}^c}$ , whose sample size is  $T/2$ . For instance,

$$\tilde{\beta}_{i,\mathcal{I}} - \beta_i = -\mathbb{A}_{1i} \nabla Q_{i,\mathcal{I}}(\beta_i) - \frac{1}{T/2} B_i + R_{i,4\mathcal{I}} + R_{i,5\mathcal{I}} + \Delta_{i\mathcal{I}} + R_{i,7\mathcal{I}}.$$

Let  $\bar{\Delta}_i = \frac{1}{2}[\Delta_{i,\mathcal{I}} + \Delta_{i,\mathcal{I}^c}]$ . Therefore, with  $\bar{\beta}_i = \frac{1}{2}[\tilde{\beta}_{i,\mathcal{I}} + \tilde{\beta}_{i,\mathcal{I}^c}]$ :

$$\begin{aligned} \bar{\beta}_i - \beta_i &= -\mathbb{A}_{1i} \frac{1}{2} [\nabla Q_{i,\mathcal{I}}(\beta_i) + \nabla Q_{i,\mathcal{I}^c}(\beta_i)] - \frac{2}{T} B_i + \bar{R}_{i,4} + \bar{R}_{i,5} + \bar{R}_{i,7} + \bar{\Delta}_i \\ &= -\mathbb{A}_{1i} \nabla Q_i(\beta_i) - \frac{2}{T} B_i + \bar{R}_{i,4} + \bar{R}_{i,5} + \bar{R}_{i,7} + \bar{\Delta}_i + R_{i,8} \end{aligned}$$

where we note that the definition of  $B_i$  does not depend on the split sample, and

$$\begin{aligned} \bar{R}_{i,7} &= \frac{1}{2} [R_{i7,\mathcal{I}} + R_{i7,\mathcal{I}^c}] \Rightarrow \frac{1}{N} \sum_i \|\bar{R}_{i,7}\|^2 = O_P(T^{-3}), \\ \frac{1}{N} \sum_i \|\bar{\Delta}_i\|^2 &= O_P(T^{-3}) \\ R_{i,8} &= -1\{T \text{ is odd}\} \frac{\mathbb{A}_{1i}}{T-1} [\nabla Q_i(\beta_i) - \nabla Q_{i,\mathcal{I}}(\beta_i)], \quad \text{if } |\mathcal{I}| = (T+1)/2 \text{ when } T \text{ is odd.} \end{aligned}$$

Then uniformly in  $y$ ,

$$\frac{1}{N} \sum_i \|R_{i,8}\|^2 \leq O_P\left(\frac{1}{T^2}\right) \frac{1}{N} \sum_i [\|\nabla Q_i(\beta_i)\|^2 + \|\nabla Q_{i,\mathcal{I}}(\beta_i)\|^2] = O_P(T^{-3}).$$

Hence

$$\bar{\beta}_i - \tilde{\beta}_i = -\frac{1}{T} B_i + \bar{\Delta}_i + \bar{R}_{i,4} + \bar{R}_{i,5} + \bar{R}_{i,7} + R_{i,8} - (\Delta_i + R_{i,4} + R_{i,5} + R_{i,7}).$$

So the jackknife debiased estimator  $\hat{\beta}_i := \tilde{\beta}_i - (\bar{\beta}_i - \tilde{\beta}_i)$  admits:

$$\hat{\beta}_i - \beta_i = -\mathbb{A}_{1i} \nabla Q_i(\beta_i) + R_{i,9} + 2R_{i,4} + 2R_{i,5} - \bar{R}_{i,4} - \bar{R}_{i,5}$$

where  $R_{i,9} = 2\Delta_i - \bar{\Delta}_i - R_{i,8} + 2\bar{R}_{i,7} - \bar{R}_{i,7}$  and  $\frac{1}{N} \sum_i \|R_{i,9}\|^2 = O_P(T^{-3})$ .  $\square$

The following lemma characterizes the analytical debias, without assuming time series stationarity.

**Lemma D.2** (Analytical debias). *Use the true value  $\beta_i := \beta_i(y)$  (we drop  $y$  for notational simplicity). The analytical-debiased estimator satisfies: for some  $R_{i,9}$ ,*

$$\hat{\beta}_i - \beta_i = -\mathbb{A}_{1i} \frac{1}{T} \sum_t \psi_{it}(y) + R_{i,4} + R_{i,5} + \tilde{\Delta}_i$$

where  $\sup_y \frac{1}{N} \sum_i \|\tilde{\Delta}_i\|^2 = O_P(L^2 T^{-3})$ .

*Proof.* It follows from Lemma D.5 and Lemma D.3,

$$\begin{aligned} \tilde{\beta}_i - \beta_i &= -\frac{1}{T} B_{i,1T}(y) - \frac{1}{T} B_{i,2T}(y) - \mathbb{A}_{1i} \frac{1}{T} \sum_t \psi_{it}(y) + R_{i,4} + R_{i,5} + \Delta_i \\ &= -\frac{1}{T} \hat{B}_{i,1T}(y) - \frac{1}{T} \hat{B}_{i,2T}(y) - \mathbb{A}_{1i} \frac{1}{T} \sum_t \psi_{it}(y) + R_{i,4} + R_{i,5} \\ &\quad + \underbrace{\Delta_i - \left( \frac{1}{T} \hat{B}_{i,1T}(y) - \frac{1}{T} B_{i,1T}(y) \right) - \left( \frac{1}{T} \hat{B}_{i,2T}(y) - \frac{1}{T} B_{i,2T}(y) \right)}_{\tilde{\Delta}_i}, \end{aligned}$$

where  $\sup_y \frac{1}{N} \sum_i \|\tilde{\Delta}_i\|^2 = O_P(L^2/T^3)$ .  $\square$

Note that Lemma D.3 below does not assume the serial stationarity.

**Lemma D.3** (Undebaised estimator). *Then for some  $\Delta_i$ ,*

$$\tilde{\beta}_i - \beta_i = -\frac{1}{T} B_{i,1T}(y) - \frac{1}{T} B_{i,2T}(y) - \mathbb{A}_{1i} \frac{1}{T} \sum_t \psi_{it}(y) + R_{i,4} + R_{i,5} + \Delta_i$$

where  $\sup_y \frac{1}{N} \sum_i \|\Delta_i\|^2 = O_P(T^{-3})$  and  $\frac{1}{T} \sum_t \psi_{it}(y) = \nabla Q_i(\beta_i)$ .

*Proof.* For notational simplicity, we drop  $y$ . The notation for higher order matrix derivatives associated with Taylor expansions are as defined in Rilstone et al. (1996). For a real-valued function  $Q(\beta)$ , let  $\nabla^3 Q(\beta)$  be a  $\dim(\beta) \times \dim(\beta)^2$  matrix, whose  $j$  th row is given by  $[\text{vec} \nabla^2(\partial_j Q(\beta))]'$ . For instance, when  $\beta = (x, y)'$ , then the first row of  $\nabla^3 Q(x, y)$  is given by

$$[\partial_x^2 g, \partial_{xy} g, \partial_{yx} g, \partial_y^2 g], \quad g = \partial_x Q(x, y).$$

With this notation, the third-order Taylor expansion leads to

$$\tilde{\beta}_i - \beta_i = -\nabla^2 Q_i(\beta_i)^{-1} \nabla Q_i(\beta_i) - \frac{1}{2} \nabla^2 Q_i(\beta_i)^{-1} \nabla^3 Q_i(\beta_i) [(\tilde{\beta}_i - \beta_i) \otimes (\tilde{\beta}_i - \beta_i)] + R_{i,1}$$

where  $\otimes$  denotes Kronecker product and

$$R_{i,1} = -\frac{1}{6}\nabla^2 Q_i(\beta_i)^{-1}\nabla^4 Q_i(\beta_i^*)[(\tilde{\beta}_i - \beta_i) \otimes (\tilde{\beta}_i - \beta_i) \otimes (\tilde{\beta}_i - \beta_i)].$$

Substituting from (D.1),

$$\begin{aligned} \tilde{\beta}_i - \beta_i &= -A_{1i}\nabla Q_i(\beta_i) - \frac{1}{2}A_{1i}A_{2i}[(-A_{1i}\nabla Q_i(\beta_i) + \Delta_i) \otimes (-A_{1i}\nabla Q_i(\beta_i) + \Delta_i)] + R_{i,1} \\ &= -A_{1i}\nabla Q_i(\beta_i) - \frac{1}{2}A_{1i}A_{2i}[(A_{1i}\nabla Q_i(\beta_i)) \otimes (A_{1i}\nabla Q_i(\beta_i))] + R_{i,1} + R_{i,2} \\ &= -A_{1i}\nabla Q_i(\beta_i) - \frac{1}{2}\mathbb{A}_{1i}\mathbb{A}_{2i}[(\mathbb{A}_{1i}\nabla Q_i(\beta_i)) \otimes (\mathbb{A}_{1i}\nabla Q_i(\beta_i))] + R_{i,1} + R_{i,2} + R_{i,3} \\ &= -\mathbb{A}_{1i}\nabla Q_i(\beta_i) - \frac{1}{T}B_{i,1T} + \sum_{d=1}^4 R_{i,d} + [\mathbb{A}_{1i} - A_{1i}]\nabla Q_i(\beta_i) \\ &= -\mathbb{A}_{1i}\nabla Q_i(\beta_i) - \frac{1}{T}B_{i,1T} + \sum_{d=1}^6 R_{i,d} - \frac{1}{T}B_{i,2T} \end{aligned} \quad (\text{D.2})$$

where

$$\begin{aligned} R_{i,2} &= A_{1i}A_{2i} \{ [(-A_{1i}\nabla Q_i(\beta_i) + \Delta_i) \otimes (-A_{1i}\nabla Q_i(\beta_i) + \Delta_i)] - [(A_{1i}\nabla Q_i(\beta_i)) \otimes (A_{1i}\nabla Q_i(\beta_i))] \} \\ R_{i,3} &= \frac{1}{2}\mathbb{A}_{1i}\mathbb{A}_{2i}[(\mathbb{A}_{1i}\nabla Q_i(\beta_i)) \otimes (\mathbb{A}_{1i}\nabla Q_i(\beta_i))] - \frac{1}{2}A_{1i}A_{2i}[(A_{1i}\nabla Q_i(\beta_i)) \otimes (A_{1i}\nabla Q_i(\beta_i))]. \\ R_{i,6} &= \mathbb{A}_{1i}[A_{1i}^{-1} - \mathbb{A}_{1i}^{-1}](A_{1i} - \mathbb{A}_{1i})\nabla Q_i(\beta_i). \end{aligned}$$

By CS and Holder's inequalities, and Lemma D.4, Assumption 5.5,

$$\begin{aligned} \frac{1}{N} \sum_i \|R_{i,1}\|^2 &\leq O_P(1) \left( \frac{1}{N} \sum_{i=1}^N \|\tilde{\beta}_i - \beta_i\|^8 \right)^{3/4} = O_P(T^{-3}). \quad (\text{by Holder } p = 4/3, q = 4) \\ \frac{1}{N} \sum_i \|R_{i,2}\|^2 &\leq O_P(1) \sqrt{\frac{1}{N} \sum_{i=1}^N \|\nabla Q_{y,i}(\beta_i(y))\|^4 \frac{1}{N} \sum_{i=1}^N \|\Delta_i\|^4} + O_P(1) \frac{1}{N} \sum_{i=1}^N \|\Delta_i\|^4 = O_P(T^{-3}). \\ \frac{1}{N} \sum_i \|R_{i,3}\|^2 &\leq O_P(1) \sqrt{\frac{1}{N} \sum_i \|A_{1i} - \mathbb{A}_{1i}\|^4 + \frac{1}{N} \sum_i \|A_{2i} - \mathbb{A}_{2i}\|^4} \sqrt{\frac{1}{N} \sum_i \|\nabla Q_{y,i}(\beta_i(y))\|^8} \\ &= O_P(T^{-3}). \\ \frac{1}{N} \sum_i \|R_{i,6}\|^2 &\leq O_P(1) \sqrt{\frac{1}{N} \sum_i \|A_{1i} - \mathbb{A}_{1i}\|^4} \sqrt{\frac{1}{N} \sum_i \|A_{1i}^{-1} - \mathbb{A}_{1i}^{-1}\|^2} \sqrt{\frac{1}{N} \sum_i \|\nabla Q_{y,i}(\beta_i(y))\|^4} \\ &= O_P(T^{-3}). \\ \frac{1}{N} \sum_i \|R_{i,7}\|^2 &\leq O(T^{-3}), \quad (\text{Assumption 5.2}). \end{aligned}$$

Hence for  $\Delta_i := R_{i,1} + R_{i,2} + R_{i,3} + R_{i,6} + R_{i,7}$ , we have

$$\tilde{\beta}_i - \beta_i = -\mathbb{A}_{1i}\nabla Q_i(\beta_i) - \frac{1}{T}B_{i,1T} - \frac{1}{T}B_{i,2T} + R_{i,4} + R_{i,5} + \Delta_i$$

and  $\sup_y \frac{1}{N} \sum_i \|\Delta_i\|^2 = O_P(T^{-3})$ .

□

**D.2. Technical lemmas.** Lemmas in this subsection do not assume the serial stationarity.

**Lemma D.4.** *Uniformly in  $y \in \mathcal{Y}$ ,*

- (i)  $\frac{1}{N} \sum_{i=1}^N \|\tilde{\beta}_i - \beta_i\|^8 = O_P(T^{-4})$ .
- (ii)  $\frac{1}{N} \sum_{i=1}^N \|\Delta_i\|^4 = O_P(T^{-4})$ .
- (iii)  $\frac{1}{N} \sum_i \|A_{1i} - \mathbb{A}_{1i}\|^4 = O_P(T^{-2})$  and  $\frac{1}{N} \sum_i \|A_{2i} - \mathbb{A}_{2i}\|^4 = O_P(T^{-2})$ .

*Proof.* For notational simplicity, we drop  $y$  in these quantities. We have

$$\tilde{\beta}_i - \beta_i = -\nabla^2 Q_i(b_i)^{-1} \nabla Q_i(\beta_i)$$

where  $b_i$  is between  $\tilde{\beta}_i$  and  $\beta_i$ . Hence

$$\begin{aligned} \sup_y \frac{1}{N} \sum_{i=1}^N \|\tilde{\beta}_i - \beta_i\|^8 &\leq O_P(1) \sup_y \frac{1}{N} \sum_{i=1}^N \|\nabla Q_i(\beta_i)\|^8 \\ &\leq O_P(T^{-4}) \max_i \mathbb{E} \sup_y \left\| \frac{1}{\sqrt{T}} \sum_t \psi_{it}(y) \right\|^8 = O_P(T^{-4}) \end{aligned}$$

where the first inequality is from:  $\sup_y \sup_b \|\nabla^2 Q_i(b)^{-1}\| = O_P(1)$  (Assumption 5.5).

(ii) Since  $\nabla^2 Q_i(\beta)$  is differentiable with a uniformly bounded gradient,

$$\frac{1}{N} \sum_{i=1}^N \|\Delta_i\|^4 \leq \frac{C}{N} \sum_{i=1}^N \|\tilde{\beta}_i - \beta_i\|^8 = O_P(T^{-4}).$$

(iii) Since  $\sup_y \max_i \|A_{1i}\| < C$  almost surely and  $\sup_y \max_i \|\mathbb{A}_{1i}\| < C$ ,

$$\begin{aligned} \frac{1}{N} \sum_i \|A_{1i} - \mathbb{A}_{1i}\|^4 &\leq O_P\left(\frac{1}{T^2}\right) \max_i \mathbb{E} \sup_y \left\| \frac{1}{\sqrt{T}} \sum_t \varpi_{it}^2(y) \right\|^4 = O_P\left(\frac{1}{T^2}\right). \\ \frac{1}{N} \sum_i \|A_{2i} - \mathbb{A}_{2i}\|^4 &\leq O_P\left(\frac{1}{T^2}\right) \max_i \mathbb{E} \sup_y \left\| \frac{1}{\sqrt{T}} \sum_t \varpi_{it}^3(y) \right\|^4 = O_P\left(\frac{1}{T^2}\right). \end{aligned}$$

□

**Lemma D.5.** *Suppose  $V_{i,k}(y)$  is independent of  $W$ . In addition, suppose there is  $a_{y,it}^d$  so that for  $d = 1, 2, \dots$ ,  $\sup_y \frac{1}{NT} \sum_{it} \|a_{y,it}^d\|^4 = O_P(1)$  and for all  $b_1, b_2$ ,*

$$\|\nabla^d q_{y,it}(b_1) - \nabla^d q_{y,it}(b_2)\| \leq \|a_{y,it}^d\| \|b_1 - b_2\|.$$

Also suppose as  $N, T, L \rightarrow \infty$ ,

$$\mathbb{E} \sup_y \left\| \frac{1}{T} \sum_{t=1}^T \ell_{it} \ell'_{it} + \frac{1}{T} \sum_{h=1}^L \sum_{t>h} [\ell_{it} \ell'_{i(t-h)} + \ell_{i(t-h)} \ell'_{it}] - \text{Var}\left(\frac{1}{\sqrt{T}} \sum_t \ell_t\right) \right\|^2 = O_P(T^{-1}).$$

Then uniformly in  $y \in \mathcal{Y}$ ,

- (i)  $\frac{1}{N} \sum_i \|\widehat{B}_{i,1T} - B_{i,1T}\|^2 = O_P(T^{-1})$ .
- (ii)  $\frac{1}{N} \sum_i \|\widehat{B}_{i,2T} - B_{i,2T}\|^2 = O_P(L^2/T)$ .

*Proof.* (i) By Assumption 5.5,  $\|\mathbb{A}_{1i}\|, \|\mathbb{A}_{2i}\|$  and  $\|\widehat{\mathbb{A}}_{2i}\|$  are all bounded uniformly in  $i$  and  $y$ . Then by Lemma D.4  $\frac{1}{N} \sum_i \|\widehat{B}_{i,1T} - B_{i,1T}\|^2 \leq a_1 + a_2 + a_3$  where

$$\begin{aligned} a_1 &= \frac{1}{N} \sum_i \|\widehat{\mathbb{A}}_{1i} - \mathbb{A}_{1i}\|^2 \|\widehat{\mathbb{A}}_{2i} \text{vec}(\widehat{M}_1(y))\|^2 \leq \sqrt{\frac{C}{N} \sum_i \|\widehat{\mathbb{A}}_{1i} - \mathbb{A}_{1i}\|^4} \sqrt{\frac{C}{N} \sum_i \|\widehat{M}_1(y)\|^4} \\ &\leq O_P(T^{-1}) \\ a_2 &= \frac{1}{N} \sum_i \|\mathbb{A}_{1i}(\widehat{\mathbb{A}}_{2i} - \mathbb{A}_{2i}) \text{vec}(\widehat{M}_1(y))\|^2 \leq \sqrt{\frac{C}{N} \sum_i \|\widehat{\mathbb{A}}_{2i} - \mathbb{A}_{2i}\|^4} \sqrt{\frac{C}{N} \sum_i \|\widehat{M}_1(y)\|^4} \\ &\leq O_P(T^{-1}) \\ a_3 &= \frac{1}{N} \sum_i \|\mathbb{A}_{1i} \mathbb{A}_{2i} \text{vec}(\widehat{M}_1(y) - M_1(y))\|^2 \leq \frac{C}{N} \sum_i \|\widehat{\Sigma}_i(y) - \text{Var}(\frac{1}{\sqrt{T}} \sum_t \mathbb{A}_{1i} \psi_{it}(y))\|^2 \end{aligned}$$

and  $\widehat{\Sigma}_i(y) = \frac{1}{T} \sum_t \widehat{\mathbb{A}}_{1i} \widehat{\psi}_{it}(y) \widehat{\psi}_{it}(y)' \widehat{\mathbb{A}}_{1i}$ . Note that

$$\begin{aligned} &\frac{C}{N} \sum_i \|\widehat{\Sigma}_i(y) - \text{Var}(\frac{1}{\sqrt{T}} \sum_t \mathbb{A}_{1i} \psi_{it}(y) | W)\|^2 \leq O_P(T^{-1}) + \sqrt{\frac{C}{NT} \sum_{it} \|\widehat{\psi}_{it}(y) - \psi_{it}(y)\|^4} \\ &\leq O_P(T^{-1}) + \sqrt{\frac{C}{NT} \sum_{it} \|a_{1,it}^1\|^4 \|\widetilde{\beta}_i(y) - \beta_i(y)\|^4} \\ &\leq O_P(T^{-1}) + (\frac{C}{NT} \sum_{it} \|a_{1,it}^1\|^8)^{1/4} (\frac{1}{N} \sum_i \|\widetilde{\beta}_i(y) - \beta_i(y)\|^8)^{1/4} = O_P(T^{-1}). \end{aligned}$$

- (ii)  $\frac{1}{N} \sum_i \|\widehat{B}_{i,2T} - B_{i,2T}\|^2 \leq a_1 + a_2$  where

$$\begin{aligned} a_1 &= \frac{1}{N} \sum_i \|\widehat{\mathbb{A}}_{1i} - \mathbb{A}_{1i}\|^2 \|\widehat{M}_2(y)\|^2 \leq \sqrt{\frac{C}{N} \sum_i \|\widehat{\mathbb{A}}_{1i} - \mathbb{A}_{1i}\|^4} \sqrt{\frac{C}{N} \sum_i \|\widehat{M}_2(y)\|^4} \\ &\leq O_P(T^{-1}) \\ a_2 &= \frac{1}{N} \sum_i \left\| \mathbb{A}_{1i} \begin{pmatrix} \text{tr}(M_{2,1}(y) - \widehat{M}_{2,1}(y)) \\ \vdots \\ \text{tr}(M_{2,\dim(\beta_i)}(y) - \widehat{M}_{2,1}(y)) \end{pmatrix} \right\|^2 \leq \max_k \frac{C}{N} \sum_i \|M_{2,k}(y) - \widehat{M}_{2,k}(y)\|^2 \end{aligned}$$

$$\begin{aligned}
&\leq \max_k \frac{C}{N} \sum_i \left\| \frac{1}{T} \sum_{t=1}^T \ell_{it} \ell'_{it} + \frac{1}{T} \sum_{h=1}^L \sum_{t>h} [\ell_{it} \ell'_{i(t-h)} + \ell_{i(t-h)} \ell'_{it}] - \text{Var}\left(\frac{1}{\sqrt{T}} \sum_t \ell_t\right) \right\|^2 \\
&\quad + \max_k \frac{C}{N} \sum_i \|J_{it}(y) J_{it}(y)' - \hat{J}_{it}(y) \hat{J}_{it}(y)'\|^2 \\
&\quad + \max_k \frac{C}{N} \sum_i \left\| \frac{1}{T} \sum_{h=1}^L \sum_{t>h} [J_{it} J'_{i(t-h)} - \hat{J}_{it} \hat{J}'_{i(t-h)}] \right\|^2 = O_P(L^2/T).
\end{aligned}$$

where  $J_{it}(y) := \mathbb{A}_{1i} \psi_{it}(y) \varpi_{it,k}^2(y)$  and  $\hat{J}_{it}(y)$  is its estimator by replacing  $\mathbb{A}_{1i}$ ,  $\psi_{it}(y)$  and  $\varpi_{it}^2(y)$  with their estimates. □

## APPENDIX E. PROOF OF THEOREM 5.1

**E.1. A high-level weak convergence result.** Suppose a functional estimator has the following expansion:

$$\hat{\vartheta}(y) - \vartheta(y) = \frac{1}{N} \sum_{i=1}^N \left[ \frac{1}{\sqrt{T}} d_{\psi,i}(y) + d_{\gamma,i}(y) \right] + o_P(\zeta_{NT}(y)) \quad (\text{E.1})$$

where  $\zeta_{NT}(y) = (NT)^{-1/2} + N^{-1/2} \|\bar{V}_\gamma(y)\|$ , and define

$$\begin{aligned}
\bar{V}_\psi(y_k, y_l) &= \mathbb{E} d_{\psi,i}(y_k) d_{\psi,i}(y_l), \quad \bar{V}_\gamma(y_k, y_l) = \mathbb{E} d_{\gamma,i}(y_k) d_{\gamma,i}(y_l) \\
\sigma_T^2(y_k, y_l) &= \frac{1}{T} \bar{V}_\psi(y_k, y_l) + \bar{V}_\gamma(y_k, y_l) \\
\sigma_T^2(y) &= \sigma_T^2(y, y), \quad s_{NT}^2(y) = \frac{1}{N} \sigma_T^2(y) \\
\bar{V}_\psi(y) &= \bar{V}_\psi(y, y), \quad \bar{V}_\gamma(y) = \bar{V}_\gamma(y, y) \\
H &= \lim_T \left( \frac{\sigma_T^2(y_k, y_l)}{\sigma_T(y_k) \sigma_T(y_l)} \right)_{M \times M}
\end{aligned}$$

We make the following assumption.

**Assumption E.1.** (i)  $\mathbb{E} d_{\psi,i}(y) = \mathbb{E} d_{\gamma,i}(y) = 0$ ,  $\mathbb{E} d_{\psi,i}(y_k) d_{\gamma,i}(y_l) = 0$  for all  $y, y_k, y_l$ .

(ii) We have  $0 < c < \inf_y \bar{V}_\psi(y) < C$ . In addition,  $\bar{V}_\gamma(y) \in [0, C]$ , with zero as a feasible value for  $\bar{V}_\gamma(y)$ .

(ii)  $\mathbb{E} \sup_y |d_{\psi,i}(y)|^{2+a} + \mathbb{E} \sup_y \left| \frac{d_{\gamma,i}(y)^2}{\bar{V}_\gamma(y)} \right|^a < C$  for some  $a \geq 2$ .

(iii) For any  $\delta > 0$ ,

$$\begin{aligned}
\mathbb{E} \sup_{\rho(y_1, y_2) < \delta} |d_{\psi,i}(y_1) - d_{\psi,i}(y_2)|^2 + \mathbb{E} \sup_{\rho(y_1, y_2) < \delta} \frac{|d_{\gamma,i}(y_1) - d_{\gamma,i}(y_2)|^2}{\sqrt{\bar{V}_\gamma(y_1) \bar{V}_\gamma(y_2)}} &\leq \delta^2 \\
\sup_{\rho(y_1, y_2) < \delta} |\bar{V}_\psi(y_1) - \bar{V}_\psi(y_2)|^2 + \sup_{\rho(y_1, y_2) < \delta} \frac{|\bar{V}_\gamma(y_1) - \bar{V}_\gamma(y_2)|^2}{\bar{V}_\gamma(y_1) \bar{V}_\gamma(y_2)} &\leq \delta^2.
\end{aligned}$$

**Proposition E.1.** *Suppose  $\{d_{\psi,i}(y), d_{\gamma,i}(y) : y \in \mathcal{T}\}$  are i.i.d. across  $i$ . Assumption E.1 holds. In addition, for each  $M$ , and any  $(y_1, \dots, y_M)$ , suppose the  $M \times M$  matrix  $H$  as defined above exists, and  $\lambda_{\min}(H) > c > 0$ .*

Then

$$\frac{\hat{\vartheta}(\cdot) - \vartheta(\cdot)}{s_{NT}(\cdot)} \Rightarrow \mathbb{G}(\cdot)$$

where  $\mathbb{G}(\cdot)$  is a centered Gaussian process with covariance kernel

$$H(y_k, y_l) = \lim_T \frac{\sigma_T^2(y_k, y_l)}{\sigma_T(y_k)\sigma_T(y_l)}.$$

*Proof.* We have  $\hat{\vartheta}(y) - \vartheta(y) = \sum_{i=1}^N \alpha_i(y) + o_P(\zeta_{NT}(y))$  where

$$\alpha_i(y) = \frac{1}{N} \frac{1}{\sqrt{T}} d_{\psi,i}(y) + \frac{1}{N} d_{\gamma,i}(y).$$

Below we prove the weak convergence of  $\sum_i \alpha_i(\cdot)/s_{NT}(\cdot)$ .

(i) show the fidi of  $\sum_i \alpha_i(\cdot)/s_{NT}(\cdot)$ . For any finite integer  $M > 0$ , and any  $y_1, \dots, y_M$ . Let  $A_i = (\alpha_i(y_1)/s_{NT}(y_1), \dots, \alpha_i(y_M)/s_{NT}(y_M))'$ . We shall show

$$\frac{g' \sum_i A_i}{\sqrt{g' H g}} \rightarrow^d \mathcal{N}(0, 1),$$

for any  $g \neq 0$  as an  $M$ -dimensional fixed vector. Here

$$H_T = \text{Var}\left(\sum_i A_i\right) = \left(\frac{\sigma_T^2(y_k, y_l)}{\sigma_T(y_k)\sigma_T(y_l)}\right)_{M \times M}, \quad H = \lim_T H_T,$$

Then the fidi follows from the Cramer-Wold theorem.

We proceed by verifying the Lindeberg condition. First, we bound  $\sum_i \mathbb{E}((g' A_i)^4)$ .

$$\begin{aligned} \sum_i \mathbb{E}((g' A_i)^4) &\leq M \|g\|^4 \sum_i \mathbb{E} \left( \sum_{m=1}^M \frac{\alpha_i(y_m)^4}{s_{NT}^4(y_m)} \right) \\ &\leq M \|g\|^4 \frac{1}{N^4} \sum_i \mathbb{E} \left( \sum_{m=1}^M \frac{\|d_{\psi,i}(y_m)\|^4}{s_{NT}^4(y_m)} \frac{1}{T^2} + \frac{\|d_{\gamma,i}(y_m)\|^4}{s_{NT}^4(y_m)} \right) \\ &\leq C \|g\|^4 \frac{1}{N} \sum_{m=1}^M \mathbb{E} \left[ \frac{d_{\psi,i}(y_m)^4}{\bar{V}_{\psi}(y_m)^2} + \frac{d_{\gamma,i}(y_m)^4}{\bar{V}_{\gamma}(y_m)^2} \right] = O\left(\frac{\|g\|^4}{N}\right). \quad (\text{E.2}) \end{aligned}$$

In addition,  $\lambda_{\min}(H_T) > \lambda_{\min}(H) - o(1) > c$  for large  $T$ . Therefore, for all  $\epsilon > 0$ , we use the inequality that  $\mathbb{E}|Y|1\{|X| > a\} \leq \mathbb{E}|YX^2|/a^2$ ,

$$\frac{1}{g' H_T g} \sum_i \mathbb{E} \left( (g' A_i)^2 1\{|g' A_i| > \epsilon \sqrt{g' H_T g}\} \right)$$

$$\leq \frac{1}{(g'H_T g)^2 \epsilon^2} \sum_i \mathbb{E}((g'A_i)^4) \leq O(N^{-1}).$$

The Lindeberg's central limit theorem then gives  
 $Y_{NT} := g' \sum_i A_i / \sqrt{g'H_T g} \rightarrow^d \mathcal{N}(0, 1)$ . Therefore,

$$\frac{g' \sum_i A_i}{\sqrt{g'H_T g}} = Y_{NT} + Y_{NT} \left( \sqrt{\frac{g'H_T g}{g'H_T g}} - 1 \right) = Y_{NT} + o_P(1) \rightarrow^d \mathcal{N}(0, 1).$$

(ii) Let  $\ell^\infty(\mathcal{Y})$  be the set of all uniformly bounded real functions on  $\mathcal{Y}$ . We show  $\sum_i \alpha_i(\cdot)/s_{NT}(\cdot)$  is asymptotically tight in  $\ell^\infty(\mathcal{Y})$ , by verifying the three conditions of Theorem 2.11.11 in van der Vaart and Wellner (1996). Let

$$\begin{aligned} b_i(y) &= \frac{\frac{1}{\sqrt{T}} d_{\psi,i}(y)}{\sigma_T(y)}, & c_i(y) &= \frac{d_{\gamma,i}(y)}{\sigma_T(y)}. \\ \bar{b}_i(y) &= \frac{\frac{1}{\sqrt{T}} d_{\psi,i}(y)}{[\frac{1}{T} \bar{V}_\psi(y)]^{1/2}}, & \bar{c}_i(y) &= \frac{d_{\gamma,i}(y)}{\bar{V}_\gamma(y)^{1/2}}. \end{aligned} \quad (\text{E.3})$$

Let  $F_i(y) = \frac{a_i}{s_{NT}} = \frac{1}{\sqrt{N}}(b_i(y) + c_i(y))$ . Define  $\rho(y_1, y_2) = C|y_1 - y_2|^{1/4}$  for some  $C > 0$ .

Condition (1). For every  $\eta > 0$ , and an arbitrarily small  $a > 0$ ,

$$\begin{aligned} & \sum_i \mathbb{E} \sup_y |F_i(y)| 1\{\sup_y |F_i(y)| > \eta\} \\ & \leq \eta^{-1} \frac{1}{N} \sum_i \mathbb{E} \sup_y |b_i(y) + c_i(y)|^2 1\{\sup_y |b_i(y) + c_i(y)| > \sqrt{N}\eta\} \\ & \leq \frac{C}{\eta^{a+1} N^{a/2}} \frac{1}{N} \sum_i \mathbb{E} \sup_y |\bar{b}_i(y)|^{2+a} + \frac{1}{\eta^{a+1} N^{a/2}} \frac{1}{N} \sum_i \mathbb{E} \sup_y |\bar{c}_i(y)|^{2+a} = o(1). \end{aligned}$$

Condition (2): For every  $y_1, y_2 \in \mathcal{Y}$ ,

$$\begin{aligned} & \sum_i \mathbb{E} |F_i(y_1) - F_i(y_2)|^2 \leq C \frac{1}{N} \sum_i \mathbb{E} |b_i(y_1) - b_i(y_2)|^2 + C \frac{1}{N} \sum_i \mathbb{E} |c_i(y_1) - c_i(y_2)|^2 \\ & \leq C \mathbb{E} [d_{\psi,i}(y_1) - d_{\psi,i}(y_2)]^2 + C |\bar{V}_\psi(y_1) - \bar{V}_\psi(y_2)|^2 + C \frac{|\bar{V}_\gamma(y_1) - \bar{V}_\gamma(y_2)|^2}{\bar{V}_\gamma(y_1) \bar{V}_\gamma(y_2)} \\ & \quad + \frac{\mathbb{E} |d_{\gamma,i}(y_1) - d_{\gamma,i}(y_2)|^2}{\sqrt{\bar{V}_\gamma(y_1) \bar{V}_\gamma(y_2)}} \leq C |y_1 - y_2|^{1/2} \leq \rho(y_1, y_2)^2. \end{aligned}$$

Condition (3): By Assumption 5.4, for every  $\delta > 0$ ,

$$\begin{aligned} & \sup_{\eta > 0} \sum_i \eta^2 P \left( \sup_{\rho(y_1, y_2) < \delta} |F_i(y_1) - F_i(y_2)| > \eta \right) \\ & \leq \sum_i \mathbb{E} \left( \sup_{\rho(y_1, y_2) < \delta} |F_i(y_1) - F_i(y_2)|^2 \right) \end{aligned}$$

$$\begin{aligned}
 &\leq \frac{1}{N} \sum_i \mathbb{E} \left( \sup_{\rho(y_1, y_2) < \delta} |b_i(y_1) - b_i(y_2)|^2 \right) + \frac{1}{N} \sum_i \mathbb{E} \left( \sup_{\rho(y_1, y_2) < \delta} |c_i(y_1) - c_i(y_2)|^2 \right) \\
 &\leq C \mathbb{E} \sup_{\rho(y_1, y_2) < \delta} |d_{\psi, i}(y_1) - d_{\psi, i}(y_2)|^2 \\
 &\quad + C \left[ \sup_{\rho(y_1, y_2) < \delta} |\bar{V}_{\psi}(y_1) - \bar{V}_{\psi}(y_2)|^2 + \sup_{\rho(y_1, y_2) < \delta} \frac{|\bar{V}_{\gamma}(y_1) - \bar{V}_{\gamma}(y_2)|^2}{\bar{V}_{\gamma}(y_1) \bar{V}_{\gamma}(y_2)} \right] \mathbb{E} \left[ \sup_y d_{\psi, i}(y)^2 + \sup_y \frac{d_{\gamma, i}(y)^2}{\bar{V}_{\gamma}(y)} \right] \\
 &\quad + \mathbb{E} \sup_{\rho(y_1, y_2) < \delta} \frac{|d_{\gamma, i}(y_1) - d_{\gamma, i}(y_2)|^2}{\sqrt{\bar{V}_{\gamma}(y_1) \bar{V}_{\gamma}(y_2)}} \leq \delta^2. \tag{E.4}
 \end{aligned}$$

Thus all conditions are satisfied;  $\frac{\sum_i \alpha_i}{s_{NT}}$  is asymptotically tight.

Together, the process  $\sum_i \alpha_i(\cdot)/s_{NT}(\cdot)$  weakly converges to a centered Gaussian process, with covariance kernel

$$H(y_k, y_l) = \lim_T \frac{\sigma_T^2(y_k, y_l)}{\sigma_T(y_k) \sigma_T(y_l)}.$$

(iii) Next, we show that  $o_P(1) \sup_y \zeta_{NT}(y) s_{NT}^{-1}(y) = o(1)$ . We have

$$\begin{aligned}
 o\left(\frac{1}{\sqrt{NT}}\right) \frac{1}{\inf_y s_{NT}(y)} &= \frac{1}{\inf_y \bar{V}_{\psi}(y)} o(1) = o(1) \\
 o\left(\frac{1}{\sqrt{N}}\right) \sup_y \|\bar{V}_{\gamma}(y)\|^{1/2} s_{NT}^{-1}(y) &\leq o(1) \sup_y \left(\frac{\bar{V}_{\gamma}(y)}{\bar{V}_{\gamma}(y)}\right)^{1/2} = o(1).
 \end{aligned}$$

Hence uniformly in  $y$ ,

$$\frac{\hat{\vartheta}(y) - \vartheta(y)}{s_{NT}(y)} = \frac{\sum_i \alpha_i(y)}{s_{NT}(y)} + o_P(1) \Rightarrow \mathbb{G}$$

This implies the weak convergence . □

## E.2. Proof of Theorem 5.1.

*Proof.* Recall that  $\mathbf{w}_i$  is the exogenous variable and

$$\hat{\boldsymbol{\theta}}(y) = \frac{1}{N} \sum_{i=1}^N \hat{\boldsymbol{\beta}}_i(y) \mathbf{w}_i' S_{wz, N}, \quad S_{wz, N} := \left(\frac{1}{N} W' W\right)^{-1} W' Z (Z' P_W Z)^{-1}.$$

Let  $S_{wz} := C_1^{-1} C_2 (C_2' C_1^{-1} C_2)^{-1}$  where  $C_1 = \sum_i \mathbb{E} \mathbf{w}_i \mathbf{w}_i'$  and  $C_2 = \mathbb{E} \mathbf{w}_i \mathbf{z}_i'$ . Then  $\|S_{wz, N} - S_{wz}\| = O_P(N^{-1/2})$ . Also by Lemma H.2,  $\|\frac{1}{N} \sum_{i=1}^N \gamma_i(y) \mathbf{w}_i'\| = o_P(1) \|\bar{V}_{\gamma}(y)\|^{1/2}$  uniformly in  $y$ . It implies that

$$\frac{1}{N} \sum_{i=1}^N \gamma_i(y) \mathbf{w}_i' S_{wz, N} = \frac{1}{N} \sum_{i=1}^N \gamma_i(y) \mathbf{w}_i' S_{wz} + o_P\left(\frac{1}{\sqrt{N}}\right) \|\bar{V}_{\gamma}(y)\|^{1/2}. \tag{E.5}$$

Write

$$\zeta_{NT}(y) := \frac{1}{\sqrt{NT}} + \frac{1}{\sqrt{N}} \|\bar{V}_\gamma(y)\|^{1/2}. \quad (\text{E.6})$$

By Lemmas D.3, E.1, with assumption  $N = o(T^2)$ , uniformly in  $y \in \mathcal{Y}$ ,

$$\begin{aligned} \hat{\boldsymbol{\theta}}(y) - \boldsymbol{\theta}(y) &= \frac{1}{N} \sum_{i=1}^N [\hat{\boldsymbol{\beta}}_i(y) - \boldsymbol{\beta}_i(y)] \mathbf{w}'_i S_{wz,N} + \frac{1}{N} \sum_{i=1}^N \gamma_i(y) \mathbf{w}'_i S_{wz,N} \\ &= \frac{1}{NT} \sum_{i=1}^N \sum_{t=1}^T \mathbb{A}_{1i}(y) \psi_{it}(y) \mathbf{w}'_i S_{wz,N} + \frac{1}{N} \sum_{i=1}^N \gamma_i(y) \mathbf{w}'_i S_{wz,N} \\ &\quad + \frac{1}{N} \sum_{i=1}^N R_{i,9} \mathbf{w}'_i S_{wz,N} + \frac{1}{N} \sum_{i=1}^N [2R_{i,4} + 2R_{i,5} - \bar{R}_{i,4} - \bar{R}_{i,5}] \mathbf{w}'_i S_{wz,N} \\ &\stackrel{(a)}{=} \frac{1}{NT} \sum_{i=1}^N \sum_{t=1}^T \mathbb{A}_{1i}(y) \psi_{it}(y) \mathbf{w}'_i S_{wz} + \frac{1}{N} \sum_{i=1}^N \gamma_i(y) \mathbf{w}'_i S_{wz} \\ &\quad + O_P(T^{-3/2} + T^{-1}N^{-1/2} + T^{-1/2}N^{-1}) + o_P\left(\frac{1}{\sqrt{N}}\right) \|\bar{V}_\gamma(y)\|^{1/2} \\ &= \frac{1}{NT} \sum_{i=1}^N \sum_{t=1}^T \mathbb{A}_{1i}(y) \psi_{it}(y) \mathbf{w}'_i S_{wz} + \frac{1}{N} \sum_{i=1}^N \gamma_i(y) \mathbf{w}'_i S_{wz} + o_P(\zeta_{NT}(y)), \end{aligned} \quad (\text{E.7})$$

where (a) follows from (E.5) and Lemma H.2. So for  $\eta \neq 0$ , uniformly in  $y$ ,  $\eta' \text{vec}(\hat{\boldsymbol{\theta}}(y) - \boldsymbol{\theta}(y)) = \frac{1}{N} \sum_i \eta' \text{vec}(\frac{1}{\sqrt{T}} a_{\psi,i}(y) + a_{\gamma,i}(y) + o_P(\zeta_{NT}(y)))$  where

$$\begin{aligned} a_{\psi,i}(y) &= \frac{1}{\sqrt{T}} \sum_{t=1}^T \mathbb{A}_{1i}(y) \psi_{it}(y) \mathbf{w}'_i S_{wz} \\ a_{\gamma,i}(y) &= \gamma_i(y) \mathbf{w}'_i S_{wz} \\ V_\psi(y_k, y_l) &= \frac{1}{N} \sum_{i=1}^N \mathbb{E}(\text{vec}(a_{\psi,i}(y_k)) \text{vec}(a_{\psi,i}(y_l))') \\ &= \mathbb{E} \left[ (S'_{wz} \mathbf{w}_i \mathbf{w}'_i S_{wz}) \otimes \left( \mathbb{A}_{1i}(y_k) \mathbb{E} \left( \frac{1}{T} \sum_{s,t \leq T} \psi_{it}(y_k) \psi_{it}(y_l)' | \mathbf{w}_i \right) \mathbb{A}_{1i}(y_l) \right) \right]. \\ V_\gamma(y_k, y_l) &= \frac{1}{N} \sum_{i=1}^N \mathbb{E}(\text{vec}(a_{\gamma,i}(y_k)) \text{vec}(a_{\gamma,i}(y_l))') \\ &= \mathbb{E}[(S'_{wz} \mathbf{w}_i \mathbf{w}'_i S_{wz}) \otimes \mathbb{E}(\gamma_i(y_k) \gamma_i(y_l)' | \mathbf{w}_i)] \\ V_\psi(y) &= V_\psi(y, y), \quad V_\gamma(y) = V_\gamma(y, y). \end{aligned}$$

Note that  $\text{vec}(a_{\psi,i}(y)) = (S'_{wz} \mathbf{w}_i) \otimes \frac{1}{\sqrt{T}} \sum_{t=1}^T \mathbb{A}_{1i}(y) \psi_{it}(y)$ , and  $\text{vec}(a_{\gamma,i}(y_k)) = (S'_{wz} \mathbf{w}_i) \otimes \gamma_i(y_k)$ . Hence  $\hat{\boldsymbol{\theta}} - \boldsymbol{\theta}$  can be written as (H.1) with notation

$$d_{\psi,i}(y) = \eta' \text{vec}(a_{\psi,i}(y)), \quad d_{\gamma,i}(y) = \eta' \text{vec}(a_{\gamma,i}(y))$$

$$\bar{V}_\psi(y_k, y_l) = \eta' V_\psi(y_k, y_l) \eta, \quad \bar{V}_\gamma(y_k, y_l) = \eta' V_\gamma(y_k, y_l) \eta.$$

We apply Proposition E.1 by verifying Assumption E.1.

*Condition (i).* This follows from the assumption that  $\mathbb{E}(\gamma_i(y_l) | \psi_{it}(y_k), \mathbf{w}_i) = 0$  for all  $y_k, y_l$ .

*Condition (ii).* First, note that  $\bar{V}_\gamma(y) \geq \|\eta\|^2 \lambda_{\min}(V_\gamma(y))$  and

$$\begin{aligned} |d_{\psi,i}(y)| &\leq C \|\mathbf{w}_i\| \left\| \frac{1}{\sqrt{T}} \sum_{t=1}^T \psi_{it}(y) \right\|, \quad |d_{\gamma,i}(y)| \leq C \|\gamma_i(y) \mathbf{w}'_i\| \\ \bar{V}_\gamma(y) &\geq \|\eta\|^2 \lambda_{\min}(V_\gamma(y)). \\ \mathbb{E} \sup_y |d_{\psi,i}(y)|^{2+a} &\leq C \sqrt{\mathbb{E} \|\mathbf{w}_i\|^{4+2a} \mathbb{E} \sup_y \left\| \frac{1}{\sqrt{T}} \sum_{t=1}^T \psi_{it}(y) \right\|^{4+2a}} < C \\ \mathbb{E} \sup_y \left| \frac{d_{\gamma,i}(y)}{\bar{V}_\gamma(y)} \right|^a &\leq C \mathbb{E} \sup_y \left[ \frac{\|\gamma_i(y) \mathbf{w}'_i\|^2}{\lambda_{\min}(V_\gamma(y))} \right]^a < C. \end{aligned}$$

*Condition (iii).* We have

$$\begin{aligned} \mathbb{E} \sup_{\rho(y_1, y_2) < \delta} |d_{\psi,i}(y_1) - d_{\psi,i}(y_2)|^2 &\leq C \sup_{\rho(y_1, y_2) < \delta} \|\mathbb{A}_{1i}(y_1) - \mathbb{A}_{1i}(y_2)\|^2 \mathbb{E} \sup_y \left\| \frac{1}{\sqrt{T}} \sum_t \psi_{it} \mathbf{w}'_i \right\|^2 \\ &+ C \mathbb{E} \sup_{\rho(y_1, y_2) < \delta} \left\| \frac{1}{\sqrt{T}} \sum_t \psi_{it}(y_1) - \frac{1}{\sqrt{T}} \sum_t \psi_{it}(y_2) \right\|^2 \|\mathbf{w}_i\|^2 \leq \delta^2. \\ \mathbb{E} \sup_{\rho(y_1, y_2) < \delta} \frac{|d_{\gamma,i}(y_1) - d_{\gamma,i}(y_2)|^2}{\sqrt{\bar{V}_\gamma(y_1) \bar{V}_\gamma(y_2)}} &\leq C \mathbb{E} \sup_{\rho(y_1, y_2) < \delta} \frac{\|\gamma_i(y_1) \mathbf{w}_i - \gamma_i(y_2) \mathbf{w}_i\|^2}{\sqrt{\lambda_{\min}(V_\gamma(y_1)) \lambda_{\min}(V_\gamma(y_2))}} < \delta^2 \\ \sup_{\rho(y_1, y_2) < \delta} |\bar{V}_\psi(y_1) - \bar{V}_\psi(y_2)|^2 &\leq C \sup_{\rho(y_1, y_2) < \delta} \|V_\psi(y_1) - V_\psi(y_2)\|^2 \leq \delta^2 \\ \sup_{\rho(y_1, y_2) < \delta} \frac{|\bar{V}_\gamma(y_1) - \bar{V}_\gamma(y_2)|^2}{\bar{V}_\gamma(y_1) \bar{V}_\gamma(y_2)} &\leq C \sup_{\rho(y_1, y_2) < \delta} \frac{\|V_\gamma(y_1) - V_\gamma(y_2)\|^2}{\lambda_{\min}(V_\gamma(y_1)) \lambda_{\min}(V_\gamma(y_2))} \leq \delta^2 \end{aligned}$$

Hence Assumption E.1 holds. Thus the weak convergence of  $\frac{\eta' \text{vec}(\hat{\boldsymbol{\theta}}(y) - \boldsymbol{\theta}(y))}{s_{NT}(y)}$  follows from Proposition E.1. □

**Lemma E.1.** *Uniformly in  $y \in \mathcal{Y}$ ,*

$$\begin{aligned} (i) \quad \frac{1}{N} \sum_i R_{i,4} \mathbf{w}'_i &= O_P\left(\frac{1}{T\sqrt{N}}\right), \quad \frac{1}{N} \sum_i \bar{R}_{i,4} \mathbf{w}'_i = O_P\left(\frac{1}{T\sqrt{N}}\right) \\ (ii) \quad \frac{1}{N} \sum_i R_{i,5} \mathbf{w}'_i &= O_P\left(\frac{1}{T\sqrt{N}}\right), \quad \text{and} \quad \frac{1}{N} \sum_i \bar{R}_{i,5} \mathbf{w}'_i = O_P\left(\frac{1}{T\sqrt{N}}\right). \end{aligned}$$

*Proof.* (i) **Term**  $\frac{1}{N} \sum_i R_{i,4} \mathbf{w}'_i$ . Recall that  $\frac{1}{N} \sum_i R_{i,4} \mathbf{w}'_i = \frac{1}{N} \sum_i [\mathbb{E}(M_i(y)) - M_i(y)] \mathbf{w}'_i$ , where by  $(AB) \otimes (AB) = (A \otimes A)(B \otimes B)$ ,

$$M_i(y) = \frac{1}{2} \mathbb{A}_{1i} \mathbb{A}_{2i} (\mathbb{A}_{1i} \nabla Q_i(\beta_i)) \otimes (\mathbb{A}_{1i} \nabla Q_i(\beta_i))$$

$$= \frac{1}{2} \mathbb{A}_{1i} \mathbb{A}_{2i} (\mathbb{A}_{1i} \otimes \mathbb{A}_{1i}) (\nabla Q_i(\beta_i) \otimes \nabla Q_i(\beta_i))$$

While this is a random matrix, as the dimension is fixed, we consider a one-dimensional case without loss of generality. In this case,  $M_i(y)$  is a scalar variable, which depends on  $y$  through  $\beta_i$ . Let  $b_i(y) = \frac{1}{2} \mathbb{A}_{1i} \mathbb{A}_{2i} (\mathbb{A}_{1i} \otimes \mathbb{A}_{1i})$  and

$$a_i(y) = T \nabla Q_i(\beta_i) \otimes \nabla Q_i(\beta_i) - T \mathbb{E}[\nabla Q_i(\beta_i) \otimes \nabla Q_i(\beta_i)].$$

Also, let  $F_i(y) = -\frac{1}{\sqrt{N}} a_i(y) b_i(y) \mathbf{w}'_i$ . Then  $\frac{T\sqrt{N}}{N} \sum_i R_{i,4} \mathbf{w}'_i = \sum_i F_i(y)$  and  $\mathbb{E} F_i(y) = 0$ .

Let  $\ell^\infty(\mathcal{Y})$  be the set of all uniformly bounded read functions on  $\mathcal{Y}$ . It suffices to show that  $\sum_i F_i(y)$  is asymptotically tight in  $\ell^\infty(\mathcal{Y})$ , by verifying conditions of Theorem 2.11.11 in van der Vaart and Wellner (1996).

Define a semi-metric  $\rho(y_1, y_2) = \bar{C} |y_1 - y_2|^{1/4}$  for all  $y \in \mathcal{Y}$  and some large  $\bar{C} > 0$ . To verify Condition (1) of the cited theorem, note for every  $\eta > 0$ , and fix some  $0 < a < 2$ , we use the inequality  $x^b 1\{x > \eta\} \leq x^{b+a} \eta^{-a}$  for  $x > 0$  to have:

$$\begin{aligned} & \sum_i \mathbb{E} \sup_y |F_i(y)| 1\{\sup_y |F_i(y)| > \eta\} \\ & \leq \eta^{-1} \frac{1}{N} \sum_i \mathbb{E} \sup_y |a_i(y) b_i(y) \mathbf{w}_i|^2 1\{\sup_y |a_i(y) b_i(y) \mathbf{w}_i| > \sqrt{N} \eta\} \\ & \leq \frac{1}{\eta^{a+1} N^{a/2}} \frac{1}{N} \sum_i \mathbb{E} \sup_y |a_i(y) b_i(y) \mathbf{w}_i|^{2+a} \\ & \leq \frac{C}{\eta^{a+1} N^{a/2}} \frac{1}{N} \sum_i [\mathbb{E} \sup_y |a_i(y)|^m]^b \|\mathbf{w}_i\|^4 \end{aligned}$$

for some constants  $b > 0$  and  $m = 4(2+a)/(2-a)$  using Holder's inequality.

By assumption 5.2 for some  $c > 0$ ,  $\mathbb{E}[\sup_y (\frac{1}{\sqrt{T}} \sum_t \psi_{it}^j(y))^{8+c} |W|] < C$ . Note that without loss of generality, we can write

$$a_i(y) = \frac{1}{\sqrt{T}} \sum_t \psi_{it}^1(y) \frac{1}{\sqrt{T}} \sum_t \psi_{it}^2(y) - \mathbb{E}[\frac{1}{\sqrt{T}} \sum_t \psi_{it}^1(y) \frac{1}{\sqrt{T}} \sum_t \psi_{it}^2(y)]$$

for some functions  $\mathbb{E} \psi_{it}^1(y) = \mathbb{E} \psi_{it}^2(y) = 0$ . This implies  $\frac{1}{N} \sum_i \mathbb{E} \sup_y |a_i(y)|^m < C$ . This verifies Condition (1).

Condition (2): For every  $y_1, y_2 \in \mathcal{Y}$ ,

$$\begin{aligned} & \sum_i \mathbb{E} |F_i(y_1) - F_i(y_2)|^2 \leq \frac{1}{N} \sum_i (\mathbb{E} |a_i(y_1) b_i(y_1) - a_i(y_2) b_i(y_2)|^4)^{1/2} (\mathbb{E} \|\mathbf{w}_i\|^4)^{1/2} \\ & \leq C \frac{1}{N} \sum_i b_i(y_1)^2 \frac{1}{N} \sum_i (\mathbb{E} |a_i(y_1) - a_i(y_2)|^4)^{1/2} + C \frac{1}{N} \sum_i |b_i(y_1) - b_i(y_2)|^2 \frac{1}{N} \sum_i (\mathbb{E} a_i(y_2)^4)^{1/2} \end{aligned}$$

$$\begin{aligned}
 &\leq C \frac{1}{N} \sum_i (\mathbb{E} |a_i(y_1) - a_i(y_2)|^4)^{1/2} + C \frac{1}{N} \sum_i |b_i(y_1) - b_i(y_2)|^2 \\
 &\leq C |y_1 - y_2|^{1/2} \leq C \rho(y_1, y_2)^2.
 \end{aligned}$$

In the third line above,  $\frac{1}{N} \sum_i |b_i(y_1) - b_i(y_2)|^2 < C |y_1 - y_2|^2$  since  $\mathbb{A}_{1i}(y)$  and  $\mathbb{A}_{2i}(y)$  are Lipschitz continuous with universe constants.

To show  $\frac{1}{N} \sum_i (\mathbb{E} |a_i(y_1) - a_i(y_2)|^4)^{1/2} < C |y_1 - y_2|^{1/2}$ , note that the left hand side is bounded by  $I_1 + I_2$  where for  $A^{\otimes 2} := A \otimes A$ ,

$$\begin{aligned}
 I_1 &= \left[ \frac{1}{N} \sum_i \left| \mathbb{E} \left( \frac{1}{\sqrt{T}} \sum_t \psi_{it}(y_1) \right)^{\otimes 2} - \mathbb{E} \left( \frac{1}{\sqrt{T}} \sum_t \psi_{it}(y_2) \right)^{\otimes 2} \right|^4 \right]^{1/2} \leq C |y_1 - y_2|^2 \\
 I_2 &= \left[ \frac{1}{N} \sum_i \mathbb{E} \left| \left( \frac{1}{\sqrt{T}} \sum_t \psi_{it}(y_1) \right)^{\otimes 2} - \left( \frac{1}{\sqrt{T}} \sum_t \psi_{it}(y_2) \right)^{\otimes 2} \right|^4 \right]^{1/2}.
 \end{aligned}$$

The bound for  $I_1$  is due to the Lipschitz continuity with a universe constant (Assumption 5.4). To bound  $I_2$ , we fix any two elements of  $\psi_{it}(y)$ :  $\psi_{it}(y_1)^1$  and  $\psi_{it}(y_1)^2$ , and let  $f_j(y) = \frac{1}{\sqrt{T}} \sum_t \psi_{it}(y)^j$  for  $j = 1, 2$ . Then

$$\begin{aligned}
 &\left[ \frac{1}{N} \sum_i \mathbb{E} |f_1(y_1) f_2(y_1) - f_1(y_2) f_2(y_2)|^4 \right]^{1/2} \\
 &\leq C (\max_{j=1,2} \frac{1}{N} \sum_i \mathbb{E} |f_1(y_1) - f_1(y_2)|^8)^{1/4} (\max_{j=1,2} \sup_y \frac{1}{N} \sum_i \mathbb{E} |f_j(y)|^8)^{1/4} \\
 &\leq C |y_1 - y_2|^{1/2}.
 \end{aligned}$$

The last inequality is due to Assumption 5.2. This verifies Condition (2).

Condition (3): For every  $\delta > 0$ ,

$$\begin{aligned}
 &\sup_{\eta > 0} \sum_i \eta^2 P \left( \sup_{\rho(y_1, y_2) < \delta} |F_i(y_1) - F_i(y_2)| > \eta \right) \\
 &\leq \sum_i \mathbb{E} \left( \sup_{\rho(y_1, y_2) < \delta} |F_i(y_1) - F_i(y_2)|^2 \right) \\
 &\leq \frac{1}{N} \sum_i \mathbb{E} \left( \sup_{\rho(y_1, y_2) < \delta} |a_i(y_1) b_i(y_1) - a_i(y_2) b_i(y_2)|^2 \|\mathbf{w}_i\|^2 \right) \\
 &\leq C \frac{1}{N} \sum_i (\mathbb{E} \sup_{|y_1 - y_2| < (\delta/\bar{C})^4} |a_i(y_1) - a_i(y_2)|^4)^{1/2} + C \frac{1}{N} \sum_i \sup_{|y_1 - y_2| < (\delta/\bar{C})^4} |b_i(y_1) - b_i(y_2)|^2 \\
 &\leq \delta^2
 \end{aligned}$$

by choosing a sufficiently large  $\bar{C}$  in the definition of  $\rho$ . In the above, to bound  $\frac{1}{N} \sum_i (\mathbb{E} \sup_{|y_1 - y_2| < (\delta/\bar{C})^4} |a_i(y_1) - a_i(y_2)|^4)^{1/2}$ , note that a similar argument as verifying

Condition (2) yields, by Assumption 5.2,

$$\begin{aligned} & \frac{1}{N} \sum_i (\mathbb{E} \sup_{|y_1 - y_2| < (\delta/\bar{C})^4} |f_1(y_1)f_2(y_1) - f_1(y_2)f_2(y_2)|^4)^{1/2} \\ & \leq C \frac{1}{N} \sum_i (\mathbb{E} \sup_{|y_1 - y_2| < (\delta/\bar{C})^4} |f_1(y_1) - f_1(y_2)|^8)^{1/4} \\ & \leq C(\delta/\bar{C})^2 < \delta^2. \end{aligned}$$

Hence all sufficient conditions of Theorem 2.11.11 in van der Vaart and Wellner (1996) are verified. Thus  $\sum_i F_i(y) = O_P(1)$  uniformly in  $y$ .

(ii) **Term**  $\frac{1}{N} \sum_i R_{i,5} \mathbf{w}'_i$ . Recall that

$$\begin{aligned} \frac{1}{N} \sum_i R_{i,5} \mathbf{w}'_i &= \frac{1}{T\sqrt{N}} \sum_i F_i(y) \\ F_i(y) &= \frac{1}{\sqrt{N}} \mathbb{A}_{1i} M_i(y) \mathbf{w}'_i \\ M_i(y) &= T(A_{1i}^{-1} - \mathbb{A}_{1i}^{-1}) \mathbb{A}_{1i} \nabla Q_i(\beta_i) - T\mathbb{E}((A_{1i}^{-1} - \mathbb{A}_{1i}^{-1}) \mathbb{A}_{1i} \nabla Q_i(\beta_i)) \end{aligned}$$

We note  $\mathbb{E}F_i(y) = 0$ . It remains to show  $\sum_i F_i(y)$  to be asymptotically tight by verifying the conditions of Theorem 2.11.11 in van der Vaart and Wellner (1996).

Condition (1): for every  $\eta > 0$ , fix  $0 < a < 2$ , by the same argument as for  $\frac{1}{N} \sum_i R_{i,4} \mathbf{w}'_i$ ,

$$\begin{aligned} & \sum_i \mathbb{E} \sup_y |F_i(y)| 1\{\sup_y |F_i(y)| > \eta\} \leq \frac{C}{\eta^{a+1} N^{a/2}} \frac{1}{N} \sum_i \mathbb{E} \sup_y |M_i(y)|^{2+a} \|\mathbf{w}_i\|^{2+a} \\ & \leq \frac{C}{\eta^{a+1} N^{a/2}} \frac{1}{N} \sum_i [\mathbb{E} \sup_y |\sqrt{T}(\mathbb{A}_{1i}^{-1} - A_{1i}^{-1})|^{4+2a}]^{1/2} [\mathbb{E} \sup_y |\sqrt{T} \nabla Q_i(\beta_i)|^{8+4a}]^{1/4} + o(1) \\ & = o(1). \end{aligned}$$

Condition (2). Define  $a_i(y) = \sqrt{T} \mathbb{A}_{1i} [A_{1i}^{-1} - \mathbb{A}_{1i}^{-1}] \mathbb{A}_{1i}$  and  $b_i(y) = \sqrt{T} \nabla Q_i(\beta_i)$ . Then  $F_i(y) = \frac{1}{\sqrt{N}} [a_i(y)b_i(y) - \mathbb{E}a_i(y)b_i(y)] \mathbf{w}'_i$ , for  $\mathbb{E} = \mathbb{E}(\cdot | \mathbf{w}_i)$ ,

$$\begin{aligned} & \sum_i \mathbb{E} |F_i(y_1) - F_i(y_2)|^2 \leq C \frac{1}{N} \sum_i \mathbb{E} |a_i(y_1)b_i(y_1) - a_i(y_2)b_i(y_2)|^2 \|\mathbf{w}_i\|^2 \\ & + C \frac{1}{N} \sum_i \mathbb{E} \|\mathbb{E}a_i(y_1)b_i(y_1) - \mathbb{E}a_i(y_2)b_i(y_2)\|^2 \|\mathbf{w}_i\|^2 \\ & \leq C \frac{1}{N} \sum_i [\mathbb{E} \|a_i(y_1) - a_i(y_2)\|^4]^{1/2} + C \frac{1}{N} \sum_i [\mathbb{E} \|b_i(y_1) - b_i(y_2)\|^4]^{1/2}. \end{aligned}$$

where we used assumption  $\text{Var}(a_i(y) | \mathbf{w}_i) < \infty$ . The second term is bounded by  $C|y_1 - y_2|^{1/2} = C\rho(y_1, y_2)^2$ . We now work on the first term. Let  $c_i(y) = \sqrt{T}[A_{1i}^{-1}(y) - \mathbb{A}_{1i}^{-1}(y)]$ .

$$a_i(y_1) - a_i(y_2) = \mathbb{A}_{1i}(y_1)c_i(y_1)\mathbb{A}_{1i}(y_1) - \mathbb{A}_{1i}(y_2)c_i(y_2)\mathbb{A}_{1i}(y_2)$$

$$\begin{aligned}
 &= [\mathbb{A}_{1i}(y_1) - \mathbb{A}_{1i}(y_2)]c_i(y_1)\mathbb{A}_{1i}(y_1) + \mathbb{A}_{1i}(y_2)[c_i(y_1) - c_i(y_2)]\mathbb{A}_{1i}(y_1) \\
 &\quad + \mathbb{A}_{1i}(y_2)c_i(y_2)[\mathbb{A}_{1i}(y_1) - \mathbb{A}_{1i}(y_2)].
 \end{aligned}$$

Hence

$$\begin{aligned}
 \left[\frac{1}{N} \sum_i \mathbb{E} \|a_i(y_1) - a_i(y_2)\|^4\right]^{1/2} &\leq C \max_i \|\mathbb{A}_{1i}(y_1) - \mathbb{A}_{1i}(y_2)\|^2 \left[\frac{1}{N} \sum_i \mathbb{E} \|c_i(y_1)\|^8\right]^{1/4} \\
 &\quad + \left[\frac{1}{N} \sum_i \mathbb{E} \|c_i(y_1) - c_i(y_2)\|^4\right]^{1/2} \\
 &\leq C |y_1 - y_2|^2 + \left[\frac{1}{N} \sum_i \mathbb{E} \|c_i(y_1) - c_i(y_2)\|^4\right]^{1/2} \\
 &\leq C |y_1 - y_2|^{1/2},
 \end{aligned}$$

where the bound for terms involving  $\mathbb{A}_{1i}(y_1) - \mathbb{A}_{1i}(y_2)$  simply applies the fact that  $\mathbb{A}_{1i}$  is continuously differentiable with respect to  $y$ , with bounded gradients uniformly in  $(y, i)$  (almost surely).

Condition (3): For every  $\delta > 0$ , for sufficiently large  $C$ ,

$$\begin{aligned}
 &\sup_{\eta > 0} \sum_i \eta^2 P \left( \sup_{\rho(y_1, y_2) < \delta} |F_i(y_1) - F_i(y_2)| > \eta \right) \\
 &\leq \frac{1}{N} \sum_i \mathbb{E} \left( \sup_{\rho(y_1, y_2) < \delta} |a_i(y_1)b_i(y_1) - a_i(y_2)b_i(y_2) - \mathbb{E}[a_i(y_1)b_i(y_1) - a_i(y_2)b_i(y_2)]|^2 \|\mathbf{w}_i\|^2 \right) \\
 &\leq C \frac{1}{N} \sum_i (\mathbb{E} \sup_{|y_1 - y_2| < (\delta/\bar{C})^4} |a_i(y_1) - a_i(y_2)|^4)^{1/2} + C \frac{1}{N} \sum_i (\mathbb{E} \sup_{|y_1 - y_2| < (\delta/\bar{C})^4} |b_i(y_1) - b_i(y_2)|^4)^{1/2} \\
 &\quad + C \frac{1}{N} \sum_i \mathbb{E} \left( \sup_{\rho(y_1, y_2) < \delta} \mathbb{E} \|a_i(y_1) - a_i(y_2)\|^2 \|\mathbf{w}_i\|^2 \right) \sup_y \mathbb{E} \|b_i(y)\|^2 \\
 &\quad + C \frac{1}{N} \sum_i \mathbb{E} \left( \sup_{\rho(y_1, y_2) < \delta} \mathbb{E} \|b_i(y_1) - b_i(y_2)\|^2 \|\mathbf{w}_i\|^2 \right) \sup_y \mathbb{E} \|a_i(y)\|^2 \\
 &\leq (C/\bar{C})\delta^2 + C \left[ \frac{1}{N} \sum_i \mathbb{E} \sup_{|y_1 - y_2| < (\delta/\bar{C})^4} \|c_i(y_1) - c_i(y_2)\|^4 \right]^{1/2} \\
 &\quad + C \frac{1}{N} \sum_i (\mathbb{E} \sup_{|y_1 - y_2| < (\delta/\bar{C})^4} |b_i(y_1) - b_i(y_2)|^4)^{1/2} \\
 &\quad + C \sup_{\mathbf{w}_i} \sup_{|y_1 - y_2| < (\delta/\bar{C})^4} [\mathbb{E} \|c_i(y_1) - c_i(y_2)\|^2 + \|b_i(y_1) - b_i(y_2)\|^2] \leq \delta^2.
 \end{aligned}$$

The proof of  $\frac{1}{N} \sum_i \bar{R}_{i,d} \mathbf{w}'_i$  is the same.

□

**Lemma E.2.**  $\inf_y \lambda_{\min}(V_\psi(y)) > c > 0$ .

*Proof.* We first define some notation. For matrices we write  $A \geq 0$  if  $A$  is semipositive definite, and write  $A \geq B$  if  $A - B \geq 0$ . Let  $G_i(y) := \mathbb{A}_{1i}(y) \text{Var}(\frac{1}{\sqrt{T}} \sum_{t \leq T} \psi_{it}(y)) \mathbb{A}_{1i}(y)$ . Let  $S_i = S'_{wz} \mathbf{w}_i \mathbf{w}'_i S_{wz}$  and  $S_{\psi,i}(y) = \text{Var}(\frac{1}{\sqrt{T}} \sum_{t \leq T} \psi_{it}(y) | \mathbf{w}_i)$ . Then almost surely

$$\inf_{Y_M} \min_i \lambda_{\min}(G_i(y)) \geq \inf_{Y_M} \min_i \lambda_{\min}^2(\mathbb{A}_{i,y1}) \min_i \lambda_{\min}(S_{\psi,i}(y)) > c.$$

So  $S_i \otimes [G_i(y) - cI] \geq 0$ , which implies  $S_i \otimes G_i(y) \geq S_i \otimes (cI)$ . Let  $v_y$  be the eigenvector of  $V_\psi(y)$  corresponding to its smallest eigenvalue,

$$\begin{aligned} \inf_{Y_M} \lambda_{\min}(V_\psi(y)) &= \inf_{Y_M} v'_y \mathbb{E}[S_i \otimes G_i(y)] v_y \geq \inf_{Y_M} v'_y [\mathbb{E} S_i \otimes (cI)] v_y \\ &= \inf_{Y_M} v'_y [(\mathbb{E} S_i) \otimes (cI)] v_y \geq \lambda_{\min}[(\mathbb{E} S_i) \otimes (cI)] \\ &= c \lambda_{\min}(\mathbb{E} S_i) = c \lambda_{\min}(S'_{wz} \mathbb{E} \mathbf{w}_i \mathbf{w}'_i S_{wz}) > c. \end{aligned}$$

□

**Lemma E.3.** *Let  $X_i(y_1, y_2)$  be a random variable so that there are  $C, c > 0$ , for all  $\epsilon > 0$   $\frac{1}{N} \sum_i \mathbb{E} \sup_{|y_1 - y_2| \leq \epsilon} \|X_i(y_1, y_2)\| < C\epsilon^c$ . Then for all  $y_1 \neq y_2$ ,*

$$\frac{1}{N} \sum_i \mathbb{E} \|X(y_1, y_2)\| < C|y_1 - y_2|^c.$$

*Proof.*

$$\frac{1}{N} \sum_i \mathbb{E} |X(y_1, y_2)| \leq \sup_{\epsilon > 0} \frac{1}{\epsilon^c} \frac{1}{N} \sum_i \mathbb{E} \sup_{|y_1 - y_2| = \epsilon} \|X(y_1, y_2)\| |y_1 - y_2|^c \leq C|y_1 - y_2|^c.$$

□

## APPENDIX F. PROOF OF THEOREM 5.2

We present the proof for a general case where, consider functionals taking the form

$$\vartheta^g(y) = \mathbb{E}_t f(\beta_i(y), \theta(y), D_{it})$$

for some known function  $f$  and “data”  $D_{it}$ . This admits both the actual distribution  $f(\beta_i(y), \theta(y), D_{it}) = \Lambda(-\mathbf{x}'_{it} \beta_i(y))$ , and the counterfactual distribution  $f(\beta_i(y), \theta(y), D_{it}) = \Lambda(-h_{it}(\mathbf{x}_{it})' \beta_i^g(y))$ , where  $\beta_i^g(y) = \theta(y)[g(\mathbf{z}_i) - \mathbf{z}_i] + \beta_i(y)$ , as special cases.

We apply Proposition E.1 by verifying Assumption E.1. For any random variable  $\mathbf{x}_{it}$ , let

$$\mathbb{Z}_t(\mathbf{x}_{it}) := \frac{\mathbf{x}_{it} - \mathbb{E}_t \mathbf{x}_{it}}{\sqrt{\text{Var}_t(\mathbf{x}_{it})}}$$

where  $\mathbb{E}_t$  and  $\text{Var}_t$  are the expectation and variance operators with respect to the cross-sectional distribution of  $\mathbf{x}_{it}$  given  $t$ .

**F.1. The functional**  $\vartheta^g(y) = \mathbb{E}_t f(\beta_i(y), \theta(y), D_{it})$ . We estimate it by the debiased estimator

$$\widehat{\vartheta}^g(y) = \frac{1}{N} \sum_i f(\widehat{\beta}_i(y), \widehat{\theta}(y), D_{it}) - \frac{1}{2NT} \sum_i \text{tr} \left[ \partial_{\beta}^2 f(\widehat{\beta}_i(y), \widehat{\theta}(y), D_{it}) \widehat{\Sigma}_i(y)^{-1} \right]$$

where  $\widehat{\Sigma}_i(y) = -\nabla^2 Q_{y,i}(\widehat{\beta}_i(y))$ .

Let  $\partial_{\beta} f_i(y) = \partial_{\beta} f_i(\beta_i(y), \theta(y), y)$ ,  $\ddot{f}_{i,\beta} := \partial_{\beta}^2 f(\beta_i(y), \theta(y), D_{it})$ ,  $\ddot{f}_{i,\theta} := \partial_{\theta}^2 f(\beta_i(y), \theta(y), D_{it})$ , and  $\ddot{f}_{i,\beta\theta} := \partial_{\beta\theta}^2 f(\beta_i(y), \theta(y), D_{it})$ . In addition, let  $\bar{G}(y) = \mathbb{E}_t \partial_{\theta} f(\beta_i(y), \theta(y), D_{it})'$ , where  $\partial_{\theta}$  is taken with respect to the coordinates of  $\text{vec}(\theta)$ .

**Assumption F.1.** (i)  $\max_i \mathbb{E} \sup_y \|\nabla f_i\|^8 + \max_i \mathbb{E} \sup_y \|\nabla^2 f_i\|^4 < C$ .

(ii) There is  $C > 0$ , for all  $y_1, y_2$ , and  $i$ ,

$$\mathbb{E} |\partial_{\beta} f_i(y_1) - \partial_{\beta} f_i(y_2)|^4 + \mathbb{E} |\ddot{f}_{i,\beta}(y_1) - \ddot{f}_{i,\beta}(y_2)|^4 \leq C |y_1 - y_2|^4.$$

(iii)  $\mathbb{E}[\psi_{it}(y_k) | \beta_i(y_l), D_{it}] = 0$  and  $\text{Var}_t(d_{\psi,i}(y)) > c > 0$ .

(iv)  $\mathbb{E} \sup_y [\mathbb{Z}_t(\mathbf{w}'_i S_{wz} \bar{G}(y) \gamma_i(y) + f(\beta_i(y), \theta(y), D_{it}))]^4 < C$ .

(v) Write  $f(y) = f(\beta_i(y), \theta(y), D_{it})$  for simplicity.

$$\begin{aligned} \mathbb{E} \sup_{\rho(y_1, y_2) < \delta} \frac{|f(y_1) - \mathbb{E} f(y_1) - (f(y_2) - \mathbb{E} f(y_2))|^2}{\sqrt{\bar{V}_{\gamma}(y_1) \bar{V}_{\gamma}(y_2)}} &\leq \delta^2 \\ \mathbb{E} \sup_{\rho(y_1, y_2) < \delta} \frac{\|\gamma_i(y_1) w' - \gamma_i(y_2) w'\|^2}{\sqrt{\bar{V}_{\gamma}(y_1) \bar{V}_{\gamma}(y_2)}} &\leq \delta^2, \quad \sup_{\rho(y_1, y_2) < \delta} \frac{|\bar{V}_{\gamma}(y_1) - \bar{V}_{\gamma}(y_2)|^2}{\bar{V}_{\gamma}(y_1) \bar{V}_{\gamma}(y_2)} \leq \delta^2. \end{aligned}$$

(vi)  $\sup_y \|\bar{G}(y)\| < C$ , and  $\|\bar{G}(y_1) - \bar{G}(y_2)\| < C |y_1 - y_2|$ .

Define

$$\begin{aligned} \bar{V}_{\psi}(y_k, y_l) &= \mathbb{E}_t [\partial_{\beta} f_i(y_k)' \mathbb{A}_{1i}(y_k) \frac{1}{T} \sum_{sl} \psi_{is}(y_k) \psi_{il}(y_l)' \mathbb{A}_{1i}(y_l) \partial_{\beta} f_i(y_l)], \\ \bar{V}_{\gamma}(y_k, y_l) &= \text{Cov}_t[f(\beta_i(y_k), \theta(y_k), D_{it}), f(\beta_i(y_l), \theta(y_l), D_{it})] \\ \sigma_T^2(y_k, y_l) &= \frac{1}{T} \bar{V}_{\psi}(y_k, y_l) + \bar{V}_{\gamma}(y_k, y_l) \\ \sigma_T^2(y) &= \sigma_T^2(y, y), \quad s_{NT}^2(y) = \frac{1}{N} \sigma_T^2(y) \\ H &= \lim_T \left( \frac{\sigma_T^2(y_k, y_l)}{\sigma_T(y_k) \sigma_T(y_l)} \right)_{M \times M} \end{aligned}$$

**Proposition F.1.** Suppose Assumption F.1 holds. Also,  $N = o(T^2)$  and  $NL^2 = o(T^3)$ . Then

$$\frac{\widehat{\vartheta}^g(\cdot) - \vartheta^g(\cdot)}{s_{NT}(\cdot)} \Rightarrow \mathbb{G}(\cdot)$$

where  $\mathbb{G}(\cdot)$  is a centered Gaussian process with covariance kernel

$$H(y_k, y_l) = \lim_T \frac{\sigma_T^2(y_k, y_l)}{\sigma_T(y_k)\sigma_T(y_l)}.$$

*Proof.* Lemma F.1 shows uniformly in  $y$ ,

$$\widehat{\vartheta}^g(y) - \vartheta^g(y) = \frac{1}{N} \sum_{i=1}^N \left[ \frac{1}{\sqrt{T}} d_{\psi,i}(y) + d_{\gamma,i}(y) \right] + o_P(\zeta_{NT}(y)),$$

where  $\partial_\beta f_i(y) := \partial_\beta f(\beta_i(y), \boldsymbol{\theta}(y), D_{it})$ ,  $\zeta_{NT} = \frac{1}{\sqrt{NT}} + \bar{V}_\gamma(y)$ ,

$$\begin{aligned} d_{\psi,i}(y) &= \frac{1}{\sqrt{T}} \sum_{t=1}^T (\mathbf{w}'_i S_{wz} \bar{G}(y) - \partial_\beta f_i(y)') \mathbb{A}_{1i}(y) \psi_{it}(y) \\ d_{\gamma,i}(y) &= \mathbf{w}'_i S_{wz} \bar{G}(y) \gamma_i(y) + f(\beta_i(y), \boldsymbol{\theta}(y), D_{it}) - \mathbb{E}_t f(\beta_i(y), \boldsymbol{\theta}(y), D_{it}). \end{aligned}$$

We now verify the three conditions in Assumption E.1.

*Assumption E.1 (i).* This follows from  $\mathbb{E}[\psi_{it}(y_k) | \gamma_i(y_l), \mathbf{w}_i, \beta_i(y_l), D_{it}] = 0$ .

*Assumption E.1 (ii).*

$$\begin{aligned} \mathbb{E} \sup_y |d_{\psi,i}(y)|^{2+a} &\leq C \mathbb{E} \sup_y \left\| \frac{1}{\sqrt{T}} \sum_{t=1}^T \psi_{it}(y) \mathbf{w}'_i \right\|^{2+a} + C \mathbb{E} \sup_y \left\| \frac{1}{\sqrt{T}} \sum_{t=1}^T \psi_{it}(y) \partial_\beta f_i(y)' \right\|^{2+a} \\ &< C \\ \mathbb{E} \sup_y \left| \frac{d_{\gamma,i}(y)}{\bar{V}_\gamma(y)} \right|^a &\leq C \mathbb{E} \sup_y [\mathbb{Z}_t(\mathbf{w}'_i S_{wz} \bar{G}(y) \gamma_i(y) + f(\beta_i(y), \boldsymbol{\theta}(y), D_{it}))]^{2a} < C. \end{aligned}$$

*Assumption E.1 (iii).* This condition is verified using the triangular inequality and the primitive inequalities in Assumption F.1.

Hence Assumption E.1 is verified. We then have the weak convergence, following from Proposition E.1.  $\square$

**Lemma F.1.** *Uniformly in  $y$ ,*

$$\begin{aligned} \widehat{\vartheta}^g(y) - \vartheta^g(y) &= o_P(\zeta_{NT}(y)) + \frac{1}{NT} \sum_{it} (\mathbf{w}'_i S_{wz} \bar{G}(y) - \partial_\beta f_i(y)') \mathbb{A}_{1i}(y) \psi_{it}(y) \\ &\quad + \frac{1}{N} \sum_{i=1}^N (\mathbf{w}'_i S_{wz} \bar{G}(y) \gamma_i(y) + [f(\beta_i(y), \boldsymbol{\theta}(y), D_{it}) - \mathbb{E}_t f(\beta_i(y), \boldsymbol{\theta}(y), D_{it})]). \end{aligned}$$

*Proof.* Write  $\partial_\beta f_i(y) := \partial_\beta f(\beta_i(y), \boldsymbol{\theta}(y), D_{it})$ . Let  $G_N(y) := \frac{1}{N} \sum_i \partial_\theta f(\beta_i(y), \boldsymbol{\theta}(y), D_{it})$ , where  $\partial_\theta$  is taken with respect to the coordinates of  $\text{vec}(\theta)$ . By the Taylor expansion up to the second order, (for the first term involving  $\widehat{\theta} - \theta$ , use the identity

$\text{tr}(A'B) = \text{vec}(A)' \text{vec}(B)$ ):

$$\begin{aligned}
& \frac{1}{N} \sum_i f(\hat{\beta}_i(y), \hat{\theta}(y), D_{it}) - f(\beta_i(y), \theta(y), D_{it}) = D_0 + \dots + D_3 + R_1 \\
D_0 &:= \frac{1}{N} \sum_i \partial_{\beta} f_i(y)' (\hat{\beta}_i(y) - \beta_i(y)) \\
D_1 &:= \frac{1}{2N} \sum_i \text{tr} \left[ \ddot{f}_{i,\beta} (\hat{\beta}_i(y) - \beta_i(y)) (\hat{\beta}_i(y) - \beta_i(y))' \right] \\
D_2 &:= \text{tr}[G_N(y)(\hat{\theta}(y) - \theta(y))], \\
&= \text{tr} \left[ \frac{1}{NT} \sum_{it} G_N(y) \mathbb{A}_{1i}(y) \psi_{it}(y) \mathbf{w}'_i S_{wz} \right] + \text{tr} \left[ \frac{1}{N} \sum_{i=1}^N G_N(y) \gamma_i(y) \mathbf{w}'_i S_{wz} \right] + o_P(\zeta_{NT}(y)) \\
&= \frac{1}{NT} \sum_{it} \mathbf{w}'_i S_{wz} G(y) \mathbb{A}_{1i}(y) \psi_{it}(y) + \frac{1}{N} \sum_{i=1}^N \mathbf{w}'_i S_{wz} G(y) \gamma_i(y) + o_P(\zeta_{NT}(y)) \\
D_3 &:= \frac{1}{N} \sum_i (\hat{\beta}_i(y) - \beta_i(y))' \ddot{f}_{i,\beta\theta} (\hat{\theta} - \theta) + (\hat{\theta} - \theta)' \frac{1}{2N} \sum_i \ddot{f}_{i,\theta} (\hat{\theta} - \theta) = o_P(\zeta_{NT}(y)) \\
& \quad (\text{F.1})
\end{aligned}$$

where for some  $a_i$ ,

$$R_1 = \frac{1}{6N} \sum_i \partial_{\beta}^3 f(a_i, D_{it}) (\hat{\beta}_i(y) - \beta_i(y)) \otimes (\hat{\beta}_i(y) - \beta_i(y)) \otimes (\hat{\beta}_i(y) - \beta_i(y)).$$

We have

$$\sup_y R_1 \leq \sup_y \frac{C}{N} \sum_i \|\hat{\beta}_i - \beta_i\|^3 = O_P\left(\frac{1}{T^{3/2}}\right) = o_P\left(\frac{1}{\sqrt{NT}}\right).$$

In the above,  $D_2$  is analyzed by using (E.7). Also all  $o_P$  terms are uniform in  $y$ .

To analyze  $D_0 + D_1$ , by Lemma D.2,  $\hat{\beta}_i - \beta_i = -\mathbb{A}_{1i} \frac{1}{T} \sum_t \psi_{it}(y) + R_{i,4} + R_{i,5} + \tilde{\Delta}_i$  where  $\sup_y \frac{1}{N} \sum_i \|\tilde{\Delta}_i\|^2 = O_P(L^2 T^{-3})$ . Substitute to the above expression,

$$\begin{aligned}
& D_0 + D_1 \\
&= -\frac{1}{N} \sum_i \partial_{\beta} f_i(y)' \mathbb{A}_{1i} \frac{1}{T} \sum_t \psi_{it}(y) + \frac{1}{2NT} \sum_i \text{tr} \left[ \ddot{f}_{i,\beta} \mathbb{E} v_i(y) \right] + \sum_{d=1}^3 H_d \\
H_1 &:= \frac{1}{2NT} \sum_i \text{tr} \left[ \ddot{f}_{i,\beta} (v_i(y) - \mathbb{E} v_i(y)) \right] \\
H_2 &:= \frac{1}{N} \sum_i \partial_{\beta} f_i(y)' (R_{i,4} + R_{i,5}) \\
H_3 &:= \frac{1}{N} \sum_i \partial_{\beta} f_i(y)' \tilde{\Delta}_i - \frac{1}{2N} \sum_i \text{tr} \left[ \ddot{f}_{i,\beta} \mathbb{A}_{1i} \frac{1}{T} \sum_t \psi_{it}(y) (R_{i,4} + R_{i,5})' \right] \\
&\quad - \frac{1}{2N} \sum_i \text{tr} \left[ \ddot{f}_{i,\beta} \mathbb{A}_{1i} \frac{1}{T} \sum_t \psi_{it}(y) \tilde{\Delta}_i' \right]
\end{aligned}$$

$$\begin{aligned}
& + \frac{1}{2N} \sum_i \text{tr} \left[ \ddot{f}_{i,\beta}(R_{i,4} + R_{i,5})(\hat{\beta}_i(y) - \beta_i(y))' \right] + \frac{1}{2N} \sum_i \text{tr} \left[ \ddot{f}_{i,\beta} \tilde{\Delta}_i(\hat{\beta}_i(y) - \beta_i(y))' \right] \\
v_i(y) & := \mathbb{A}_{1i} \frac{1}{\sqrt{T}} \sum_t \psi_{it}(y) \frac{1}{\sqrt{T}} \sum_s \psi_{is}(y)' \mathbb{A}_{1i}.
\end{aligned}$$

We proceed as following steps. Step 1, show  $\sum_{d=1}^3 H_d$  is negligible. Step 2, estimate the bias  $\mathbb{E}v_i(y)$  by  $\hat{\Sigma}_i(y)^{-1}$  and compute the debiased estimator, and show that the bias estimation is negligible.

**step 1.** Write  $F_i(y) = \frac{1}{2\sqrt{N}} \text{tr} \left[ \ddot{f}_{i,\beta}(v_i(y) - \mathbb{E}v_i(y)) \right]$ . Then  $H_1 = \frac{1}{T\sqrt{N}} \sum_i F_i(y)$ . We now show  $\sum_i F_i(y) = O_P(1)$  uniformly in  $y$  by showing it is asymptotically tight. For notational simplicity, we focus on an arbitrary element of  $\ddot{f}_{i,\beta}B_i(y)$  and continue using  $\ddot{f}_{i,\beta}B_i(y)$  to denote this element with abuse of notation. Since the dimension of  $\beta_i(y)$  is fixed, this does not affect the asymptotic behavior. For any  $\eta > 0$ , and  $a > 0$ ,

$$\begin{aligned}
& \sum_i \mathbb{E} \sup_y |F_i(y)| 1\{\sup_y |F_i(y)| > \eta\} \leq \frac{1}{\eta} \sum_i \mathbb{E} \sup_y |F_i(y)|^2 1\{\sup_y |F_i(y)| > \eta\} \\
& = \frac{1}{4N\eta} \sum_i \mathbb{E} \sup_y \left[ \ddot{f}_{i,\beta}(v_i(y) - \mathbb{E}v_i(y)) \right]^2 1\{\sup_y \left| \ddot{f}_{i,\beta}(v_i(y) - \mathbb{E}v_i(y)) \right| > 2\sqrt{N}\eta\} \\
& \leq \frac{1}{4N^{a/2}\eta^{1+a}} \frac{1}{N} \sum_i \mathbb{E} \sup_y \left[ \ddot{f}_{i,\beta}(v_i(y) - \mathbb{E}v_i(y)) \right]^{2+a} \\
& \leq \frac{C}{N^{a/2}\eta^{1+a}} \frac{1}{N} \sum_i [\mathbb{E} \sup_y [v_i(y) - \mathbb{E}v_i(y)]^4]^{(2+a)/4} = o(1)
\end{aligned}$$

provided that  $\mathbb{E} \sup_y [v_i(y) - \mathbb{E}v_i(y)]^4 \leq C \mathbb{E} \sup_y v_i(y)^4$  and  $\max_i \mathbb{E} \sup_y \|\ddot{f}\|^{4/3} < C$ .

We recall that  $\ddot{f}_{i,\beta}$  depends on  $y$  through  $\beta_i(y)$ . For every  $y_1, y_2 \in \mathcal{Y}$ , by Assumption 5.2 and Lemma E.3,  $\frac{1}{N} \sum_i \mathbb{E}(v_i(y_1) - v_i(y_2))^4 \leq C|y_1 - y_2|$ . Hence

$$\begin{aligned}
& \sum_i \mathbb{E} |F_i(y_1) - F_i(y_2)|^2 \leq \frac{C}{N} \sum_i (\mathbb{E} |\ddot{f}_{i,\beta}(y_1) - \ddot{f}_{i,\beta}(y_2)|^4)^{1/2} (\mathbb{E} v_i(y_1)^4)^{1/2} \\
& + \left[ \frac{C}{N} \sum_i \mathbb{E}(v_i(y_1) - v_i(y_2))^4 \right]^{1/2} \leq C|y_1 - y_2|^2 + C|y_1 - y_2|^{1/2} \leq C|y_1 - y_2|^{1/2}.
\end{aligned}$$

For every  $\delta > 0$ , and  $\rho(y_1, y_2) = \bar{C}|y_1 - y_2|^{1/4}$ , for sufficiently large  $\bar{C}$ ,

$$\begin{aligned}
& \sup_{\eta > 0} \sum_i \eta^2 P \left( \sup_{\rho(y_1, y_2) < \delta} |F_i(y_1) - F_i(y_2)| > \eta \right) \leq \sum_i \mathbb{E} \left( \sup_{\rho(y_1, y_2) < \delta} |F_i(y_1) - F_i(y_2)|^2 \right) \\
& \leq \frac{C}{N} \sum_i (\mathbb{E} \sup_{\rho(y_1, y_2) < \delta} |\ddot{f}_{i,\beta}(y_1) - \ddot{f}_{i,\beta}(y_2)|^4)^{1/2} (\mathbb{E} \sup_y v_i(y)^4)^{1/2}
\end{aligned}$$

$$+ [\frac{C}{N} \sum_i \mathbb{E} \sup_{\rho(y_1, y_2) < \delta} (v_i(y_1) - v_i(y_2))^4]^{1/2} \leq \delta^2.$$

Hence all conditions of Theorem 2.11.11 in van der Vaart and Wellner (1996) are verified. Thus  $\sum_i F_i(y) = O_P(1)$  uniformly in  $y$ . This implies  $\sup_y H_1 = O_P(\frac{1}{T\sqrt{N}})$ . In addition, it follows from the same argument of that of Lemma E.1 that  $\sup_y H_2 = O_P(\frac{1}{T\sqrt{N}})$ . Next, by Cauchy-Schwarz inequality, uniformly in  $y$ ,

$$\begin{aligned} H_3^2 &\leq O_P(1) \frac{1}{N} \sum_i \|\tilde{\Delta}_i\|^2 + O_P(1) \left( \frac{1}{N} \sum_i \left[ \frac{1}{T} \sum_t \psi_{it}(y) \right]^4 \right)^{1/2} \frac{1}{N} \sum_i [\|R_{i,4} + R_{i,5}\|^2 + \|\tilde{\Delta}_i\|^2] \\ &\quad + O_P(1) \left( \frac{1}{N} \sum_i [\hat{\beta}_i - \beta_i]^4 \right)^{1/2} \frac{1}{N} \sum_i [\|R_{i,4} + R_{i,5}\|^2 + \|\tilde{\Delta}_i\|^2] = O_P\left(\frac{1}{T^3} + \frac{L^2}{T^4}\right). \end{aligned}$$

Together, provided that  $N = o(T^2)$  and  $NL^2 = o(T^3)$ ,

$$\sup_y |H_1 + H_2 + H_3| = O_P\left(\frac{1}{T\sqrt{N}} + \frac{1}{T^{3/2}} + \frac{L}{T^2}\right) = o_P\left(\frac{1}{\sqrt{NT}}\right).$$

**Step 2.** Bias correction. Because  $\psi_{is}(y)$  is a martingale difference, and the loss function is the log-likelihood,

$$\mathbb{E} v_i(y) = \mathbb{A}_{1i} \frac{1}{T} \sum_t \mathbb{E} \psi_{it}(y) \psi_{it}(y)' \mathbb{A}_{1i} = -\mathbb{A}_{1i}.$$

The effect of bias correction is: uniformly in  $y$ ,

$$\begin{aligned} &\frac{1}{2NT} \sum_i \text{tr} \left[ \partial_{\beta}^2 f(\hat{\beta}_i(y), D_{it}) \hat{\Sigma}_i(y)^{-1} \right] - \frac{1}{2NT} \sum_i \text{tr} \left[ \partial_{\beta}^2 f(\beta_i(y), D_{it}) \mathbb{E} v_i(y) \right] \\ &\leq \frac{1}{2NT} \sum_i \text{tr} \left[ \partial_{\beta}^2 f(\hat{\beta}_i(y), D_{it}) - \partial_{\beta}^2 f(\beta_i(y), D_{it}) \right] \hat{\Sigma}_i(y)^{-1} \\ &\quad + \frac{1}{2NT} \sum_i \text{tr} \partial_{\beta}^2 f(\beta_i(y), D_{it}) \left[ \hat{\Sigma}_i(y)^{-1} - \mathbb{E} v_i(y) \right] \\ &\leq \frac{C}{T} \left( \frac{1}{N} \sum_i \|\hat{\beta}_i(y) - \beta_i(y)\|^2 \right)^{1/2} \left( \frac{1}{N} \sum_i \|\hat{\Sigma}_i(y)\|^2 \right)^{1/2} + \frac{C}{T} \left( \frac{1}{N} \sum_i \|\hat{\Sigma}_i(y)^{-1} - \mathbb{E} v_i(y)\|^2 \right)^{1/2} \\ &= O_P\left(\frac{1}{T^{3/2}}\right) = o_P\left(\frac{1}{\sqrt{NT}}\right), \end{aligned}$$

where we used

$$\frac{1}{N} \sum_i \|\hat{\Sigma}_i(y)^{-1} - \mathbb{E} v_i(y)\|^2 \leq O_P(1) \frac{1}{N} \sum_i \|\nabla^2 Q_i(\hat{\beta}_i(y))^{-1} - [\nabla^2 \mathbb{E} Q_i(\beta_i(y))]^{-1}\|^2 = O_P\left(\frac{1}{T}\right).$$

So

$$\begin{aligned}
& \frac{1}{N} \sum_i f(\widehat{\beta}_i(y), \widehat{\theta}(y), D_{it}) - \frac{1}{2NT} \sum_i \text{tr} \left[ \partial_{\beta}^2 f(\widehat{\beta}_i(y), \widehat{\theta}(y), D_{it}) \widehat{\Sigma}_i(y)^{-1} \right] - f(\beta_i(y), \theta(y), D_{it}) \\
&= \frac{1}{NT} \sum_{it} [\mathbf{w}'_i S_{wz} G(y) - \partial_{\beta} f_i(y)'] \mathbb{A}_{1i}(y) \psi_{it}(y) + \frac{1}{N} \sum_{i=1}^N \mathbf{w}'_i S_{wz} G(y) \gamma_i(y) + o_P(\zeta_{NT}(y)).
\end{aligned}$$

□

## F.2. Proof of Theorem 5.2.

*Proof.* We now apply Proposition F.1 to obtain the weak convergence of the cross-sectional distributions. This boils down to verifying Assumption F.1 for  $G_t$ .

**For  $F_t$ .** In this case  $f(b, D_{it}) = \Lambda(-\mathbf{x}'_{it}b)$ .

*Verifying Assumption F.1(i).* We have  $\partial_{\beta} f_i = -\dot{\Lambda}(-\mathbf{x}'_{it}\beta_i(y))\mathbf{x}_{it}$ , and  $\ddot{f}_i = \ddot{\Lambda}(-\mathbf{x}'_{it}\beta_i(y))\mathbf{x}_{it}\mathbf{x}'_{it}$ . Then

$$\max_i \mathbb{E} \sup_y \|\partial_{\beta} f_i\|^8 + \max_i \mathbb{E} \sup_y \|\ddot{f}_{i,\beta}\|^4 \leq C \max_i \mathbb{E} \|\mathbf{x}_{it}\|^8 < C$$

*Verifying Assumption F.1(ii).* For  $k \geq 4$ ,

$$\begin{aligned}
\mathbb{E} \|\ddot{f}_{i,\beta}(y_1) - \ddot{f}_{i,\beta}(y_2)\|^4 &\leq \mathbb{E} |\ddot{\Lambda}(-\mathbf{x}'_{it}\beta_i(y_1)) - \ddot{\Lambda}(-\mathbf{x}'_{it}\beta_i(y_2))|^4 \|\mathbf{x}_{it}\|^8 \leq C |y_1 - y_2|^4 \\
\mathbb{E} |\partial_{\beta} f_i(y_1) - \partial_{\beta} f_i(y_2)|^4 &\leq \mathbb{E} |\dot{\Lambda}(-\mathbf{x}'_{it}\beta_i(y_1)) - \dot{\Lambda}(-\mathbf{x}'_{it}\beta_i(y_2))|^4 \|\mathbf{x}_{it}\|^4 \leq C |y_1 - y_2|^4.
\end{aligned}$$

*Verifying Assumption F.1(iii).* This holds given  $\mathbb{E}[\psi_{it}(y_k)|\beta_i(y_t), \mathbf{x}_{it}] = 0$  and

$$\begin{aligned}
\text{Var}_t(d_{\psi,i}(y)) &= \mathbb{E}_t \dot{\Lambda}(-\mathbf{x}'_{it}\beta_i(y))^2 \mathbf{x}'_{it} \mathbb{A}_{1i} \text{Var}_t\left(\frac{1}{\sqrt{T}} \sum_s \psi_{is}(y) | \mathbf{x}_{it}, \beta_i(y)\right) \mathbb{A}_{1i} \mathbf{x}_{it} \\
&\geq \lambda_{\min}(\text{Var}_t\left(\frac{1}{\sqrt{T}} \sum_s \psi_{is}(y) | \mathbf{x}_{it}, \beta_i(y)\right)) \lambda_{\min}(\mathbb{A}_{1i}(y)^2) \mathbb{E}_t \dot{\Lambda}(-\mathbf{x}'_{it}\beta_i(y))^2 \|\mathbf{x}_{it}\|^2 > c.
\end{aligned}$$

*Verifying Assumption F.1(iv).* This holds since  $\mathbb{E} \sup_y [\mathbb{Z}_t(\Lambda(-\mathbf{x}'_{it}\beta_i(y)))]^4 < C$ .

*Verifying Assumption F.1(v).* This holds for  $f(\beta_i(y), D_{it}) = \Lambda(-\mathbf{x}'_{it}\beta_i(y))$ .

Therefore by Proposition F.1,

$$\frac{\widehat{F}_t(\cdot) - F_t(\cdot)}{s_{NT}(\cdot)} \Rightarrow \mathbb{G}(\cdot), \quad \frac{\widehat{F}_{t,I}(\cdot) - F_{t,I}(\cdot)}{s_{NT,I}(\cdot)} \Rightarrow \mathbb{G}_I(\cdot).$$

**For  $G_t$ .** In this case  $f(\beta_i(y), \theta(y), D_{it}) = \Lambda(-h_{it}(\mathbf{x}_{it})' \beta_i^g(y))$ , where

$$\beta_i^g(y) = \theta(y)[g(\mathbf{z}_i) - \mathbf{z}_i] + \beta_i(y).$$

*Verifying Assumption F.1(i).* We have  $\partial_{\beta} f_i = -\dot{\Lambda}(-h_{it}(\mathbf{x}_{it})' \beta_i^g(y)) h_{it}(\mathbf{x}_{it})$ , and  $\ddot{f}_{i,\beta} = \ddot{\Lambda}(-h_{it}(\mathbf{x}_{it})' \beta_i^g(y)) h_{it}(\mathbf{x}_{it}) h_{it}(\mathbf{x}_{it})'$ .

$$\max_i \mathbb{E}_t \sup_y \|\partial_{\beta} f_i\|^8 + \max_i \mathbb{E}_t \sup_y \|\partial_{\theta} f_i\|^8 \leq C \mathbb{E}_t \|h_{it}(\mathbf{x}_{it})\|^8 + C \mathbb{E} \|h_{it}(\mathbf{x}_{it})\|^8 \|g(\mathbf{z}_i) - \mathbf{z}_i\|^8 < C$$

$$\begin{aligned} \max_i \mathbb{E}_t \sup_y \|\ddot{f}_{i,\beta}\|^4 + \max_i \mathbb{E}_t \sup_y \|\ddot{f}_{i,\theta}\|^4 &\leq C \mathbb{E}_t \|h_{it}(\mathbf{x}_{it})\|^8 + C \mathbb{E}_t \|h_{it}(\mathbf{x}_{it})\|^8 \|g(\mathbf{z}_i) - \mathbf{z}_i\|^8 < C \\ \max_i \mathbb{E}_t \sup_y \|\ddot{f}_{i,\beta\theta}\|^4 &\leq C \mathbb{E}_t \|h_{it}(\mathbf{x}_{it})\|^8 \|g(\mathbf{z}_i) - \mathbf{z}_i\|^4 < C. \end{aligned}$$

Verifying Assumption F.1(ii). This holds by the assumption that for  $k \geq 4$ ,

$$\begin{aligned} \mathbb{E}_t |\ddot{\Lambda}(-h_{it}(\mathbf{x}_{it})' \beta_i^g(y_1)) - \ddot{\Lambda}(-h_{it}(\mathbf{x}_{it})' \beta_i^g(y_2))|^k \|h_{it}(\mathbf{x}_{it})\|^{2k} &\leq C |y_1 - y_2|^k \\ \mathbb{E}_t |\dot{\Lambda}(-h_{it}(\mathbf{x}_{it})' \beta_i^g(y_1)) - \dot{\Lambda}(-h_{it}(\mathbf{x}_{it})' \beta_i^g(y_2))|^k \|h_{it}(\mathbf{x}_{it})\|^k &\leq C |y_1 - y_2|^k. \end{aligned}$$

Verifying Assumption F.1(iii). This holds for  $\mathbb{E}[\psi_{it}(y_k) | \beta_i(y_l), h_{it}(\mathbf{x}_{it}), \mathbf{z}_i, \mathbf{w}_i] = 0$  and

$$\begin{aligned} \text{Var}_t(d_{\psi,i}(y)) &\geq \lambda_{\min}(\text{Var}_t(\frac{1}{\sqrt{T}} \sum_s \psi_{is}(y) | h_{it}(\mathbf{x}_{it}), \mathbf{z}_i, \beta_i(y))) \lambda_{\min}(\mathbb{A}_{1i}(y)^2) \\ &\quad \times \mathbb{E}_t \|\mathbf{w}_i' S_{wz} \bar{G}(y) + \dot{\Lambda}(-h_{it}(\mathbf{x}_{it})' \beta_i^g(y)) h_{it}(\mathbf{x}_{it})'\| > c. \end{aligned}$$

Verifying Assumption F.1(iv). This holds since

$$\mathbb{E} \sup_y [\mathbb{Z}_t(\mathbf{w}_i' S_{wz} \bar{G}(y) \gamma_i(y) + \Lambda(-h_{it}(\mathbf{x}_{it})' \beta_i^g(y)))]^4 < C.$$

Verifying Assumption F.1(v). This holds for  $f(\beta_i(y), \theta(y), D_{it}) = \Lambda(-h_{it}(\mathbf{x}_{it})' \beta_i^g(y))$ .

Verifying Assumption F.1(vi). Note that

$$\bar{G}(y) = -\mathbb{E}_t \dot{\Lambda}(-h_{it}(\mathbf{x}_{it})' \beta_i^g(y)) \text{vec}(h_{it}(\mathbf{x}_{it})(g(\mathbf{z}_i) - \mathbf{z}_i)').$$

Hence  $\sup_y \|\bar{G}(y)\| \leq C \mathbb{E}_t \|h_{it}(\mathbf{x}_{it})\| \|g(\mathbf{z}_i) - \mathbf{z}_i\| < C$ , and

$$\|\bar{G}(y_1) - \bar{G}(y_2)\| \leq C \mathbb{E}_t |\dot{\Lambda}(-h_{it}(\mathbf{x}_{it})' \beta_i^g(y_1)) - \dot{\Lambda}(-h_{it}(\mathbf{x}_{it})' \beta_i^g(y_2))| \|h_{it}(\mathbf{x}_{it})[g(\mathbf{z}_i) - \mathbf{z}_i]'\| \leq C |y_1 - y_2|.$$

Therefore by Proposition F.1, for  $F \in \{F_t, G_t\}$  and  $\hat{F} \in \{\hat{F}_t, \hat{G}_t\}$

$$\frac{\hat{F}(\cdot) - F(\cdot)}{s_{NT}(\cdot)} \Rightarrow \mathbb{G}(\cdot).$$

□

## APPENDIX G. PROOF OF THEOREM 5.3: THE COUNTERFACTUAL QE

Consider a generic  $F \in \{F_t, G_t\}$ . Let  $\hat{F} \in \{\hat{F}_t, \hat{G}_t\}$  be its estimator. The goal is to obtain an expansion for  $\phi(\hat{F}, \tau) - \phi(F, \tau)$  uniformly in  $\tau$ . The novelty of our analysis is that  $\hat{F} - F$  does not weakly converge due to the issue of unknown rate of convergence we discussed earlier. Hence the usual functional delta-method is not directly applicable. Instead, we obtain an expansion for the standardized  $\phi(\hat{F}, \tau) - \phi(F, \tau)$ .

*Proof.* Lemma G.1 below shows the uniform expansions of  $\phi(\widehat{F}, \tau) - \phi(F, \tau)$  for  $F \in \{F_t, G_t\}$  and  $\widehat{F} \in \{\widehat{F}_t, \widehat{G}_t\}$ . This implies

$$\widehat{\mathbb{Q}\mathbb{E}}(\tau) - \mathbb{Q}\mathbb{E}(\tau) = \frac{1}{N} \sum_{i=1}^N \left[ \frac{1}{\sqrt{T}} p_{\psi,i}^{II}(\tau) + p_{\gamma,i}^{II}(\tau) \right] + o_P\left(\frac{1}{\sqrt{NT}} + \text{Var}_t(p_{\gamma,i}^{II}(\tau))\right),$$

where for  $q_0(\tau) = \phi(F_t, \tau)$ ,  $q_{II}(\tau) = \phi(G_t, \tau)$ ,

$$p_{\psi,i}^{II}(\tau) = \frac{-d_{\psi,i}^{II}(q_{II}(\tau))}{\dot{G}_t(q_{II}(\tau))} + \frac{d_{\psi,i}^0(q_0(\tau))}{\dot{F}_t(q_0(\tau))}, \quad p_{\gamma,i}^{II}(\tau) = \frac{-d_{\gamma,i}^{II}(q_{II}(\tau))}{\dot{G}_t(q_{II}(\tau))} + \frac{d_{\gamma,i}^0(q_0(\tau))}{\dot{F}_t(q_0(\tau))}. \quad (\text{G.1})$$

We also used the assumption that  $\text{Var}_t(d_{\gamma,i}^0) + \text{Var}_t(d_{\gamma,i}^{II}) = O(\text{Var}_t(p_{\gamma,i}^{II}))$ . From here, establishing the weak convergence can be done via applying Proposition E.1. We now verify the three conditions in Assumption E.1.

*Assumption E.1 (i).* This follows from the assumption.

*Assumption E.1 (ii).*

$$\begin{aligned} \mathbb{E} \sup_y |p_{\psi,i}^{II}(y)|^{2+a} &\leq C \mathbb{E} \sup_y [|d_{\psi,i}^0(y)| + |d_{\psi,i}^{II}(y)|]^{2+a} < C \\ \mathbb{E} \sup_y \left| \frac{p_{\gamma,i}^{II}(y)^2}{\text{Var}_t(p_{\gamma,i}^{II}(y))} \right|^a &\leq \mathbb{E} \sup_y \left| \frac{d_{\gamma,i}^0(y)^2}{\text{Var}_t(p_{\gamma,i}^{II}(y))} \right|^a + \mathbb{E} \sup_y \left| \frac{d_{\gamma,i}^{II}(y)^2}{\text{Var}_t(p_{\gamma,i}^{II}(y))} \right|^a \\ &\leq \mathbb{E} \sup_y \left| \frac{d_{\gamma,i}^0(y)^2}{\text{Var}_t(d_{\gamma,i}^0(y))} \right|^a + \mathbb{E} \sup_y \left| \frac{d_{\gamma,i}^{II}(y)^2}{\text{Var}_t(d_{\gamma,i}^{II}(y))} \right|^a \leq C \end{aligned}$$

where we also used the assumption  $\text{Var}_t(d_{\gamma,i}^0) + \text{Var}_t(d_{\gamma,i}^{II}) = O(\text{Var}_t(p_{\gamma,i}^{II}))$ .

*Assumption E.1 (iii).* This condition is verified using the triangular inequality and the primitive inequalities in Assumption F.1.

Hence Assumption E.1 is verified. We then have the weak convergence, following from Proposition E.1.  $\square$

**Lemma G.1.** *Let  $\dot{F}$  be the density of  $F \in \{F_t, G_t\}$ . Let  $q(\tau) = \phi(F, \tau)$ ,  $z(y) = (NT)^{-1/2} + N^{-1/2} \text{Var}_t(d_{\gamma,i}(y))^{1/2}$ . Uniformly in  $\tau$ , we have*

$$\phi(\widehat{F}, \tau) - \phi(F, \tau) = \frac{-1}{\dot{F}(q(\tau))} \frac{1}{N} \sum_i \left[ \frac{1}{\sqrt{T}} d_{\psi,i}(q(\tau)) + d_{\gamma,i}(q(\tau)) \right] + o_P(z(q(\tau))),$$

where  $(d_{\psi,i}, d_{\gamma,i}) \in \{(d_{\psi,i}^0, d_{\gamma,i}^0), (d_{\psi,i}^{II}, d_{\gamma,i}^{II})\}$ , corresponding to  $F \in \{F_t, G_t\}$ .

*Proof.* Consider a generic  $F \in \{F_t, G_t\}$ . Let  $\widehat{F} \in \{\widehat{F}_t, \widehat{G}_t\}$  be its estimator. Note that  $F(\phi(F, \tau)) = \widehat{F}(\phi(\widehat{F}, \tau)) = \tau$ , we have

$$F(\phi(\widehat{F}, \tau)) - F(\phi(F, \tau)) = -[\widehat{F}(\phi(\widehat{F}, \tau)) - F(\phi(\widehat{F}, \tau))]. \quad (\text{G.2})$$

Applying the mean value theorem to the left hand side, there is  $\tilde{q}_\tau$  so that

$$\phi(\hat{F}, \tau) - \phi(F, \tau) = \frac{-1}{\dot{F}(\tilde{q}_\tau)} [\hat{F}(\phi(\hat{F}, \tau)) - F(\phi(\hat{F}, \tau))].$$

We have proved that  $\sup_y |\hat{F} - F| = o_P(1)$ , e.g., Lemma F.1. By the continuous mapping theorem  $\sup_\tau |\phi(F, \tau) - \phi(F, \tau)| = o_P(1)$ . Hence  $1/\dot{F}(\tilde{q}_\tau) < C$  uniformly in  $\tau$ . This implies  $|\phi(\hat{F}, \tau) - \phi(F, \tau)| \leq C|\Delta_F(\phi(\hat{F}, \tau))|$  where

$$\Delta_F(y) := \hat{F}(y) - F(y).$$

Applying the second-order mean value theorem to the left hand side of (G.2), there is  $c_\tau$  so that, for  $q(\tau) := \phi(F, \tau)$ ,

$$\dot{F}(q(\tau))(\phi(\hat{F}, \tau) - q(\tau)) + \frac{1}{2} \frac{d^2 F(c_\tau)}{dy} (\phi(\hat{F}, \tau) - q(\tau))^2 = -[\hat{F}(\phi(\hat{F}, \tau)) - F(\phi(\hat{F}, \tau))].$$

Rearranging and applying  $|\phi(\hat{F}, \tau) - \phi(F, \tau)| \leq C|\Delta_F(\phi(\hat{F}, \tau))|$ , we have

$$\begin{aligned} \phi(\hat{F}, \tau) - q(\tau) &= \frac{-1}{\dot{F}(q(\tau))} \Delta_F(\phi(\hat{F}, \tau)) + M_1(\tau) \\ &= \frac{-1}{\dot{F}(q(\tau))} \Delta_F(q(\tau)) + M_1(\tau) + M_2(\tau) \\ M_1(\tau) &\leq C \Delta_F(\phi(\hat{F}, \tau))^2 \leq C |\Delta_F(\phi(\hat{F}, \tau)) - \Delta_F(q(\tau))|^2 + C \Delta_F(q(\tau))^2 \\ M_2(\tau) &= -\frac{\Delta_F(\phi(\hat{F}, \tau)) - \Delta_F(q(\tau))}{\dot{F}(q(\tau))} \leq C |\Delta_F(\phi(\hat{F}, \tau)) - \Delta_F(q(\tau))|. \end{aligned} \tag{G.3}$$

Apply Lemma F.1, with  $\vartheta^g(y) = \mathbb{E}_t \Lambda(h_{it}(\mathbf{x}_{it})' \beta_i^g(y))$ . We have, for all  $F \in \{F_t, G_t\}$ ,

$$\Delta_F(y) = \frac{1}{N} \sum_i \left[ \frac{1}{\sqrt{T}} d_{\psi,i}(y) + d_{\gamma,i}(y) \right] + o_P(z(y))$$

where  $z(y) = \frac{1}{\sqrt{NT}} + \frac{1}{\sqrt{N}} \text{Var}_t(d_{\gamma,i}(y))^{1/2}$ . By Lemma G.2,  $\frac{1}{\sqrt{N}} \sum_i d_{\psi,i}(y)$

and  $\text{Var}_t(d_{\gamma,i}(y))^{-1/2} \frac{1}{\sqrt{N}} \sum_i d_{\gamma,i}(y)$  are stochastically equicontinuous in  $\ell^\infty(\mathcal{Y})$ . Then for  $q(\tau) = \phi(F, \tau)$ ,  $\hat{q}(\tau) = \phi(\hat{F}, \tau)$ ,  $V_F(y) := \text{Var}_t(d_{\gamma,i}(y))$ ,

$$\begin{aligned} |\Delta_F(\phi(\hat{F}, \tau)) - \Delta_F(q(\tau))| &\leq \frac{1}{\sqrt{NT}} \left| \frac{1}{\sqrt{N}} \sum_i d_{\psi,i}(\hat{q}(\tau)) - d_{\psi,i}(q(\tau)) \right| \\ &\quad + \frac{1}{\sqrt{N}} \left| \frac{1}{\sqrt{N}} \sum_i d_{\gamma,i}(\hat{q}(\tau)) - d_{\gamma,i}(q(\tau)) \right| + o_P(z(q(\tau))) \\ &= \frac{V_F(\hat{q}(\tau))^{1/2}}{\sqrt{N}} \left| V_F(\hat{q}(\tau))^{-1/2} \frac{1}{\sqrt{N}} \sum_i d_{\gamma,i}(\hat{q}(\tau)) - V_F(q(\tau))^{-1/2} \frac{1}{\sqrt{N}} \sum_i d_{\gamma,i}(q(\tau)) \right| \end{aligned}$$

$$\begin{aligned}
& + \frac{1}{\sqrt{N}} \left| V_F(\widehat{q}(\tau))^{1/2} V_F(q(\tau))^{-1/2} - 1 \right| \left| \frac{1}{\sqrt{N}} \sum_i d_{\gamma,i}(q(\tau)) \right| \\
& = o_P(z(q(\tau))) \\
& \quad M_1(\tau) + M_2(\tau) = o_P(z(q(\tau))).
\end{aligned}$$

The desired expansion then follows from (G.3). □

**Lemma G.2.**  $\frac{1}{\sqrt{N}} \sum_i d_{\psi,i}(y)$ , and  $\text{Var}_t(d_{\gamma,i}(y))^{-1/2} \frac{1}{\sqrt{N}} \sum_i d_{\gamma,i}(y)$  are asymptotically stochastically equicontinuous (ASE).

*Proof.* We show respectively that both  $\frac{1}{\sqrt{N}} \sum_i d_{\psi,i}(y)$ , and  $\text{Var}_t(d_{\gamma,i}(y))^{-1/2} \frac{1}{\sqrt{N}} \sum_i d_{\gamma,i}(y)$  are asymptotically tight under the metric  $\rho(y_1, y_2) = \bar{C}|y_1 - y_2|^{1/4}$  for some large  $\bar{C}$ .

(i) For any  $\eta, \delta > 0$ , by Assumption E.1,

$$\begin{aligned}
& \sum_i \mathbb{E} \sup_y |N^{-1/2} d_{\psi,i}(y)| 1\{\sup_y |N^{-1/2} d_{\psi,i}(y)| > \eta\} \\
& \leq \frac{1}{N\eta} \sum_i \mathbb{E} \sup_y |d_{\psi,i}(y)|^2 1\{\sup_y |d_{\psi,i}(y)| > \sqrt{N}\eta\} \\
& \leq C \sqrt{P(\sup_y |d_{\psi,i}(y)|^2 > N\eta^2)} \leq \frac{C}{N} \sqrt{\mathbb{E} \sup_y |d_{\psi,i}(y)|^2} = o(1). \\
& \frac{1}{N} \sum_i \mathbb{E} |d_{\psi,i}(y_1) - d_{\psi,i}(y_2)|^2 \leq C|y_1 - y_2|^{1/2}. \\
& \sup_{\eta > 0} \sum_i \eta^2 P \left( \sup_{\rho(y_1, y_2) < \delta} |d_{\psi,i}(y_1) - d_{\psi,i}(y_2)| > \sqrt{N}\eta \right) \leq \mathbb{E} \left( \sup_{\rho(y_1, y_2) < \delta} |d_{\psi,i}(y_1) - d_{\psi,i}(y_2)|^2 \right) \\
& \leq \delta^2.
\end{aligned}$$

Hence all conditions of Theorem 2.11.11 in van der Vaart and Wellner (1996) are verified. This implies the ASE of  $\frac{1}{\sqrt{N}} \sum_i d_{\psi,i}(y)$ .

(ii) Write  $v(y) = \text{Var}_t(d_{\gamma,i}(y))^{1/2}$ . Suppose  $v(y_1) \geq v(y_2)$ . Still by Assumption E.1,

$$\begin{aligned}
& \sum_i \mathbb{E} \sup_y |N^{-1/2} v(y)^{-1} d_{\gamma,i}(y)| 1\{\sup_y |N^{-1/2} v(y)^{-1} d_{\gamma,i}(y)| > \eta\} \\
& \leq \frac{1}{N\eta} \sum_i \mathbb{E} \sup_y \left[ \frac{|d_{\gamma,i}(y)|}{v(y)} \right]^2 1\{\sup_y v(y)^{-1} |d_{\gamma,i}(y)| > \sqrt{N}\eta\} \\
& \leq \frac{C}{N} \sqrt{\mathbb{E} \sup_y \left[ \frac{|d_{\gamma,i}(y)|}{v(y)} \right]^2} = o(1). \\
& \frac{1}{N} \sum_i \mathbb{E} |v(y_1)^{-1} d_{\gamma,i}(y_1) - v(y_2)^{-1} d_{\gamma,i}(y_2)|^2 \leq \mathbb{E} \frac{|d_{\gamma,i}(y_1) - d_{\gamma,i}(y_2)|^2}{v(y_1)v(y_2)}
\end{aligned}$$

$$\begin{aligned}
& + \sqrt{\mathbb{E} \frac{|d_{\gamma,i}(y_2)|^4}{v^4(y_2)}} \sqrt{\mathbb{E} \frac{|v(y_1)^2 - v(y_2)^2|^2}{v(y_1)^2 v(y_2)^2}} \leq C |y_1 - y_2|^{1/2}. \\
& \sup_{\eta > 0} \sum_i \eta^2 P \left( \sup_{\rho(y_1, y_2) < \delta} |v(y_1)^{-1} d_{\gamma,i}(y_1) - v(y_2)^{-1} d_{\gamma,i}(y_2)| > \sqrt{N} \eta \right) \\
& \leq \mathbb{E} \left( \sup_{\rho(y_1, y_2) < \delta} |v(y_1)^{-1} d_{\gamma,i}(y_1) - v(y_2)^{-1} d_{\gamma,i}(y_2)|^2 \right) \\
& \leq \mathbb{E} \sup_{\rho(y_1, y_2) < \delta} \frac{|d_{\gamma,i}(y_1) - d_{\gamma,i}(y_2)|^2}{v(y_1) v(y_2)} + \sqrt{\mathbb{E} \sup_{\rho(y_1, y_2) < \delta} \frac{|d_{\gamma,i}(y_2)|^4}{v^4(y_2)}} \sqrt{\mathbb{E} \sup_{\rho(y_1, y_2) < \delta} \frac{|v(y_1)^2 - v(y_2)^2|^2}{v(y_1)^2 v(y_2)^2}} \\
& \leq \delta^2.
\end{aligned}$$

Hence all conditions of Theorem 2.11.11 in van der Vaart and Wellner (1996) are verified. This implies the ASE of  $\text{Var}_t(d_{\gamma,i}(y))^{-1/2} \frac{1}{\sqrt{N}} \sum_i d_{\gamma,i}(y)$ .

$$\begin{aligned}
& \mathbb{E} \sup_{\rho(y_1, y_2) < \delta} |d_{\psi,i}(y_1) - d_{\psi,i}(y_2)|^2 + \mathbb{E} \sup_{\rho(y_1, y_2) < \delta} \frac{|d_{\gamma,i}(y_1) - d_{\gamma,i}(y_2)|^2}{\sqrt{\bar{V}_\gamma(y_1) \bar{V}_\gamma(y_2)}} \leq \delta^2 \\
& \sup_{\rho(y_1, y_2) < \delta} |\bar{V}_\psi(y_1) - \bar{V}_\psi(y_2)|^2 + \sup_{\rho(y_1, y_2) < \delta} \frac{|\bar{V}_\gamma(y_1) - \bar{V}_\gamma(y_2)|^2}{\bar{V}_\gamma(y_1) \bar{V}_\gamma(y_2)} \leq \delta^2.
\end{aligned}$$

□

## APPENDIX H. PROOF OF THEOREM 5.4: BOOTSTRAP VALIDITY

**H.1. Bootstrap weak convergence.** Suppose a functional estimator, whose bootstrap version also has the following expansion:

$$\hat{\vartheta}^*(y) - \vartheta(y) = \frac{1}{N} \sum_{i=1}^N \left[ \frac{1}{\sqrt{T}} d_{\psi,i}^*(y) + d_{\gamma,i}^*(y) \right] + o_{P^*}(\zeta_{NT}(y)) \quad (\text{H.1})$$

where  $(d_{\psi,i}^*(y), d_{\gamma,i}^*(y))$  is an SRS with replacement from  $(d_{\psi,i}(y), d_{\gamma,i}(y))$ .

**Proposition H.1.** *Suppose  $\hat{\vartheta}$  satisfies conditions in Proposition E.1. We have*

(i)

$$\frac{\hat{\vartheta}^*(\cdot) - \hat{\vartheta}(\cdot)}{s_{NT}(\cdot)} \Rightarrow^* \mathbb{G}(\cdot),$$

where  $s_{NT}^2(y) = \frac{1}{NT} \text{Var}_t(d_{\psi,i}) + \frac{1}{N} \text{Var}_t(d_{\gamma,i})$ , and  $\mathbb{G}(\cdot)$  is a centered Gaussian process with covariance kernel

$$H(y_k, y_l) = \lim_T \frac{\sigma_T^2(y_k, y_l)}{\sigma_T(y_k) \sigma_T(y_l)}.$$

(ii) For the same  $\mathbb{G}$ ,

$$\frac{\widehat{\vartheta}^*(\cdot) - \widehat{\vartheta}(\cdot)}{\widehat{s}^*(\cdot)} \Rightarrow^* \mathbb{G}(\cdot)$$

where  $\widehat{s}^*$  is the interquartile range of  $\widehat{\vartheta}^*(\cdot) - \widehat{\vartheta}(\cdot)$ , defined as

$$\widehat{s}^*(y) = \frac{q_{.75}^*(y) - q_{.25}^*(y)}{z_{.75} - z_{.25}};$$

here  $q_p^*(y)$  is the  $p$  th bootstrap quantile of  $\widehat{\vartheta}^*(y) - \widehat{\vartheta}(y)$  and  $z_p$  is the  $p$  th quantile of standard normal distribution.

(iii) Let  $q_\tau$  be the bootstrap quantile of  $\sup_y |\widehat{\vartheta}^*(y) - \widehat{\vartheta}(y)|/\widehat{s}^*(y)$ . Uniformly for  $P \in \mathcal{P}$ ,

$$P(|\widehat{\vartheta}(y) - \vartheta(y)| \leq q_\tau \widehat{s}^*(y), \quad \forall y \in \mathcal{Y}) \rightarrow 1 - \tau.$$

*Proof.* (i) Comparing the expansions of  $\widehat{\vartheta}^*$  with  $\widehat{\vartheta}$ , we have

$$\widehat{\vartheta}^*(y) - \widehat{\vartheta}(y) = \sum_{i=1}^N [\alpha_i^*(y) - \mathbb{E}^* \alpha_i^*(y)] + o_{P^*}(\zeta_{NT}(y))$$

where  $\alpha_i^*(y) = \frac{1}{N} \frac{1}{\sqrt{T}} d_{\psi,i}^*(y) + \frac{1}{N} d_{\gamma,i}(y)$ . Below we prove the weak convergence of  $\sum_i [\alpha_i^* - \mathbb{E}^* \alpha_i^*]/s_{NT}$ , where  $s_{NT} = \frac{1}{NT} \text{Var}_t(d_{\psi,i}) + \frac{1}{N} \text{Var}_t(d_{\gamma,i})$ .

(i) show the fidi. For any finite integer  $M > 0$ , and any  $y_1, \dots, y_M$ . Let  $A_i^* = ((\alpha_i^*(y_1) - \mathbb{E}^* \alpha_i^*(y_1))/s_{NT}(y_1), \dots, ((\alpha_i^*(y_M) - \mathbb{E}^* \alpha_i^*(y_M))/s_{NT}(y_M)))'$ . We shall show

$$\frac{g' \sum_i A_i^*}{\sqrt{g' H g}} \rightarrow^d \mathcal{N}(0, 1),$$

for any  $g \neq 0$  as an  $M$ -dimensional fixed vector. Note that  $\text{Var}^*(A_i^*) \rightarrow^P H$ . This implies  $\text{Var}^*(g' \sum_i A_i^*) - g' H g = o_P(g' H g)$ , given that  $\lambda_{\min}(H) > c > 0$ . Hence by the central limit theorem for i.i.d. data (the bootstrap data is i.i.d. since they are SRS draws with replacement),

$$\frac{g' \sum_i A_i^*}{\sqrt{g' H g}} = \frac{g' \sum_i A_i^*}{\sqrt{\text{Var}^*(g' \sum_i A_i^*)}} + o_{P^*}(1) \rightarrow^{d^*} \mathcal{N}(0, 1).$$

(ii) Let  $\ell^\infty(\mathcal{Y})$  be the set of all uniformly bounded real functions on  $\mathcal{Y}$ . We show the asymptotic tightness in  $\ell^\infty(\mathcal{Y})$ , by verifying the three conditions of Theorem 2.11.11 in van der Vaart and Wellner (1996). Let

$$\begin{aligned} b_i^*(y) &= \frac{\frac{1}{\sqrt{T}} d_{\psi,i}^*(y)}{\sigma_T(y)}, & c_i(y) &= \frac{d_{\gamma,i}^*(y)}{\sigma_T(y)}. \\ \bar{b}_i(y) &= \frac{\frac{1}{\sqrt{T}} d_{\psi,i}^*(y)}{[\frac{1}{T} \bar{V}_\psi(y)]^{1/2}}, & \bar{c}_i(y) &= \frac{d_{\gamma,i}^*(y)}{\bar{V}_\gamma(y)^{1/2}}. \end{aligned} \tag{H.2}$$

Let  $F_i^*(y) = \frac{\alpha_i^*}{s_{NT}} = \frac{1}{\sqrt{N}}(b_i^*(y) + c_i^*(y))$ . Define  $\rho(y_1, y_2) = C|y_1 - y_2|^{1/4}/\sqrt{\epsilon}$  for some  $C > 0$  and an arbitrarily small  $\epsilon > 0$ . Also recall the definition of  $b_i, c_i, \bar{b}_i, \bar{c}_i$  in (E.3).

Condition (1). For every  $\eta > 0$ , and an arbitrarily small  $a > 0$ ,

$$\begin{aligned}
 & \sum_i \mathbb{E}^* \sup_y |F_i^*(y)| 1\{\sup_y |F_i^*(y)| > \eta\} \\
 & \leq \eta^{-1} \frac{1}{N} \sum_i \sup_y |b_i(y) + c_i(y)|^2 1\{\sup_y |b_i(y) + c_i(y)| > \sqrt{N}\eta\} \\
 & \leq \frac{C}{\eta^{a+1}N^{a/2}} \frac{1}{N} \sum_i \sup_y |\bar{b}_i(y)|^{2+a} + \frac{1}{\eta^{a+1}N^{a/2}} \frac{1}{N} \sum_i \sup_y |\bar{c}_i(y)|^{2+a} \\
 & = O_P(1) \frac{C}{\eta^{a+1}N^{a/2}} \mathbb{E} \sup_y |\bar{b}_i(y)|^{2+a} + O_P(1) \frac{1}{\eta^{a+1}N^{a/2}} \mathbb{E} \sup_y |\bar{c}_i(y)|^{2+a} = o_P(1).
 \end{aligned}$$

Condition (2): For every  $y_1, y_2 \in \mathcal{Y}$ , and every  $\epsilon > 0$ , with probability at least  $1 - \epsilon$ ,  $\frac{1}{N} \sum_i |F_i(y_1) - F_i(y_2)|^2 \leq \frac{1}{N} \sum_i \mathbb{E} |F_i(y_1) - F_i(y_2)|^2 / \epsilon$ . On this event,

$$\begin{aligned}
 & \sum_i \mathbb{E}^* |F_i^*(y_1) - F_i^*(y_2)|^2 = \sum_i |F_i(y_1) - F_i(y_2)|^2 \\
 & \leq \sum_i \mathbb{E} |F_i(y_1) - F_i(y_2)|^2 / \epsilon \leq C \mathbb{E} |b_i(y_1) - b_i(y_2)|^2 / \epsilon + C \mathbb{E} |c_i(y_1) - c_i(y_2)|^2 / \epsilon \\
 & \leq C \mathbb{E} [d_{\psi,i}(y_1) - d_{\psi,i}(y_2)]^2 / \epsilon + C |\bar{V}_\psi(y_1) - \bar{V}_\psi(y_2)|^2 / \epsilon + C \frac{|\bar{V}_\gamma(y_1) - \bar{V}_\gamma(y_2)|^2}{\bar{V}_\gamma(y_1)\bar{V}_\gamma(y_2)} / \epsilon \\
 & \quad + \frac{\mathbb{E} |d_{\gamma,i}(y_1) - d_{\gamma,i}(y_2)|^2}{\sqrt{\bar{V}_\gamma(y_1)\bar{V}_\gamma(y_2)}} / \epsilon \leq C |y_1 - y_2|^{1/2} / \epsilon \leq \rho(y_1, y_2)^2.
 \end{aligned}$$

Condition (3): For every  $\delta > 0$ , on the event  $\sum_i (\sup_{\rho(y_1, y_2) < \delta} |F_i(y_1) - F_i(y_2)|^2) \leq \sum_i \mathbb{E} (\sup_{\rho(y_1, y_2) < \delta} |F_i(y_1) - F_i(y_2)|^2) / \epsilon$ ,

$$\begin{aligned}
 & \sup_{\eta > 0} \sum_i \eta^2 P^* \left( \sup_{\rho(y_1, y_2) < \delta} |F_i(y_1) - F_i(y_2)| > \eta \right) \leq \sum_i \mathbb{E}^* \left( \sup_{\rho(y_1, y_2) < \delta} |F_i(y_1) - F_i(y_2)|^2 \right) \\
 & = \sum_i \left( \sup_{\rho(y_1, y_2) < \delta} |F_i(y_1) - F_i(y_2)|^2 \right) \leq \sum_i \mathbb{E} \left( \sup_{\rho(y_1, y_2) < \delta} |F_i(y_1) - F_i(y_2)|^2 \right) / \epsilon \\
 & \leq \frac{1}{N} \sum_i \mathbb{E} \left( \sup_{\rho(y_1, y_2) < \delta} |b_i(y_1) - b_i(y_2)|^2 \right) / \epsilon + \frac{1}{N} \sum_i \mathbb{E} \left( \sup_{\rho(y_1, y_2) < \delta} |c_i(y_1) - c_i(y_2)|^2 \right) / \epsilon \\
 & \leq \delta^2.
 \end{aligned} \tag{H.3}$$

Thus all conditions are satisfied. Together, the process  $\sum_i [\alpha_i^*(\cdot) - \mathbb{E}^* \alpha_i^*(\cdot)] / s_{NT}(\cdot)$  weakly converges to a centered Gaussian process, with covariance kernel

$$H(y_k, y_l) = \lim_T \frac{\sigma_T^2(y_k, y_l)}{\sigma_T(y_k)\sigma_T(y_l)}.$$

Hence uniformly in  $y$ ,

$$\mathbb{Z}_{NT}^*(y) := \frac{\widehat{\vartheta}^*(y) - \widehat{\vartheta}(y)}{s_{NT}(y)} = \frac{\sum_i [\alpha_i^*(y) - \mathbb{E}^* \alpha_i^*(y)]}{s_{NT}(y)} + o_{P^*}(1) \Rightarrow \mathbb{G}$$

This implies the weak convergence .

(ii) The interquartile range is defined as

$$\widetilde{s}^*(y) = \frac{q_{.75}^*(y) - q_{.25}^*(y)}{z_{.75} - z_{.25}},$$

where  $q_p^*(y)$  is the  $p$  th bootstrap quantile of  $\widehat{\vartheta}^*(y) - \widehat{\vartheta}(y)$  and  $z_p$  is the  $p$  th quantile of standard normal distribution. It suffices to prove

$$\sup_y \left| \frac{s_{NT}}{\widetilde{s}^*} - 1 \right| = o_P(1). \quad (\text{H.4})$$

To see this, note that  $P^*(\mathbb{Z}_{NT}^*(y) < v) \rightarrow^P P(\mathbb{G}(y) < v)$  uniformly in  $(y, v) \in \mathcal{Y} \times \mathbb{R}$ . Let  $\kappa_p(y)$  be the  $p$  th bootstrap quantile of  $\mathbb{Z}_{NT}^*(y)$ . Note that the covariance kernel of  $\mathbb{G}(y)$  satisfies  $H(y, y) = 1$ , so  $\mathbb{G}(y)$  is standard normal for any give  $y$ . Thus  $\kappa_p(y) \rightarrow^P z_p$  uniformly in  $y$ . Recall that  $q_p^*(y)$  is the  $p$  th bootstrap quantile of  $\widehat{\vartheta}^*(y) - \widehat{\vartheta}(y) = s_{NT}(y)\mathbb{Z}_{NT}^*(y)$ , we have  $q_p^*(y) = s_{NT}(y)\kappa_p(y)$ . Let  $\Delta q^*(y) = q_{.75}^*(y) - q_{.25}^*(y)$ ; similarly define  $\Delta \kappa(y)$  and  $\Delta z$ . We have  $\Delta q^*(y) = s_{NT}(y)\Delta \kappa(y)$ . Therefore

$$\frac{\widetilde{s}^*(y)}{s_{NT}(y)} - 1 = \frac{\Delta q^*(y)/\Delta z - s_{NT}(y)}{s_{NT}(y)} = \frac{\Delta \kappa(y)}{\Delta z} - 1 = \frac{\kappa_{.75} - z_{.75}}{\Delta z} - \frac{\kappa_{.25} - z_{.25}}{\Delta z},$$

which converges to zero in probability uniformly in  $y$ . This also implies (H.4).

(iii) Let

$$\begin{aligned} A &:= \sup_y \left| \frac{\widehat{\vartheta}(y) - \vartheta(y)}{s_{NT}(y)} \right|, \quad B := \sup_y \left| \frac{\widehat{\vartheta}(y) - \vartheta(y)}{\widetilde{s}^*(y)} \right| \\ \text{CI}(y) &:= \left\{ a : |\widehat{\vartheta}(y) - a| \leq q_\tau \widetilde{s}^*(y) \right\}. \end{aligned}$$

By Proposition E.1 and the continuous mapping theorem,  $A \rightarrow^d \sup_y |\mathbb{G}(y)|$ . In addition, by (H.4)

$$|B - A| \leq A \sup_y \left| \frac{s_{NT}}{\widetilde{s}^*} \left( 1 - \frac{\widetilde{s}^*}{s_{NT}} \right) \right| = o_P(1),$$

implying  $B \rightarrow^d \sup_y |\mathbb{G}(y)|$ . Next, by part (ii) of the proposition,

$$C := \sup_y \left| \frac{\widehat{\vartheta}^*(y) - \widehat{\vartheta}(y)}{\widetilde{s}^*} \right| \rightarrow^{d^*} \sup_y |\mathbb{G}(y)|.$$

Therefore for the event:  $E := \{\vartheta(y) \in \text{Cl}_\tau(y), \forall y\}$ , we have

$$P(E) = P(B \leq q_\tau) \rightarrow P^*(C \leq q_\tau) = 1 - \tau.$$

Now consider a DGP sequence  $\{P_T : T \geq 1\} \subset \mathcal{P}$  and its subsequence  $\{P_{T_k} : k \geq 1\}$  so that

$$\limsup_T \sup_{P \in \mathcal{P}} |P(E) - (1 - \tau)| = \limsup_T |P_T(E) - (1 - \tau)| = \lim_k |P_{T_k}(E) - (1 - \tau)|.$$

Note that  $\{P_{T_k} : k \geq 1\} \subset \mathcal{P}$  so the probability measure  $P_{T_k}$  satisfies the conditions of this proposition. It implies  $\lim_k P_{T_k}(E) \rightarrow 1 - \tau$ . Hence

$$\limsup_T \sup_{P \in \mathcal{P}} |P(E) - (1 - \tau)| = 0.$$

□

## H.2. Proof of Theorem 5.4 (i): coverage of $\theta(y)$ .

*Proof.* The expansion of Lemma D.3 still holds:

$$\hat{\beta}_i^* - \beta_i^* = -\mathbb{A}_{1i}^* \frac{1}{T} \sum_t \psi_{it}(y)^* + R_{i,9}^* + 2R_{i,4}^* + 2R_{i,5}^* - \bar{R}_{i,4}^* - \bar{R}_{i,5}^*$$

where the  $*$  variables are defined as a cross-sectional random sample with replacement. Define, for  $P_W^* = W^*(W^{*'}W^*)^{-1}W^{*'}$ ,

$$\hat{\theta}^*(y) = \frac{1}{N} \sum_{i=1}^N \hat{\beta}_i^*(y) \mathbf{w}_i^{*'} S_{wz,N}^*, \quad S_{wz,N}^* := \left( \frac{1}{N} W^{*'} W^* \right)^{-1} W^{*'} Z^* (Z^{*'} P_W^* Z^*)^{-1}.$$

Also note that  $\beta_i^* = \theta \mathbf{w}_i^* + \gamma_i^*$ . Then similar to (E.7), by Lemmas H.1 and H.2,

$$\begin{aligned} \hat{\theta}^*(y) - \theta(y) &= \frac{1}{NT} \sum_{i=1}^N \sum_{t=1}^T \mathbb{A}_{1i}^*(y) \psi_{y,it}^* \mathbf{w}_i^{*'} S_{wz,N}^* + \frac{1}{N} \sum_{i=1}^N \gamma_i^*(y) \mathbf{w}_i^{*'} S_{wz,N}^* \\ &\quad + \frac{1}{N} \sum_{i=1}^N R_{i,9}^* \mathbf{w}_i^{*'} S_{wz,N}^* + \frac{1}{N} \sum_{i=1}^N [2R_{i,4}^* + 2R_{i,5}^* - \bar{R}_{i,4}^* - \bar{R}_{i,5}^*] \mathbf{w}_i^{*'} S_{wz,N}^* \\ &= \frac{1}{NT} \sum_{i=1}^N \sum_{t=1}^T \mathbb{A}_{1i}^*(y) \psi_{it}(y)^* \mathbf{w}_i^{*'} S_{wz,N}^* + \frac{1}{N} \sum_{i=1}^N \gamma_i^*(y) \mathbf{w}_i^{*'} S_{wz,N}^* + o_{P^*} \left( \frac{1}{\sqrt{NT}} \right) \\ &= \frac{1}{NT} \sum_{i=1}^N \sum_{t=1}^T \mathbb{A}_{1i}^*(y) \psi_{it}(y)^* \mathbf{w}_i^{*'} S_{wz} + \frac{1}{N} \sum_{i=1}^N \gamma_i^*(y) \mathbf{w}_i^{*'} S_{wz} + o_{P^*}(\zeta_{NT}(y)) \\ &= \frac{1}{NT} \sum_{i=1}^N \left[ \frac{1}{\sqrt{T}} d_{\psi,i}^*(y) + d_{\gamma,i}^*(y) \right] + o_{P^*}(\zeta_{NT}(y)). \end{aligned} \tag{H.5}$$

Hence expansion (H.1) holds. This leads to the desired result, following from Proposition H.1.  $\square$

**Lemma H.1.** *For the cross sectional bootstrap, uniformly in  $y \in \mathcal{Y}$ ,  $\frac{1}{N} \sum_i \|R_{i8}^*\|^2 = O_{P^*}(T^{-3})$ ,  $\frac{1}{N} \sum_i R_{i,4}^* \mathbf{w}_i^{*'} = O_{P^*}(\frac{1}{T\sqrt{N}})$ , and  $\frac{1}{N} \sum_i \bar{R}_{i,4}^* \mathbf{w}_i^{*'} = O_{P^*}(\frac{1}{T\sqrt{N}})$ . Also,  $\frac{1}{N} \sum_i R_{i,5}^* \mathbf{w}_i^{*'} = O_{P^*}(\frac{1}{T\sqrt{N}})$ , and  $\frac{1}{N} \sum_i \bar{R}_{i,5}^* \mathbf{w}_i^{*'} = O_{P^*}(\frac{1}{T\sqrt{N}})$ .*

*Proof.* First of all, the same proof of Lemma D.4, D.3 in the bootstrap world still holds. So it is easy to claim  $\frac{1}{N} \sum_i \|R_{i8}^*\|^2 = O_{P^*}(T^{-3})$ . The proof is similar to that of Lemma E.1, with a slight modification.

(i) For  $\frac{1}{N} \sum_i R_{i,4}^* \mathbf{w}_i^{*'}$ , we define  $b_i^*(y) = \frac{1}{2} \mathbb{A}_{1i}^* \mathbb{A}_{2i}^* (\mathbb{A}_{1i}^* \otimes \mathbb{A}_{1i}^*)$  and

$$a_i^*(y) = T \nabla Q_i^*(\beta_i) \otimes \nabla Q_i^*(\beta_i) - T(\mathbb{E}[\nabla Q_i(\beta_i) \otimes \nabla Q_i(\beta_i)])^*.$$

Again, the star variable means a cross-sectional random sample from  $i = 1, \dots, N$ . Also, let  $F_i^*(y) = -\frac{1}{\sqrt{N}} a_i^*(y) b_i^*(y) \mathbf{w}_i^*$ . Now  $\mathbb{E}^* F_i^*(y) = \sum_i F_i(y)$ . Hence

$$\frac{T\sqrt{N}}{N} \sum_i R_{i,4}^* \mathbf{w}_i^* = \sum_i F_i^*(y) = \sum_i [F_i^*(y) - \mathbb{E}^* F_i^*(y)] + \sum_i F_i(y).$$

The proof of Lemma E.1 shows  $\sup_y \|\sum_i F_i(y)\| = O_P(1)$ . It remains to prove  $\sum_i [F_i^*(y) - \mathbb{E}^* F_i^*(y)]$  is asymptotically tight. The proof is mimicking that of Lemma E.1 in the bootstrap world, so we are briefly outlying it here.

For Condition (1) of Theorem 2.11.11 in van der Vaart and Wellner (1996),

$$\begin{aligned} & \sum_i \mathbb{E}^* \sup_y |F_i^*(y)| 1\{\sup_y |F_i^*(y)| > \eta\} \leq \frac{1}{\eta^{a+1} N^{a/2}} \mathbb{E}^* \sup_y |a_i^*(y) b_i^*(y) \mathbf{w}_i^*|^{2+a} \\ & \leq O_P\left(\frac{1}{\eta^{a+1} N^{a/2}}\right) \frac{1}{N} \sum_i \mathbb{E} \sup_y |a_i(y) b_i(y) \mathbf{w}_i|^{2+a} \leq O_P(1). \end{aligned}$$

The bound  $\frac{1}{N} \sum_i \mathbb{E} \sup_y |a_i(y)|^m < C$  follows from the proof of Lemma E.1.

Condition (2): Take  $y_1, y_2 \in \mathcal{Y}$ . For an arbitrarily small  $\epsilon > 0$ , with probability at least  $1 - \epsilon$ ,  $\sum_i |F_i(y_1) - F_i(y_2)|^2 \leq \sum_i \mathbb{E} |F_i(y_1) - F_i(y_2)|^2 / \epsilon$ . On this event,

$$\begin{aligned} & \sum_i \mathbb{E}^* |F_i^*(y_1) - F_i^*(y_2)|^2 = \sum_i |F_i(y_1) - F_i(y_2)|^2 \leq \sum_i \mathbb{E} |F_i(y_1) - F_i(y_2)|^2 / \epsilon \\ & \leq C \frac{1}{N} \sum_i (\mathbb{E} |a_i(y_1) - a_i(y_2)|^4)^{1/2} / \epsilon + C \frac{1}{N} \sum_i |b_i(y_1) - b_i(y_2)|^2 / \epsilon \\ & \leq C |y_1 - y_2|^{1/2} / \epsilon \leq \rho(y_1, y_2)^2, \end{aligned}$$

where  $\rho(y_1, y_2) = \bar{C} |y_1 - y_2|^{1/4} / \sqrt{\epsilon}$  for sufficiently large  $\bar{C}$ .

Condition (3): For every  $\epsilon > 0$ , with probability at least  $1 - \epsilon$ ,  $\sum_i (\sup_{\rho(y_1, y_2) < \delta} |F_i(y_1) - F_i(y_2)|^2) \leq \sum_i \mathbb{E} (\sup_{\rho(y_1, y_2) < \delta} |F_i(y_1) - F_i(y_2)|^2) / \epsilon$ . On this event, for every  $\delta > 0$ ,

$$\begin{aligned}
 & \sup_{\eta > 0} \sum_i \eta^2 P^* \left( \sup_{\rho(y_1, y_2) < \delta} |F_i^*(y_1) - F_i^*(y_2)| > \eta \right) \\
 & \leq \sum_i \mathbb{E}^* \left( \sup_{\rho(y_1, y_2) < \delta} |F_i^*(y_1) - F_i^*(y_2)|^2 \right) = \sum_i \left( \sup_{\rho(y_1, y_2) < \delta} |F_i(y_1) - F_i(y_2)|^2 \right) \\
 & \leq \frac{1}{N} \sum_i \mathbb{E} \left( \sup_{\rho(y_1, y_2) < \delta} |a_i(y_1)b_i(y_1) - a_i(y_2)b_i(y_2)|^2 \|\mathbf{w}_i\|^2 \right) / \epsilon \\
 & \leq C \frac{1}{N} \sum_i (\mathbb{E} \sup_{|y_1 - y_2| < (\delta/\bar{C})^4 \epsilon^2} |a_i(y_1) - a_i(y_2)|^4)^{1/2} / \epsilon + C \frac{1}{N} \sum_i \sup_{|y_1 - y_2| < (\delta/\bar{C})^4 \epsilon^2} |b_i(y_1) - b_i(y_2)|^2 / \epsilon \\
 & \leq \delta^2 \frac{C\epsilon}{\bar{C}^2 \epsilon} < \delta^2
 \end{aligned}$$

by choosing a sufficiently large  $\bar{C}$  in the definition of  $\rho$ . Hence all sufficient conditions of Theorem 2.11.11 in van der Vaart and Wellner (1996) are verified. Thus  $\sum_i [F_i^*(y) - \mathbb{E}^* F_i^*(y)]$  is asymptotically tight.

(ii) For  $\frac{1}{N} \sum_i R_{i,5}^* \mathbf{w}_i^{*'}$ , similar to Lemma E.1, we show  $\sup_y \|\sum_i F_i^*(y)\| = O_{P^*}(1)$  where

$$F_i^*(y) = \frac{T}{\sqrt{N}} \mathbb{A}_{1i}^* [A_{1i}^{*-1} - \mathbb{A}_{1i}^{*-1}] \mathbb{A}_{1i}^* \nabla Q_i^*(\beta_i^*) \mathbf{w}_i^* - \frac{T}{\sqrt{N}} (\mathbb{E} \mathbb{A}_{1i} [A_{1i}^{-1} - \mathbb{A}_{1i}^{-1}] \mathbb{A}_{1i} \nabla Q_i(\beta_i) \mathbf{w}_i)^*.$$

By Lemma E.1,

$$\mathbb{E}^* \sum_i F_i^*(y) = \frac{T}{\sqrt{N}} \sum_i \mathbb{A}_{1i} [A_{1i}^{-1} - \mathbb{A}_{1i}^{-1}] \mathbb{A}_{1i} \nabla Q_i(\beta_i) \mathbf{w}_i - \mathbb{E} (\mathbb{A}_{1i} [A_{1i}^{-1} - \mathbb{A}_{1i}^{-1}] \mathbb{A}_{1i} \nabla Q_i(\beta_i) \mathbf{w}_i)$$

is asymptotically tight. Hence it remains to show  $\sum_i (\mathbf{z}_i^*(y) - \mathbb{E}^* \mathbf{z}_i^*(y))$  is asymptotically tight by verifying the conditions of Theorem 2.11.11 in van der Vaart and Wellner (1996).

Condition (1): for every  $\eta > 0$ , fix  $0 < a < 2$ ,

$$\begin{aligned}
 & \sum_i \mathbb{E}^* \sup_y |F_i^*(y)| 1\{\sup_y |F_i^*(y)| > \eta\} = \sum_i \sup_y |F_i(y)| 1\{\sup_y |F_i(y)| > \eta\} \\
 & \leq O_P\left(\frac{C}{\eta^{a+1} N^{a/2}}\right) \frac{1}{N} \sum_i [\mathbb{E} \sup_y |\sqrt{T}(\mathbb{A}_{1i}^{-1} - A_{1i}^{-1})|^{4+2a}]^{1/2} [\mathbb{E} \sup_y |\sqrt{T} \nabla Q_i(\beta_i)|^{8+4a}]^{1/4} \\
 & \leq o_P(1).
 \end{aligned}$$

Condition (2). Define  $a_i(y) = \sqrt{T} \mathbb{A}_{1i} [A_{1i}^{-1} - \mathbb{A}_{1i}^{-1}] \mathbb{A}_{1i}$ ,  $b_i(y) = \sqrt{T} \nabla Q_i(\beta_i)$  and  $c_i(y) = \sqrt{T} [A_{1i}^{-1}(y) - \mathbb{A}_{1i}^{-1}(y)]$ . With probability at least  $1 - \epsilon$ ,

$\sum_i |F_i(y_1) - F_i(y_2)|^2 \leq \mathbb{E} \sum_i |F_i(y_1) - F_i(y_2)|^2 / \epsilon$ . On this event,

$$\begin{aligned}
& \sum_i \mathbb{E}^* |F_i^*(y_1) - F_i^*(y_2)|^2 \\
&= \sum_i |F_i(y_1) - F_i(y_2)|^2 \leq \sum_i \mathbb{E} |F_i(y_1) - F_i(y_2)|^2 / \epsilon \\
&\leq C \frac{1}{N} \sum_i [\mathbb{E} \|a_i(y_1) - a_i(y_2)\|^4]^{1/2} / \epsilon + C \frac{1}{N} \sum_i [\mathbb{E} \|b_i(y_1) - b_i(y_2)\|^4]^{1/2} / \epsilon \\
&\leq C |y_1 - y_2|^2 / \epsilon + [\frac{1}{N} \sum_i \mathbb{E} \|c_i(y_1) - c_i(y_2)\|^4]^{1/2} / \epsilon + C |y_1 - y_2|^{1/2} / \epsilon \\
&\leq C |y_1 - y_2|^{1/2} / \epsilon \leq \rho(y_1, y_2)^2.
\end{aligned}$$

Condition (3): Define

$$M := \frac{1}{N} \sum_i \left( \sup_{\rho(y_1, y_2) < \delta} |a_i(y_1)b_i(y_1) - a_i(y_2)b_i(y_2)|^2 \|\mathbf{w}_i\|^2 \right).$$

For every  $\epsilon > 0$ , with probability at least  $1 - \epsilon$ ,  $M \leq \mathbb{E}M / \epsilon$ . On this event, for every  $\delta > 0$ , and sufficiently large  $\bar{C}$ , recall  $\rho(y_1, y_2) = \bar{C}|y_1 - y_2|^{1/4} / \sqrt{\epsilon}$ .

$$\begin{aligned}
& \sup_{\eta > 0} \sum_i \eta^2 P^* \left( \sup_{\rho(y_1, y_2) < \delta} |F_i^*(y_1) - F_i^*(y_2)| > \eta \right) \\
&\leq \frac{1}{N} \sum_i \mathbb{E}^* \left( \sup_{\rho(y_1, y_2) < \delta} |a_i^*(y_1)b_i^*(y_1) - a_i^*(y_2)b_i^*(y_2)|^2 \|w_i^*\|^2 \right) \\
&\quad + \frac{1}{N} \sum_i \mathbb{E}^* \left( \sup_{\rho(y_1, y_2) < \delta} |(\mathbb{E}a_i(y_1)b_i(y_1))^* - (\mathbb{E}a_i(y_2)b_i(y_2))^*|^2 \|w_i^*\|^2 \right) \\
&= M + \frac{1}{N} \sum_i \mathbb{E} \left( \sup_{\rho(y_1, y_2) < \delta} |\mathbb{E}a_i(y_1)b_i(y_1) - \mathbb{E}a_i(y_2)b_i(y_2)|^2 \|\mathbf{w}_i\|^2 \right) \\
&\leq \mathbb{E}M / \epsilon + \frac{1}{N} \sum_i \mathbb{E} \left( \sup_{\rho(y_1, y_2) < \delta} \mathbb{E} \|a_i(y_1) - a_i(y_2)\|^2 \|\mathbf{w}_i\|^2 \right) \sup_y \mathbb{E} \|b_i(y)\|^2 \\
&\quad + \frac{1}{N} \sum_i \mathbb{E} \left( \sup_{\rho(y_1, y_2) < \delta} \mathbb{E} \|b_i(y_1) - b_i(y_2)\|^2 \|\mathbf{w}_i\|^2 \right) \sup_y \mathbb{E} \|a_i(y)\|^2 \\
&\leq C \frac{1}{N} \sum_i (\mathbb{E} \sup_{|y_1 - y_2| < (\delta/\bar{C})^4 \epsilon^2} |a_i(y_1) - a_i(y_2)|^4)^{1/2} / \epsilon \\
&\quad + C \frac{1}{N} \sum_i (\mathbb{E} \sup_{|y_1 - y_2| < (\delta/\bar{C})^4 \epsilon^2} |b_i(y_1) - b_i(y_2)|^4)^{1/2} / \epsilon \\
&\quad + C \sup_{\mathbf{w}_i} \sup_{|y_1 - y_2| < (\delta/\bar{C})^4} [\mathbb{E} \|c_i(y_1) - c_i(y_2)\|^2 + \|b_i(y_1) - b_i(y_2)\|^2] \leq \delta^2.
\end{aligned}$$

The proof of  $\frac{1}{N} \sum_i \bar{R}_{i,5}^* w_i^*$  is the same.

□

**Lemma H.2.** Let  $\bar{V}_\gamma(y) = \mathbb{E}(\mathbf{w}_i \mathbf{w}_i') \otimes \mathbb{E}(\gamma_i(y) \gamma_i(y)' | \mathbf{w}_i)$ . Then

- (i)  $\sup_y \left\| \frac{1}{NT} \sum_{i=1}^N \sum_{t=1}^T \mathbb{A}_{1i}(y) \psi_{it}(y) \mathbf{w}_i' \right\| = O_P(\frac{1}{\sqrt{NT}})$ ,
- (ii)  $\sup_y \left\| \bar{V}_\gamma(y)^{-1/2} \text{vec}(\frac{1}{N} \sum_i \gamma_i(y) \mathbf{w}_i') \right\| = o_P(1)$ ,
- (iii)  $\frac{1}{N} \sum_{i=1}^N \frac{1}{T} \sum_{t=1}^T \mathbb{A}_{1i}^*(y) \psi_{it}(y)^* \mathbf{w}_i^{*'} (S_{wz,N}^* - S_{wz}) = o_{P^*}(\frac{1}{\sqrt{NT}})$ ,
- (iv)  $\frac{1}{N} \sum_{i=1}^N \gamma_i^*(y) \mathbf{w}_i^{*'} (S_{wz,N}^* - S_{wz}) = o_{P^*}(\frac{1}{\sqrt{N}} \|\bar{V}_\gamma(y)\|^{1/2})$ .

*Proof.* Let  $b_i(y) = \frac{1}{\sqrt{N}} \frac{1}{\sqrt{T}} \sum_{t=1}^T \mathbb{A}_{1i}(y) \psi_{it}(y) \mathbf{w}_i'$ ;  $b_i^*(y) = \frac{1}{\sqrt{N}} \frac{1}{\sqrt{T}} \sum_{t=1}^T \mathbb{A}_{1y,i}^* \psi_{it}^*(y) \mathbf{w}_i^{*'}$ . Also let  $c_i(y)$  be any component of  $\bar{V}_\gamma(y)^{-1/2} \text{vec}(\frac{1}{\sqrt{N}} \sum_i \gamma_i(y) \mathbf{w}_i')$ , and  $c_i^*(y)$  be any component of  $\bar{V}_\gamma(y)^{-1/2} \text{vec}(\frac{1}{\sqrt{N}} \sum_i \gamma_i^*(y) \mathbf{w}_i^{*'})$ . In addition, let  $F_{i,1}(y) = \frac{1}{\sqrt{N}} b_i(y)$ ,  $F_{i,1}^*(y) = \frac{1}{\sqrt{N}} b_i^*(y)$ ,  $F_{i,2}(y) = \frac{1}{\sqrt{N}} c_i(y)$ , and  $F_{i,2}^*(y) = \frac{1}{\sqrt{N}} c_i^*(y)$ .

Then, the same argument in part (ii) of the proof for Theorem 5.1 can be applied, to show that both  $\sum_i F_{i,1}(y)$  and  $\sum_i F_{i,2}(y)$  are asymptotically tight in  $\ell^\infty(\mathcal{Y})$ . This leads to (i) and (ii).

In addition, the same argument can be applied to show that both  $\sum_i F_{i,1}^*(y)$  and  $\sum_i F_{i,2}^*(y)$  are asymptotically tight. Hence  $\sup_y \left\| \frac{1}{NT} \sum_{i=1}^N \sum_{t=1}^T \mathbb{A}_{1y,i}^* \psi_{it}^*(y) \mathbf{w}_i^{*'} \right\| = O_{P^*}(\frac{1}{\sqrt{NT}})$ , and  $\sup_y \left\| \bar{V}_\gamma(y)^{-1/2} \text{vec}(\frac{1}{N} \sum_i \gamma_i^*(y) \mathbf{w}_i^{*'}) \right\| = o_{P^*}(1)$ . Finally,  $\|S_{wz,N}^* - S_{wz}\| = o_{P^*}(1)$ . This leads to (iii)(iv). □

### H.3. Proof of Theorem 5.4 (ii): coverage of cross-section distributions.

*Proof.* We first prove the expansion of  $\hat{G}_t$ . By (H.5),

$$\hat{\theta}^*(y) - \theta(y) = \frac{1}{NT} \sum_{i=1}^N \sum_{t=1}^T \mathbb{A}_{1i}^*(y) \psi_{it}(y)^* \mathbf{w}_i^{*'} S_{wz} + \frac{1}{N} \sum_{i=1}^N \gamma_i^*(y) \mathbf{w}_i^{*'} S_{wz} + o_{P^*}(\zeta_{NT}(y)).$$

Recall that  $\hat{\beta}_i^{g*}(y) = \hat{\beta}_i^*(y) + \hat{\theta}^*(y)[g^*(\mathbf{z}_i) - \mathbf{z}_i^*]$ . Similar to (F.1),

$$\begin{aligned} & \frac{1}{N} \sum_i \Lambda(-\mathbf{x}_{it}^{*'} \hat{\beta}_i^{g*}(y)) - \frac{1}{N} \sum_i \Lambda(-\mathbf{x}_{it}^{*'} \beta_i^{g*}(y)) = D_0^* + \dots + D_3 + o_{P^*}(\zeta_{NT}) \\ D_0^* &:= -\frac{1}{N} \sum_i \dot{\Lambda}(-\mathbf{x}_{it}^{*'} \beta_i^{g*}(y)) \mathbf{x}_{it}^{*'} (\hat{\beta}_i^*(y) - \beta_i^*(y)) \\ &= -\frac{1}{NT} \sum_{it} \dot{\Lambda}(-\mathbf{x}_{it}^{*'} \beta_i^{g*}(y)) \mathbf{x}_{it}^{*'} \mathbb{A}_{1i}^* \psi_{it}^*(y) + o_{P^*}(\zeta_{NT}(y)) \\ D_1^* &:= \frac{1}{2N} \sum_i \text{tr} \left[ \ddot{\Lambda}(-\mathbf{x}_{it}^{*'} \beta_i^{g*}(y)) \mathbf{x}_{it}^* \mathbf{x}_{it}^{*'} (\hat{\beta}_i^*(y) - \beta_i^*(y)) (\hat{\beta}_i^*(y) - \beta_i^*(y))' \right] \\ &= \frac{1}{2NT} \sum_i \text{tr} \left[ \ddot{\Lambda}(-\mathbf{x}_{it}^{*'} \beta_i^{g*}(y)) \mathbf{x}_{it}^* \mathbf{x}_{it}^{*'} \hat{B}_i^*(y)^{-1} \right] + o_{P^*}(\zeta_{NT}(y)) \end{aligned}$$

$$\begin{aligned}
D_2^* &:= \text{tr}[\bar{G}(y)(\hat{\theta}^*(y) - \theta(y))] \\
&= \frac{1}{NT} \sum_{it} \mathbf{w}_i^{*'} S_{wz} \bar{G}(y) \mathbb{A}_{1i}^*(y) \psi_{it}^*(y) + \frac{1}{N} \sum_{i=1}^N \mathbf{w}_i^{*'} S_{wz} \bar{G}(y) \gamma_i^*(y) + o_{P^*}(\zeta_{NT}(y)) \\
D_3^* &:= \frac{1}{N} \sum_i (\hat{\beta}_i^*(y) - \beta_i^*(y))' \ddot{\Lambda}(-\mathbf{x}_{it}^{*'} \beta_i^{g*}(y)) \mathbf{x}_{it}^* \mathbf{x}_{it}^{*'} (\hat{\theta}^* - \theta) [g^*(\mathbf{z}_i) - \mathbf{z}_i^*] \\
&\quad + \frac{1}{2N} \sum_i \ddot{\Lambda}(-\mathbf{x}_{it}^{*'} \beta_i^{g*}(y)) [\mathbf{x}_{it}^{*'} (\hat{\theta}^* - \theta) (g^*(\mathbf{z}_i) - \mathbf{z}_i^*)]^2 = o_{P^*}(\zeta_{NT}(y)).
\end{aligned}$$

Recall that  $\Psi_{i,II}^*(y; \hat{\beta}_i^{g*}(y)) = \Lambda(-\mathbf{x}_{it}^{*'} \hat{\beta}_i^{g*}(y)) - \frac{1}{2T} \text{tr} \left( \ddot{\Lambda}(-\mathbf{x}_{it}^{*'} \beta_i^{g*}(y)) \mathbf{x}_{it}^* \mathbf{x}_{it}^{*'} \hat{B}_i^*(y)^{-1} \right)$ . Hence

$$\begin{aligned}
\hat{G}_t^*(y) &:= \frac{1}{N} \sum_i \Psi_{i,II}^*(y; \hat{\beta}_i^{g*}(y)) = \frac{1}{N} \sum_i \Lambda(-\mathbf{x}_{it}^{*'} \beta_i^{g*}(y)) + \frac{1}{N} \sum_{i=1}^N \mathbf{w}_i^{*'} S_{wz} \bar{G}(y) \gamma_i^*(y) \\
&\quad + \frac{1}{NT} \sum_{it} [\mathbf{w}_i^{*'} S_{wz} \bar{G}(y) - \dot{\Lambda}(-\mathbf{x}_{it}^{*'} \beta_i^{g*}(y)) \mathbf{x}_{it}^{*'}] \mathbb{A}_{1i}^*(y) \psi_{it}^*(y) + o_{P^*}(\zeta_{NT}(y)) \\
&= \frac{1}{N} \sum_i \frac{1}{\sqrt{T}} d_{\psi,i}^{II*}(y) + \frac{1}{N} \sum_i d_{\gamma,i}^{II*}(y) + G_t(y) + o_{P^*}(\zeta_{NT}(y)) \tag{H.6}
\end{aligned}$$

This shows

$$\hat{G}_t^*(y) - G_t(y) = \frac{1}{N} \sum_{i=1}^N \left[ \frac{1}{\sqrt{T}} d_{\psi,i}^{II*}(y) + d_{\gamma,i}^{II*}(y) \right] + o_{P^*}(\zeta_{NT}(y)).$$

Hence expansion (H.1) holds for  $G_t$ . The same proof also carries over to obtaining expansions for  $F_t$  and  $F_{t,I}$ , so we omit the proof for brevity. This leads to the desired coverage for following from Proposition H.1.  $\square$

#### H.4. Proof of Theorem 5.4 (iii): coverage of QE.

*Proof.* For a generic and  $\hat{F}^* \in \{\hat{F}_t^*, \hat{G}_t^*\}$ , and  $F \in \{F_t, G_t\}$ , we have

$$\hat{F}^*(\phi(\hat{F}^*, \tau)) = F(\phi(F, \tau)) = \tau.$$

Thus similar to the proof of Lemma G.1, for  $q_\tau := \phi(F, \tau)$ ,

$$\begin{aligned}
\phi(\hat{F}^*, \tau) - \phi(F, \tau) &= \frac{-1}{\dot{F}_t(q_\tau)} \Delta_F(q_\tau) + M_1(\tau) + M_2(\tau) \\
\Delta_F(y) &:= \hat{F}^*(y) - F(y) \\
M_1(\tau) &\leq C |\Delta_F(\phi(\hat{F}^*, \tau)) - \Delta_F(q_\tau)|^2 + C \Delta_F(q_\tau)^2 \\
M_2(\tau) &\leq C |\Delta_F(\phi(\hat{F}^*, \tau)) - \Delta_F(q_\tau)|. \tag{H.7}
\end{aligned}$$

Expansion (H.6) can be proved very similarly for  $\widehat{F}_t^*$ . Hence in general,

$$\Delta_F(y) = \frac{1}{N} \sum_i \frac{1}{\sqrt{T}} d_{\psi,i}^*(y) + \frac{1}{N} \sum_i d_{\gamma,i}^*(y) + o_{P^*}(\zeta_{NT}(y)). \quad (\text{H.8})$$

By Lemma H.3,  $\frac{1}{\sqrt{N}} \sum_i d_{\psi,i}^*(y)$ , and  $\text{Var}_t(d_{\gamma,i}(y))^{-1/2} \frac{1}{\sqrt{N}} \sum_i d_{\gamma,i}^*(y)$  are asymptotically stochastically equicontinuous. Then  $M_1 + M_2 = o_{P^*}(\zeta_{NT}(y))$ . Combine (H.8) and (H.7),

$$\phi(\widehat{F}^*, \tau) - \phi(F, \tau) = \frac{-1}{\dot{F}_t(q_\tau)} \left[ \frac{1}{N} \sum_i \frac{1}{\sqrt{T}} d_{\psi,i}^*(q_\tau) + \frac{1}{N} \sum_i d_{\gamma,i}^*(q_\tau) \right] + o_{P^*}(\zeta_{NT}(q_\tau)).$$

Thus

$$\widehat{\text{QE}}_t^*(\tau) - \text{QE}_t(\tau) = \frac{1}{N} \sum_{i=1}^N \left[ \frac{1}{\sqrt{T}} p_{\psi,i}^{II*}(\tau) + p_{\gamma,i}^{II*}(\tau) \right] + o_{P^*} \left( \frac{1}{\sqrt{NT}} + \text{Var}_t(p_{\gamma,i}^{II}(\tau)) \right),$$

where  $p^{II*}$  is SRS with replacement from  $p^{II}$ ; the latter is defined in (G.1). Hence expansion (H.1) holds for  $\widehat{\text{QE}}_t^*(\tau) - \text{QE}_t(\tau)$ . This leads to the desired coverage result, following from Proposition H.1. □

**Lemma H.3.**  $\frac{1}{\sqrt{N}} \sum_i d_{\psi,i}^*(y)$ , and  $\text{Var}_t(d_{\gamma,i}(y))^{-1/2} \frac{1}{\sqrt{N}} \sum_i d_{\gamma,i}^*(y)$  are asymptotically stochastically equicontinuous.

*Proof.* The proof is the mimick of that of Lemma G.2 in the bootstrap world. As it is almost the same, we omit the proof for brevity. □

## APPENDIX I. PROOFS FOR THE STATIONARY DISTRIBUTION

### I.1. The asymptotic distribution.

**Proposition I.1.** *We have*

$$\frac{\widehat{F}_\infty(\cdot) - F_\infty(\cdot)}{s_{NT}(\cdot)} \Rightarrow \mathbb{G}(\cdot)$$

where  $\mathbb{G}(\cdot)$  is a centered Gaussian process with covariance kernel

$$H(y_k, y_l) = \lim_T \frac{\sigma_T^2(y_k, y_l)}{\sigma_T(y_k) \sigma_T(y_l)}.$$

*Proof.* For notational simplicity, we write  $d_{\psi,i} = d_{\psi,i}^\infty$  and  $d_{\gamma,i} = d_{\gamma,i}^\infty$ . Lemma I.1 shows uniformly in  $y$ ,  $\zeta_{NT} = \frac{1}{\sqrt{NT}} + \bar{V}_\gamma(y)$ ,

$$\hat{F}_\infty(y) - F_\infty(y) = \frac{1}{N} \sum_{i=1}^N \left[ \frac{1}{\sqrt{T}} d_{\psi,i}(y) + d_{\gamma,i}(y) \right] + o_P(\zeta_{NT}(y)).$$

We now verify the three conditions in Assumption E.1.

*Assumption E.1 (i).* This follows from  $\mathbb{E}[\psi_{it}(y_k) | \gamma_i(y_l), \mathbf{w}_i, \beta_i(y_l), D_{it}] = 0$ .

*Assumption E.1 (ii).*

$$\begin{aligned} \mathbb{E} \sup_y |d_{\psi,i}(y)|^{2+a} &\leq C \mathbb{E} \sup_y \left\| \frac{1}{\sqrt{T}} \sum_{t=1}^T \partial_\beta f_i(\beta_i, y)' \mathbf{Z}_{it} \right\|^{2+a} \leq C \\ \mathbb{E} \sup_y \left| \frac{d_{\gamma,i}(y)^2}{\bar{V}_\gamma(y)} \right|^a &\leq C \mathbb{E} \sup_y [\mathbb{Z}_t(f(\beta_i, y))]^{2a} < C. \end{aligned}$$

*Assumption E.1 (iii).* For any  $\delta \in (0, 1)$ , and  $\rho(y_1, y_2) = \bar{C}^{1/4} |y_1 - y_2|^{1/4}$

$$\begin{aligned} &\mathbb{E} \sup_{\rho(y_1, y_2) < \delta} |d_{\psi,i}(y_1) - d_{\psi,i}(y_2)|^2 \\ &\leq \mathbb{E} \sup_{\rho(y_1, y_2) < \delta} \|\partial_\beta f_i(\beta_i, y_1)' - \partial_\beta f_i(\beta_i, y_2)'\|^2 \left\| \frac{1}{\sqrt{T}} \sum_{t=1}^T \mathbf{Z}_{it} \right\|^2 \\ &\leq C \left( \mathbb{E} \sup_{|y_1 - y_2| \leq \bar{C} \delta^4} \|\partial_\beta f_i(\beta_i, y_1)' - \partial_\beta f_i(\beta_i, y_2)'\|^4 \right)^{1/2} \leq C \bar{C} \delta^4 \leq \delta^2. \end{aligned}$$

Let  $V = \text{Var}(\frac{1}{\sqrt{T}} \sum_{t=1}^T \mathbf{Z}_{it} | \beta_i)$  and  $r(y) = \partial_\beta f_i(\beta_i, y)$ . Then  $\bar{V}_\psi(y) = \mathbb{E} r(y)' V r(y)$ . Hence

$$\begin{aligned} &\sup_{\rho(y_1, y_2) < \delta} |\bar{V}_\psi(y_1) - \bar{V}_\psi(y_2)|^2 \\ &\leq \sup_{\rho(y_1, y_2) < \delta} |\mathbb{E}(r(y_1) - r(y_2))' V r(y_1)|^2 + |\mathbb{E}(r(y_1) - r(y_2))' V r(y_2)|^2 \\ &\leq C \sup_{|y_1 - y_2| < \bar{C} \delta^4} \mathbb{E} \|r(y_1) - r(y_2)\|^2 \sup_y \mathbb{E} \|r(y)\|^2 \leq C \sup_{|y_1 - y_2| < \bar{C} \delta^4} \mathbb{E} \|r(y_1) - r(y_2)\|^2 \\ &\leq C \bar{C} \delta^8 \leq \delta^2. \end{aligned}$$

Also, it is our assumption that

$$\begin{aligned} &\mathbb{E} \sup_{\rho(y_1, y_2) < \delta} \frac{|f_i(\beta_i, y_1) - \mathbb{E} f_i(\beta_i, y_1) - (f_i(\beta_i, y_2) - \mathbb{E} f_i(\beta_i, y_2))|^2}{\sqrt{\text{Var}(f_i(\beta_i, y_1)) \text{Var}(f_i(\beta_i, y_2))}} \leq \delta^2 \\ &\sup_{\rho(y_1, y_2) < \delta} \frac{|\text{Var}(f_i(\beta_i, y_1)) - \text{Var}(f_i(\beta_i, y_2))|^2}{\text{Var}(f_i(\beta_i, y_1)) \text{Var}(f_i(\beta_i, y_2))} \leq \delta^2. \end{aligned}$$

Hence Assumption E.1 is verified. We then have the weak convergence, following from Proposition E.1.  $\square$

**Lemma I.1.** *Suppose Assumption F.1 holds. Uniformly in  $y$ ,*

$$\begin{aligned}\widehat{F}_\infty(y) - F_\infty(y) &= -\frac{1}{NT} \sum_{it} \partial_\beta f_i(\beta_i, y)' \mathbf{Z}_{it} \\ &\quad + \frac{1}{N} \sum_i [f_i(\beta_i, y) - \mathbb{E}f_i(\beta_i, y)] + o_P\left(\frac{1}{\sqrt{NT}}\right).\end{aligned}\quad (\text{I.1})$$

*Proof.* By Lemma D.2,

$$\widehat{\beta}_i - \beta_i = -\frac{1}{T} \sum_t \mathbf{Z}_{it} + \mathbf{R}_{i,4} + \mathbf{R}_{i,5} + \widetilde{\Delta}_i$$

where  $\sup_y \frac{1}{N} \sum_i \|\widetilde{\Delta}_i\|^2 = O_P(L^2 T^{-3})$  and  $\mathbf{R}_{i,d}$  is the vectorization of  $(R_{i,d}(y) : y = y_i^1, \dots, y_i^K)$ . Hence

$$\begin{aligned}& \frac{1}{N} \sum_{i=1}^N f_i(\widehat{\beta}_i, y) - F_\infty(y) \\ &= \frac{1}{N} \sum_i \dot{f}_i(y)' (\widehat{\beta}_i - \beta_i) + \frac{1}{2N} \sum_i \text{tr} \left[ \ddot{f}_{i,\beta}(y) (\widehat{\beta}_i - \beta_i) (\widehat{\beta}_i - \beta_i)' \right] \\ &\quad + \frac{1}{N} \sum_i f_i(\beta_i, y) - \mathbb{E}f_i(\beta_i, y) + R_1 \\ &= -\frac{1}{NT} \sum_{it} \dot{f}_i(y)' \mathbf{Z}_{it} + \frac{1}{2NT} \sum_i \text{tr} \left[ \ddot{f}_{i,\beta}(y) \mathbb{E}v_i \right] \\ &\quad + \frac{1}{N} \sum_i [f_i(\beta_i, y) - \mathbb{E}f_i(\beta_i, y)] + \sum_{d=1}^4 H_d\end{aligned}$$

where for some  $a_i$ ,

$$\begin{aligned}H_1 &:= \frac{1}{2NT} \sum_i \text{tr} \left[ \ddot{f}_{i,\beta}(y) (v_i - \mathbb{E}v_i) \right] \\ H_2 &:= \frac{1}{N} \sum_i \dot{f}_i(y)' (\mathbf{R}_{i,4} + \mathbf{R}_{i,5}) \\ H_3 &:= \frac{1}{N} \sum_i \dot{f}_i(y)' \widetilde{\Delta}_i - \frac{1}{2N} \sum_i \text{tr} \left[ \ddot{f}_{i,\beta}(y) \frac{1}{T} \sum_t \mathbf{Z}_{it} (\mathbf{R}_{i,4} + \mathbf{R}_{i,5})' \right] \\ &\quad - \frac{1}{2N} \sum_i \text{tr} \left[ \ddot{f}_{i,\beta}(y) \frac{1}{T} \sum_t \mathbf{Z}_{it} \widetilde{\Delta}_i' \right] \\ &\quad + \frac{1}{2N} \sum_i \text{tr} \left[ \ddot{f}_{i,\beta}(y) (\mathbf{R}_{i,4} + \mathbf{R}_{i,5}) (\widehat{\beta}_i - \beta_i)' \right] + \frac{1}{2N} \sum_i \text{tr} \left[ \ddot{f}_{i,\beta}(y) \widetilde{\Delta}_i (\widehat{\beta}_i - \beta_i)' \right]\end{aligned}$$

$$\begin{aligned}
H_4 &= \frac{1}{6N} \sum_i \partial_{\beta}^3 f_i(a_i, y, D_{it}) (\hat{\beta}_i - \beta_i) \otimes (\hat{\beta}_i - \beta_i) \otimes (\hat{\beta}_i - \beta_i) \\
v_i &:= \frac{1}{\sqrt{T}} \sum_t \mathbf{Z}_{it} \frac{1}{\sqrt{T}} \sum_s \mathbf{Z}'_{is} \quad \dot{f}(y) = \partial_{\beta} f_i(\beta, y), \quad \ddot{f}(y) = \partial_{\beta}^2 f_i(\beta, y)
\end{aligned}$$

We proceed as following steps. Step 1, show  $\sum_{d=1}^4 H_d$  is negligible. Step 2, estimate the bias  $\mathbb{E}v_i$  and compute the debiased estimator, and show that the bias estimation is negligible.

**step 1.** Write  $F_i(y) = \frac{1}{2\sqrt{N}} \text{tr} \left[ \ddot{f}_{i,\beta}(y)(v_i - \mathbb{E}v_i) \right]$ . Then  $H_1 = \frac{1}{T\sqrt{N}} \sum_i F_i(y)$ . We now show  $\sum_i F_i(y) = O_P(1)$  uniformly in  $y$  by showing it is asymptotically tight. For any  $\eta > 0$ , and  $a > 0$ ,

$$\begin{aligned}
& \sum_i \mathbb{E} \sup_y |F_i(y)| 1\{\sup_y |F_i(y)| > \eta\} \leq \frac{1}{\eta} \sum_i \mathbb{E} \sup_y |F_i(y)|^2 1\{\sup_y |F_i(y)| > \eta\} \\
& \leq \frac{1}{4N^{a/2}\eta^{1+a}} \frac{1}{N} \sum_i \mathbb{E} \sup_y \left[ \ddot{f}_{i,\beta}(y)(v_i - \mathbb{E}v_i) \right]^{2+a} \\
& \leq \frac{C}{N^{a/2}\eta^{1+a}} \frac{1}{N} \sum_i [\mathbb{E} [v_i - \mathbb{E}v_i]^4]^{(2+a)/4} = o(1)
\end{aligned}$$

provided that  $\mathbb{E}v_i^4$  and  $\max_i \mathbb{E} \sup_y \|\ddot{f}(y)\|^{4/3} < C$ .

Next, for every  $y_1, y_2 \in \mathcal{Y}$ ,

$$\begin{aligned}
& \sum_i \mathbb{E} |F_i(y_1) - F_i(y_2)|^2 \leq \frac{C}{N} \sum_i (\mathbb{E} \|\ddot{f}_{i,\beta}(y_1) - \ddot{f}_{i,\beta}(y_2)\|^4)^{1/2} (\mathbb{E} \|v_i\|^4)^{1/2} \\
& \leq C |y_1 - y_2|^2.
\end{aligned}$$

For every  $\delta > 0$ , and  $\rho(y_1, y_2) = \bar{C}|y_1 - y_2|$ , for sufficiently large  $\bar{C}$ ,

$$\begin{aligned}
& \sup_{\eta > 0} \sum_i \eta^2 P \left( \sup_{\rho(y_1, y_2) < \delta} |F_i(y_1) - F_i(y_2)| > \eta \right) \leq \sum_i \mathbb{E} \left( \sup_{\rho(y_1, y_2) < \delta} |F_i(y_1) - F_i(y_2)|^2 \right) \\
& \leq \frac{C}{N} \sum_i (\mathbb{E} \sup_{\rho(y_1, y_2) < \delta} |\ddot{f}_{i,\beta}(y_1) - \ddot{f}_{i,\beta}(y_2)|^4)^{1/2} (\mathbb{E} \|v_i\|^4)^{1/2} \leq \delta^2.
\end{aligned}$$

Hence all conditions of Theorem 2.11.11 in van der Vaart and Wellner (1996) are verified. Thus  $\sum_i F_i(y) = O_P(1)$  uniformly in  $y$ . This implies  $\sup_y H_1 = O_P(\frac{1}{T\sqrt{N}})$ . In addition, it follows from the same argument that  $\sup_y H_2 = O_P(\frac{1}{T\sqrt{N}})$ . Next, by Cauchy-Schwarz inequality, uniformly in  $y$ ,

$$H_3^2 \leq O_P(1) \frac{1}{N} \sum_i \|\tilde{\Delta}_i\|^2 + O_P(1) \left( \frac{1}{N} \sum_i \left[ \frac{1}{T} \sum_t \mathbf{Z}_{it} \right]^4 \right)^{1/2} \frac{1}{N} \sum_i [\|\mathbf{R}_{i,4} + \mathbf{R}_{i,5}\|^2 + \|\tilde{\Delta}_i\|^2]$$

$$+O_P(1) \left( \frac{1}{N} \sum_i [\hat{\beta}_i - \beta_i]^4 \right)^{1/2} \frac{1}{N} \sum_i [\|\mathbf{R}_{i,4} + \mathbf{R}_{i,5}\|^2 + \|\tilde{\Delta}_i\|^2] = O_P\left(\frac{1}{T^3} + \frac{L^2}{T^4}\right).$$

Together, provided that  $N = o(T^2)$  and  $NL^2 = o(T^3)$ ,

$$\begin{aligned} \sup_y |H_1 + H_2 + H_3| &= O_P\left(\frac{1}{T\sqrt{N}} + \frac{1}{T^{3/2}} + \frac{L}{T^2}\right) = o_P\left(\frac{1}{\sqrt{NT}}\right) \\ \sup_y H_4 &\leq \sup_y \frac{C}{N} \sum_i \|\hat{\beta}_i - \beta_i\|^3 = O_P\left(\frac{1}{T^{3/2}}\right) = o_P\left(\frac{1}{\sqrt{NT}}\right). \end{aligned}$$

**Step 2.** Bias correction. Because  $\psi_{is}(y)$  is a martingale difference,

$$\mathbb{E}v_i = \frac{1}{T} \sum_t \mathbb{E}\mathbf{Z}_{it}\mathbf{Z}'_{it}.$$

The effect of bias correction is: uniformly in  $y$ ,

$$\begin{aligned} & \frac{1}{2NT} \sum_i \text{tr} \left[ \partial_{\beta}^2 f_i(\hat{\beta}_i, y) \frac{1}{T} \sum_t \hat{\mathbf{Z}}_{it} \hat{\mathbf{Z}}'_{it} \right] - \frac{1}{2NT} \sum_i \text{tr} [\partial_{\beta}^2 f_i(\beta_i, y) \mathbb{E}v_i(y)] \\ & \leq \frac{1}{2NT} \sum_i \text{tr} [\partial_{\beta}^2 f_i(\hat{\beta}_i, y) - \partial_{\beta}^2 f_i(\beta_i, y)] \frac{1}{T} \sum_t \hat{\mathbf{Z}}_{it} \hat{\mathbf{Z}}'_{it} \\ & \quad + \frac{1}{2NT} \sum_i \text{tr} \partial_{\beta}^2 f_i(\beta_i, y) \left[ \frac{1}{T} \sum_t \hat{\mathbf{Z}}_{it} \hat{\mathbf{Z}}'_{it} - \mathbb{E}v_i \right] \\ & \leq \frac{1}{T} \left( \frac{1}{N} \sum_i \|\hat{\beta}_i - \beta_i\|^4 \right)^{1/4} O_P(1) + \frac{C}{T} \left( \frac{1}{N} \sum_i \left\| \frac{1}{T} \sum_t \hat{\mathbf{Z}}_{it} \hat{\mathbf{Z}}'_{it} - \mathbb{E}v_i \right\|^2 \right)^{1/2} \\ & = O_P\left(\frac{1}{T^{3/2}}\right) = o_P\left(\frac{1}{\sqrt{NT}}\right). \end{aligned}$$

□

**Proposition I.2.** *We have*

$$\frac{\hat{G}_{\infty}(\cdot) - G_{\infty}(\cdot)}{s_{NT}(\cdot)} \Rightarrow \mathbb{G}(\cdot)$$

where  $\mathbb{G}(\cdot)$  is a centered Gaussian process with covariance kernel

$$H(y_k, y_l) = \lim_T \frac{\sigma_T^2(y_k, y_l)}{\sigma_T(y_k)\sigma_T(y_l)}.$$

*Proof.* For notational simplicity, we write  $d_{\psi,i} = d_{\psi,i}^{\infty,II}$  and  $d_{\gamma,i} = d_{\gamma,i}^{\infty,II}$ . Write  $\partial_{\beta} f_i(y) := \partial_{\beta} f_i(\beta_i, \theta_i, y)$ . Then uniformly in  $i \leq N$ , (E.7) implies

$$\hat{\theta}_i - \theta_i = \frac{1}{NT} \sum_{jt} \mathbf{Z}_{jt,i} \mathbf{w}'_j S_{wz} + \frac{1}{N} \sum_j \gamma_{j,i} \mathbf{w}'_j S_{wz} + o_P(\zeta_{NT}(y)).$$

By the Taylor expansion up to the second order,

$$\begin{aligned}
& \frac{1}{N} \sum_i f_i(\hat{\beta}_i, \hat{\theta}_i, y) - \frac{1}{N} \sum_i f(\beta_i, \theta_i, y) = D_0 + \dots + D_3 + R_1 \\
D_0 &:= \frac{1}{N} \sum_i \partial_{\beta} f_i(y)' (\hat{\beta}_i - \beta_i) = -\frac{1}{NT} \sum_{it} \partial_{\beta} f_i(y)' \mathbf{Z}_{it} + o_P(\zeta_{NT}(y)) \\
D_1 &:= \frac{1}{2N} \sum_i \text{tr} \left[ \ddot{f}_{i,\beta}(\hat{\beta}_i - \beta_i)(\hat{\beta}_i - \beta_i)' \right] \\
&= \frac{1}{2NT} \sum_i \text{tr} \left[ \partial_{\beta}^2 f_i(\hat{\beta}_i, \hat{\theta}_i, y) \frac{1}{T} \sum_i \hat{\mathbf{Z}}_{it} \hat{\mathbf{Z}}_{it}' \right] + o_P(\zeta_{NT}(y)) \\
D_2 &:= \frac{1}{N} \sum_i \partial_{\theta} f_i(\beta_i, \theta_i, y)' (\hat{\theta}_i - \theta_i) \\
&= \frac{1}{N^2 T} \sum_{ijt} \partial_{\theta} f_i(\beta_i, \theta_i, y)' \mathbf{Z}_{jt,i} \mathbf{w}'_j S_{wz} + \frac{1}{N^2} \sum_{ij} \partial_{\theta} f_i(\beta_i, \theta_i, y)' \gamma_{j,i} \mathbf{w}'_j S_{wz} + o_P(\zeta_{NT}(y)) \\
D_3 &:= \frac{1}{N} \sum_i (\hat{\beta}_i(y) - \beta_i(y))' \ddot{f}_{i,\beta\theta}(\hat{\theta}_i - \theta_i) + \frac{1}{2N} \sum_i (\hat{\theta}_i - \theta_i)' \ddot{f}_{i,\theta}(\hat{\theta}_i - \theta_i) = o_P(\zeta_{NT}(y)).
\end{aligned}$$

This implies

$$\hat{G}_{\infty}(y) - G_{\infty}(y) = \frac{1}{N} \sum_j \left[ \frac{1}{\sqrt{T}} d_{\psi,j}(y) + d_{\gamma,j}(y) \right] + o_P(\zeta_{NT}(y)). \quad (\text{I.2})$$

We now verify the three conditions in Assumption E.1.

*Assumption E.1 (i)(ii)* hold by the assumption.

*Assumption E.1 (iii).* Let  $A := \frac{1}{N} \sum_i \mathbb{E} \|\mathbf{w}'_j S_{wz}\|^4 \|\frac{1}{\sqrt{T}} \sum_t \mathbf{Z}_{jt,i}\|^4$ . For any  $\delta \in (0, 1)$ , and  $\rho(y_1, y_2) = \bar{C}^{1/4} |y_1 - y_2|^{1/4}$

$$\begin{aligned}
& \mathbb{E} \sup_{\rho(y_1, y_2) < \delta} |d_{\psi,i}(y_1) - d_{\psi,i}(y_2)|^2 \\
& \leq \mathbb{E} \sup_{\rho(y_1, y_2) < \delta} \|\partial_{\beta} f_i(\beta_i, \theta_i, y_1)' - \partial_{\beta} f_i(\beta_i, \theta_i, y_2)'\|^2 \left\| \frac{1}{\sqrt{T}} \sum_{t=1}^T \mathbf{Z}_{it} \right\|^2 \\
& \quad + C \mathbb{E} \sup_{\rho(y_1, y_2) < \delta} \left\| \frac{1}{\sqrt{T}} \sum_t H_{it}(y_1) - H_{it}(y_2) \right\|^2 \|\mathbf{w}'_j S_{wz}\|^2 \\
& \leq C \bar{C} \delta^4 + C \left[ \mathbb{E} \sup_{\rho(y_1, y_2) < \delta} \|\partial_{\theta} f_i(y_1) - \partial_{\theta} f_i(y_2)\|^4 \right]^{1/2} \sqrt{A} \leq C \bar{C} \delta^4 \leq \delta^2.
\end{aligned}$$

Next,  $d_{\psi,j}(y)$  can be expressed in a more compact form. Let

$$\partial_{\theta} \mathbf{f}(y)' = (\partial_{\theta} f_1(y)', \dots, \partial_{\theta} f_N(y)'), \quad \bar{\mathbf{Z}}_{jt} = \text{vec}(\mathbf{Z}_{jt,1}, \dots, \mathbf{Z}_{jt,N}), \quad \bar{\mathbf{e}}_j = (\mathbf{0}, \dots, \mathbf{0}, \underbrace{\mathbf{I}}_{j \text{ th block}}, \mathbf{0} \dots).$$

Then

$$d_{\psi,j}(y) = \left[ \frac{1}{N} \mathbf{w}'_j S_{wz} \partial_{\theta} \mathbf{f}(y)' - \partial_{\beta} f_j(y)' \bar{\mathbf{e}}'_j \right] \frac{1}{\sqrt{T}} \sum_t \bar{\mathbf{Z}}_{jt}$$

Let  $r_1(y)' = \frac{1}{N} \mathbf{w}'_j S_{wz} \partial_{\theta} \mathbf{f}(y)'$ ,  $r_2(y)' = -\partial_{\beta} f_j(y)' \bar{\mathbf{e}}'_j$ ,  $V = \text{Var}(\frac{1}{\sqrt{T}} \sum_t \bar{\mathbf{Z}}_{jt} | \boldsymbol{\beta}, \mathbf{w}_j)$ . Also let  $V_{k_1, k_2}$  denote the  $(k_1, k_2)$  th block of  $V$ , which is a matrix collecting pairwise covariances between elements of  $\mathbf{Z}_{jt, k_1}$  and  $\mathbf{Z}_{jt, k_2}$ . Then we have  $\bar{V}_{\psi}(y) = \mathbb{E}(r_1(y) + r_2(y))' V (r_1(y) + r_2(y))$ . Hence

$$\begin{aligned} & \sup_{\rho(y_1, y_2) < \delta} |\bar{V}_{\psi}(y_1) - \bar{V}_{\psi}(y_2)|^2 \\ & \leq \max_{d=1,2} \sup_{\rho(y_1, y_2) < \delta} |\mathbb{E}(r_1(y_1) - r_1(y_2))' V r_1(y_d)|^2 + \max_{d=1,2} \sup_{\rho(y_1, y_2) < \delta} |\mathbb{E}(r_1(y_1) - r_1(y_2))' V r_2(y_d)|^2 \\ & \quad + \max_{d=1,2} \sup_{\rho(y_1, y_2) < \delta} |\mathbb{E}(r_2(y_1) - r_2(y_2))' V r_1(y_d)|^2 + \max_{d=1,2} \sup_{\rho(y_1, y_2) < \delta} |\mathbb{E}(r_2(y_1) - r_2(y_2))' V r_2(y_d)|^2 \\ & \leq a_1 + \dots + a_4 \\ a_1 & \leq \max_{d=1,2} \sup_{\rho(y_1, y_2) < \delta} \left[ \frac{1}{N^2} \sum_{k_1, k_2 \leq N} \mathbb{E} \|\partial_{\theta} f_{k_1}(y_1) - \partial_{\theta} f_{k_1}(y_2)\| \|V_{k_1, k_2}\| \|\partial_{\theta} f_{k_2}(y_d)\| \|\mathbf{w}_j\|^2 \|S_{wz}\|^2 \right]^2 \\ & \leq C \max_{d=1,2} \sup_{\rho(y_1, y_2) < \delta} \max_{k_1, k_2 \leq N} [\mathbb{E} \|\partial_{\theta} f_{k_1}(y_1) - \partial_{\theta} f_{k_1}(y_2)\|^4]^{1/2} [\mathbb{E} \|\partial_{\theta} f_{k_2}(y_d)\|^4]^{1/2} \mathbb{E} \|\mathbf{w}_j\|^4 \\ & \leq \delta^2 \\ a_2 & \leq \max_{d=1,2} \sup_{\rho(y_1, y_2) < \delta} \left[ \frac{1}{N} \sum_{k_1=1}^N \mathbb{E} \|\partial_{\theta} f_{k_1}(y_1) - \partial_{\theta} f_{k_1}(y_2)\| \|V_{k_1, j}\| \|\mathbf{w}_j\| \|S_{wz}\| \|\partial_{\beta} f_j(y_d)\| \right]^2 \leq \delta^2 \\ a_3 & \leq \max_{d=1,2} \sup_{\rho(y_1, y_2) < \delta} \left[ \frac{1}{N} \sum_{k_2=N}^N \mathbb{E} \|\partial_{\beta} f_j(y_1) - \partial_{\beta} f_j(y_2)\| \|V_{j, k_2}\| \|\partial_{\theta} f_{k_2}(y_d)\| \|\mathbf{w}_j\| \|S_{wz}\| \right]^2 \leq \delta^2 \\ a_4 & \leq \max_{d=1,2} \sup_{\rho(y_1, y_2) < \delta} [\mathbb{E} \|\partial_{\beta} f_j(y_1) - \partial_{\beta} f_j(y_2)\| \|V_{j, j}\| \|\partial_{\beta} f_j(y_d)\|]^2 \leq \delta^2. \end{aligned}$$

Also, it is our assumption that

$$\begin{aligned} & \mathbb{E} \sup_{\rho(y_1, y_2) < \delta} \frac{|f_i(\boldsymbol{\beta}_i, y_1) - \mathbb{E} f_i(\boldsymbol{\beta}_i, y_1) - (f_i(\boldsymbol{\beta}_i, y_2) - \mathbb{E} f_i(\boldsymbol{\beta}_i, y_2))|^2}{\sqrt{\bar{V}_{\gamma}(y_1) \bar{V}_{\gamma}(y_2)}} \leq \delta^2 \\ & \mathbb{E} \sup_{\rho(y_1, y_2) < \delta} \frac{\|\partial_{\theta} f_i(\boldsymbol{\beta}_i, \boldsymbol{\theta}_i, y_1) - \partial_{\theta} f_i(\boldsymbol{\beta}_i, \boldsymbol{\theta}_i, y_2)\|^2 \|\boldsymbol{\gamma}_{j,i} \mathbf{w}'_j\|^2}{\sqrt{\bar{V}_{\gamma}(y_1) \bar{V}_{\gamma}(y_2)}} \leq \delta^2 \\ & \sup_{\rho(y_1, y_2) < \delta} \frac{|\bar{V}_{\gamma}(y_1) - \bar{V}_{\gamma}(y_2)|^2}{\bar{V}_{\gamma}(y_1) \bar{V}_{\gamma}(y_2)} \leq \delta^2 \end{aligned}$$

Hence Assumption E.1 is verified. Then based on (I.2), we have the weak convergence, following from Proposition E.1.

□

**Proposition I.3.** *For all  $F \in \{F_\infty, G_\infty\}$ ,  $F$  is continuously differentiable, whose density  $\dot{F}$  satisfies: there are  $C, c > 0$  so that  $\inf_\tau \inf_{|y-\phi(F,\tau)|<C} \dot{F}(y) > c$ .*

Then

$$\frac{\widehat{\mathbb{Q}\mathbb{E}}_\infty(\cdot) - \mathbb{Q}\mathbb{E}_\infty(\cdot)}{J_{NT}(\cdot)} \Rightarrow \mathbb{G}_{\mathbb{Q}\mathbb{E},\infty}(\cdot),$$

and

$$\frac{\widehat{\mathbb{Q}\mathbb{E}}_{\infty,II}^*(\cdot) - \widehat{\mathbb{Q}\mathbb{E}}_\infty(\cdot)}{J_{NT}(\cdot)} \Rightarrow \mathbb{G}_{\mathbb{Q}\mathbb{E},\infty}(\cdot),$$

*Proof.* Similar to the proof of Lemma G.1, for  $F \in \{F_\infty, G_\infty\}$  and  $\widehat{F} \in \{\widehat{F}_\infty, \widehat{G}_\infty\}$ ,

$$\phi(\widehat{F}, \tau) - \phi(F, \tau) = \frac{-1}{\dot{F}(q(\tau))} \frac{1}{N} \sum_i \left[ \frac{1}{\sqrt{T}} d_{\psi,i}(q(\tau)) + d_{\gamma,i}(q(\tau)) \right] + o_P(z(q(\tau))),$$

where  $q(\tau) = \phi(F, \tau)$ ,  $z(y) = (NT)^{-1/2} + N^{-1/2} \text{Var}_t(d_{\gamma,i}(y))^{1/2}$ . This implies

$$\widehat{\mathbb{Q}\mathbb{E}}_\infty(\tau) - \mathbb{Q}\mathbb{E}_\infty(\tau) = \frac{1}{N} \sum_{i=1}^N \left[ \frac{1}{\sqrt{T}} p_{\psi,i}^{\infty,II}(\tau) + p_{\gamma,i}^{\infty,II}(\tau) \right] + o_P\left(\frac{1}{\sqrt{NT}} + \text{Var}(p_{\gamma,i}^{\infty,II}(\tau))\right),$$

From here, establishing the weak convergence can be done via applying Proposition E.1, where all conditions in Assumption E.1 are straightforward to verify.

The bootstrap convergence for  $\widehat{\mathbb{Q}\mathbb{E}}_\infty^*(\tau) - \widehat{\mathbb{Q}\mathbb{E}}_\infty(\tau)$  follows from the same argument.  $\square$

## REFERENCES

- DHAENE, G. and JOCHMANS, K. (2015). Split-panel jackknife estimation of fixed-effect models. *The Review of Economic Studies* **82** 991–1030.
- OKUI, R. and YANAGI, T. (2019). Panel data analysis with heterogeneous dynamics. *Journal of Econometrics* **212** 451–475.
- RILSTONE, P., SRIVASTAVA, V. K. and ULLAH, A. (1996). The second-order bias and mean squared error of nonlinear estimators. *Journal of Econometrics* **75** 369–395.
- VAN DER VAART, A. and WELLNER, J. (1996). *Weak convergence and empirical processes*. The first edition ed. Springer.

DEPARTMENT OF ECONOMICS, BOSTON UNIVERSITY, BOSTON, MA  
*Email address:* `ivanf@bu.edu`

DEPARTMENT OF ECONOMICS, UNIVERSITY OF PENNSYLVANIA, PHILADELPHIA, PA  
*Email address:* `waynegao@upenn.edu`

DEPARTMENT OF ECONOMICS, RUTGERS UNIVERSITY, NEW BRUNSWICK, NJ 08901  
*Email address:* `yuan.liao@rutgers.edu`

DEPARTMENT OF ECONOMICS, GEORGETOWN UNIVERSITY,  
*Email address:* `fgv@georgetown.edu`
